# Supplementary material for: Knowledge Graphs for Multilingual Language Translation and Generation
Source: arXiv:2009.07715 source file (2020-09-16)
Supplement: Supplementary file 3 [file MAG_40.pdf]

# Entity Linking in 40 Languages using MAG

Diego Moussallem[1,2], Ricardo Usbeck[2][0000−0002−0191−7211], Michael Röder[2], and Axel-Cyrille Ngonga Ngomo[1,2]

[1] AKSW Research Group, University of Leipzig, Germany
[2] Data Science Department, Paderborn University, Germany
lastname@informatik.uni-leipzig.de

**Abstract.** A plethora of Entity Linking (EL) approaches has recently been developed. While many claim to be multilingual, the MAG (Multilingual AGDISTIS) approach has been shown recently to outperform the state of the art in multilingual EL on 7 languages. With this demo, we extend MAG to support EL in 40 different languages, including especially low-resources languages such as Ukrainian, Greek, Hungarian, Croatian, Portuguese, Japanese and Korean. Our demo relies on online web services which allow for an easy access to our entity linking approaches and can disambiguate against DBpedia and Wikidata. During the demo, we will show how to use MAG by means of POST requests as well as using its user-friendly web interface. All data used in the demo is available at `https://hobbitdata.informatik.uni-leipzig.de/agdistis/`

## 1 Introduction

A recent survey by IBM[3] suggests that more than 2.5 quintillion bytes of data are produced on the Web every day. Entity Linking (EL), also known as Named Entity Disambiguation (NED), is one of the most important Natural Language Processing (NLP) techniques for extracting knowledge automatically from this huge amount of data. The goal of an EL approach is as follows: Given a piece of text, a reference knowledge base $K$ and a set of entity mentions in that text, map each entity mention to the corresponding resource in $K$ [4]. A large number of challenges has to be addressed while performing a disambiguation. For instance, a given resource can be referred to using different labels due to phenomena such as synonymy, acronyms or typos. For example, `New York City`, `NY` and `Big Apple` are all labels for the same entity. Also, multiple entities can share the same name due to homonymy and ambiguity. For example, both the state and the city of Rio de Janeiro are called `Rio de Janeiro`.

Despite the complexity of the task, EL approaches have recently achieved increasingly better results by relying on trained machine learning models [6]. A portion of these approaches claim to be multilingual and most of them rely on models which are trained on English corpora with cross-lingual dictionaries. However, MAG (Multilingual AGDISTIS) [4] showed that the underlying models being trained on English corpora make them prone to failure when migrated to a different language. Additionally, these approaches hardly make their models or data available on more than three languages [6]. The new version of MAG (which is the quintessence of this demo) provides

[3] `https://tinyurl.com/ibm2017stats`

support for 40 different languages using sophisticated indices[4]. For the sake of server space, we deployed MAG-based web services for 9 languages and offer the other 31 languages for download. Additionally, we provide an English index using Wikidata to show the knowledge-base agnosticism of MAG. During the demo, we will show how to use the web services as well as MAG's user interface.

## 2 MAG Entity Linking System

MAG's EL process comprises two phases, namely an offline and an online phase. The sub-indices (which are generated during the offline phase) consist of surface forms, person names, rare references, acronyms and context information. During the online phase, the EL is carried out in two steps: 1) candidate generation and 2) disambiguation. The goal of the candidate generation step is to retrieve a tractable number of candidates for each mention. These candidates are later inserted into the disambiguation graph, which is used to determine the mapping between entities and mentions. MAG implements two graph-based algorithms to disambiguate entities, i.e., PageRank and HITS. Independently of the chosen graph algorithm, the highest candidate score among the set of candidates is chosen as correct disambiguation for a given mention [4].

## 3 Demonstration

Our demonstration will show the capabilities of MAG for different languages. We provide a graphical, web-based user interface (GUI). In addition, users can choose to use the REST interface or a Java snippet. For research purposes, MAG can be downloaded and deployed via Maven or Docker. Figure 1 illustrates an example of MAG working on Spanish. The online demo can be accessed via `http://http://agdistis.aksw.org/mag-demo` and its code can be downloaded from `https://github.com/dice-group/AGDISTIS_DEMO/tree/v2`.

We have set up a web service interface for each language version. Each of these interfaces understands two mandatory parameters: (1) `text` and (2) `type`.

1. `text` accepts an UTF-8 and URL encoded string with entities annotated with XML-tag `<entity>`. It is also capable of recognizing NIF [3] or txt files.
2. `type` accepts two different values. First, `'agdistis'` to disambiguate the mentions using the graph-based algorithms, but also `'candidates'` which list all possible entities for a given mention through the depth-candidate selection of MAG.

**Other parameters.** The user can also define more parameters to fine-tune the disambiguation. These parameters have to be set up within the properties file[5] or via environment variables while deploying it locally. Below, we describe all the parameters.

[4] The quality of indices is directly related to how much information is provided by Wikipedia and DBpedia

[5] `https://tinyurl.com/agdistis-properties`

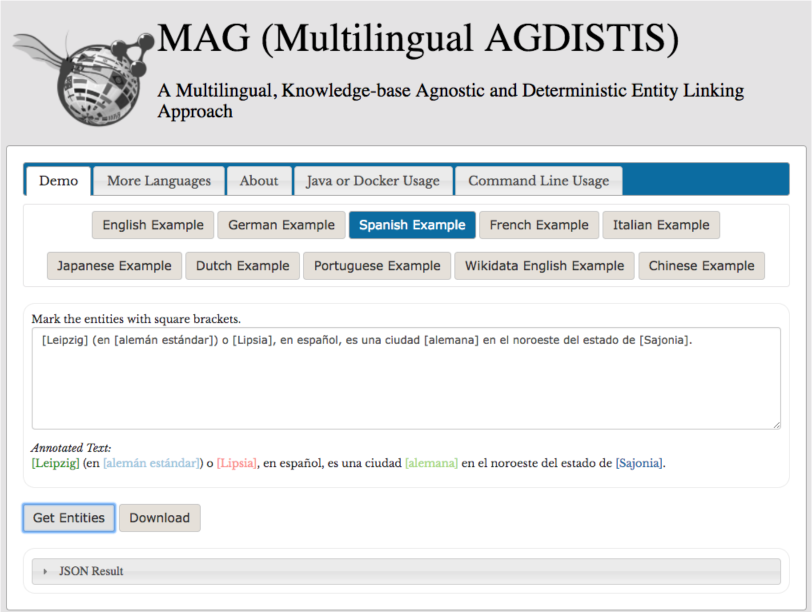


**Fig. 1.** A screenshot of MAG's web-based demo working on Spanish.

- **Popularity** - The user can set it as `popularity=false` or `popularity=true`. It allows MAG to use either the Page Rank or the frequency of a candidate to sort while candidate retrieval.
- **Graph-based algorithm** - The user can choose which graph-based algorithm to use for disambiguating among the candidates per mentions. The current implementation offers HITS and PageRank as algorithms, `algorithm=hits` or `algorithm =pagerank`.
- **Search by Context** - This boolean parameter provides a search of candidates using a context index [4].
- **Acronyms** - This parameter enables a search by acronyms. In this case, MAG uses an additional index to filter the acronyms by expanding their labels and assigns them a high probability. For example, PSG equals Paris Saint-Germain. The parameter is `acronym=false` or `acronym=true`.
- **Common Entities** - This boolean option supports finding common entities , in case, users desire to find more than ORGANIZATIONs, PLACEs and PERSONs as entity type.
- **Ngram Distance** - This integer parameter chooses the ngram distance between words, e.g., bigram, trigram and so on.
- **Depth** - This parameter numerically defines how deep the exploration of a semantic disambiguation graph must go.
- **Heuristic Expansion** - This boolean parameter defines whether a simple co-occurrence resolution is done or not. For instance, if Barack and Barack Obama are in the same text then Barack is expanded to Barack Obama.

**Knowledge-base Agnosticism.** Figure 2 shows a screen capture of our demo for disambiguating mentions using Wikidata. We also provide a web service to allow further investigation. In addition, MAG is used in a domain specific problem using a music Knowledge Base (KB) [5].

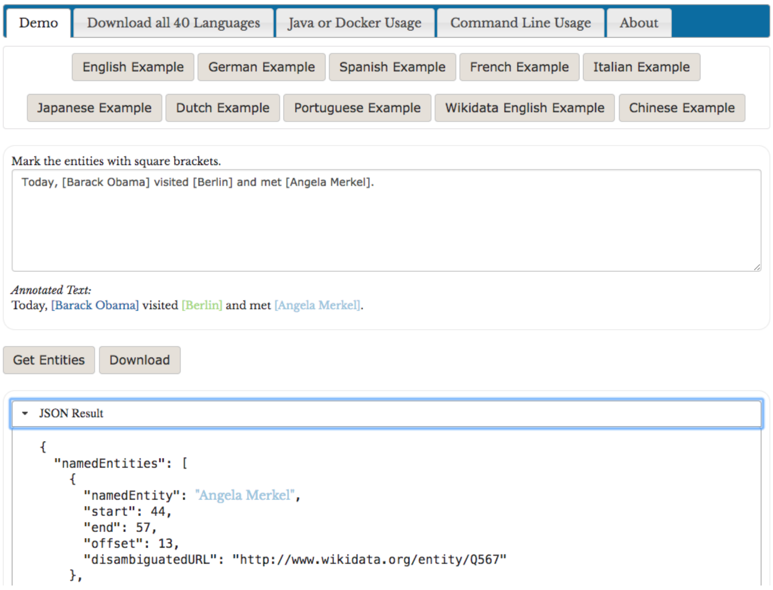


**Fig. 2.** MAG working on Wikidata as Knowledge base.

## 4 Evaluation of the user interface

We performed a system usability study (SUS)[6][7] to validate the design of our user interface. 15 users - with a good or no knowledge of Semantic Web, EL or knowledge extraction - selected randomly from all departments at Leipzig University answered our survey. We achieved a SUS-Score of 86.3. This score assigns the mark $S$ to the current interface of MAG and places it into the *category of the 10% interfaces*, meaning that users of the interface are likely to recommend it to a friend. Figure 3 shows the average voting per question and its standard deviation.

## 5 Summary

In this demo, we will present MAG, a KB-agnostic and deterministic approach for multilingual EL on 40 different languages contained in DBpedia. Currently, MAG is used

[6] `http://www.measuringu.com/sus.php`
[7] `https://goo.gl/forms/01kpxBf24pjbsWUV2`

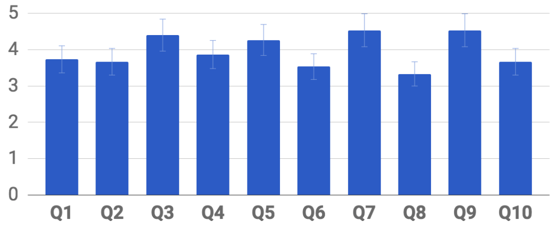


**Fig. 3.** Standard Usability Score results. The vertical bars show the standard deviation

in diverse projects[8] and has been used largely by the Semantic Web community. We also provide a demo/web-service using Wikidata for supporting an investigation of the graphs structures behind DBpedia and Wikidata pertaining to Information Extraction tasks [1, 2]. The indexes we provided will be used in future work to investigate the EL problem in low-resource languages. Our next step will hence be to to evaluate EL on all 40 languages presented in this demo.

**Acknowledgements** This work has been supported by the EuroStars projects DIESEL (no. 01QE1512C) and QAMEL (no. 01QE1549C) and supported by the Brazilian National Council for Scientific and Technological Development (CNPq) (no. 206971/2014-1). This work has also been supported by the German Federal Ministry of Transport and Digital Infrastructure (BMVI) in the projects LIMBO (no. 19F2029I) and OPAL (no. 19F2028A) as well as by the German Federal Ministry of Education and Research (BMBF) within 'KMU-innovativ: Forschung für die zivile Sicherheit' in particular 'Forschung für die zivile Sicherheit' and the project SOLIDE (no. 13N14456).

## References

1. M. Färber, B. Ell, C. Menne, and A. Rettinger. A comparative survey of dbpedia, freebase, opencyc, wikidata, and yago. *Semantic Web Journal*, 1:1–5, 2015.
2. J. Geiß, A. Spitz, and M. Gertz. Neckar: A named entity classifier for wikidata. In *International Conference of the German Society for Computational Linguistics and Language Technology*, pages 115–129. Springer, 2017.
3. S. Hellmann, J. Lehmann, S. Auer, and M. Brümmer. Integrating NLP using Linked Data. In *12th International Semantic Web Conference*, 2013.
4. D. Moussallem, R. Usbeck, M. Röeder, and A.-C. N. Ngomo. MAG: A Multilingual, Knowledge-base Agnostic and Deterministic Entity Linking Approach. In *Proceedings of the Knowledge Capture Conference*, page 9. ACM, 2017.
5. S. Oramas, A. Ferraro, A. Correya, and X. Serra. Mel: A music entity linking system. In *18th International Society for Music Information Retrieval Conference (ISMIR17)*, 2017.
6. M. Röder, R. Usbeck, and A.-C. N. Ngomo. GERBIL–Benchmarking Named Entity Recognition and Linking Consistently. *Semantic Web Journal*, 2018.

[8] For example, `http://diesel-project.eu/`, `https://qamel.eu/` or `https://www.limbo-project.org/`
