# Supplementary material for: Knowledge Graphs for Multilingual Language Translation and Generation
Source: arXiv:2009.07715 source file (2020-09-16)
Supplement: Supplementary file 5 [file KG-NMT.pdf]

# Utilizing Knowledge Graphs for Neural Machine Translation Augmentation

Diego Moussallem

Data Science Research Group, Paderborn University  
Germany  
diego.moussallem@upb.de

Paul Buitelaar

Insight Centre for Data Analytics, Data Science Institute  
National University of Ireland Galway  
Ireland  
paul.buitelaar@insight-centre.org

Axel-Cyrille Ngonga Ngomo

Data Science Group, Paderborn University  
Germany  
axel.ngonga@upb.de

Mihael Arcan

Insight Centre for Data Analytics, Data Science Institute  
National University of Ireland Galway  
Ireland  
mihael.arcan@insight-centre.org

## ABSTRACT

While neural networks have led to substantial progress in machine translation, their success depends heavily on large amounts of training data. However, parallel training corpora are not always readily available. Moreover, out-of-vocabulary words—mostly entities and terminological expressions—pose a difficult challenge to Neural Machine Translation systems. Recent efforts have tried to alleviate the data sparsity problem by augmenting the training data using different strategies, such as external knowledge injection. In this paper, we hypothesize that knowledge graphs enhance the semantic feature extraction of neural models, thus optimizing the translation of entities and terminological expressions in texts and consequently leading to better translation quality. We investigate two different strategies for incorporating knowledge graphs into neural models without modifying the neural network architectures. Additionally, we examine the effectiveness of our augmented models on domain-specific texts and ontologies. Our knowledge-graph-augmented neural translation model, dubbed *KG-NMT*, achieves significant and consistent improvements of +3 BLEU, METEOR and CHRF3 on average on the *newstest* datasets between 2015 and 2018 for the WMT English-German translation task.

## CCS CONCEPTS

• **Information systems** → **Information extraction**; • **Computing methodologies** → **Natural language processing**.

## KEYWORDS

Neural Machine Translation, Knowledge Graphs, NLP, Linked Data

### ACM Reference Format:

Diego Moussallem, Axel-Cyrille Ngonga Ngomo, Paul Buitelaar, and Mihael Arcan. 2019. Utilizing Knowledge Graphs for Neural Machine Translation

Permission to make digital or hard copies of all or part of this work for personal or classroom use is granted without fee provided that copies are not made or distributed for profit or commercial advantage and that copies bear this notice and the full citation on the first page. Copyrights for components of this work owned by others than the author(s) must be honored. Abstracting with credit is permitted. To copy otherwise, or republish, to post on servers or to redistribute to lists, requires prior specific permission and/or a fee. Request permissions from [permissions@acm.org](mailto:permissions@acm.org).

K-CAP '19, November 19–21, 2019, Marina Del Rey, CA, USA

© 2019 Copyright held by the owner/author(s). Publication rights licensed to ACM.

ACM ISBN 978-1-4503-7008-0/19/11...\$15.00

<https://doi.org/10.1145/3360901.3364423>

Augmentation. In *Proceedings of the 10th International Conference on Knowledge Capture (K-CAP '19)*, November 19–21, 2019, Marina Del Rey, CA, USA. ACM, New York, NY, USA, 9 pages. <https://doi.org/10.1145/3360901.3364423>

## 1 INTRODUCTION

Neural Network (NN) models have shown significant improvements in translation generation and have been widely adopted due to their consistent improvements over the Phrase-Based Statistical Machine Translation (PBSMT) approaches [20]. A number of Neural Machine Translation (NMT) architectures have been proposed in recent years, ranging from recurrent [4] to self-attentional networks [45]. However, a major drawback of these models is that they need large amounts of training data to return adequate results and have a limited vocabulary size due to their computational complexity [25]. The data sparsity problem in Machine Translation (MT), which is mostly caused by the lack of training data, manifests itself in particular in a poor translation of out-of-vocabulary (OOV) words, e.g., entities or terminological expressions rarely or never seen in the training data.

Previous work has attempted to deal with the data sparsity problem by introducing character-based models [25] and Byte Pair Encoding (BPE) algorithms [38]. Also, different strategies were devised for overcoming the lack of training data, for instance, back-translation [37], which relies on the use of monolingual data being translated by a different NMT model and added as additional synthetic training data. In addition, pre-trained monolingual word embeddings were used for leveraging the embedding matrix of low-resource NMT models [34]. Moreover, distinct external knowledge injection approaches have been tried for guiding the NNs to use domain-specific data while translating, for example, ontologies [1, 2].

Despite the significant advancement of previous work in NMT, translating entities and terminological expressions remains a challenge. In detail, entities can be classified into two groups, i.e., proper nouns and common nouns. Proper nouns are also known as Named Entity (NE) and correspond to the name of people, organizations or locations, e.g., *John*, *WHO* or *Canada*. Common nouns describe classes of object, e.g., *spoon* or *cancer*. Both types of entities can

be found in a Knowledge Graph (KG),<sup>1</sup> in which they are commonly modelled as resources and described by triples. Each triple consists of a subject—often an entity—, a relation—often called property—and an object—often an entity or a literal.<sup>2</sup> For example,  $\langle \text{USA}, \text{type}, \text{Country} \rangle$ ,<sup>3</sup> corresponds to “The USA is a country” in natural language. Recent work has successfully exploited the contribution of KGs to improve Natural Language Processing (NLP) tasks such as Natural Language Inference (NLI) [17] or Question Answering (QA) [40]. Additionally, the benefits of incorporating type information on entities—e.g., NE-tags such as PERSON, LOCATION or ORGANIZATION—into NMT by relying on Named Entity Recognition (NER) systems have been studied in previous work [44]. However, none of these have exploited the combination of Entity Linking (EL) with KGs in NMT models.

The goal of EL is to disambiguate and link a given NE within a text to a corresponding resource in a reference KB. If the reference KB is bilingual, the links generated by EL can be used to retrieve the translation of entities found in the text. In this work, we aim to use EL to improve the results of NMT approaches. We build upon recent works, which have devised Knowledge Graph Embeddings (KGE)s approaches [35], i.e., approaches that embed KGs into continuous vector spaces. Since NN models learn translations in a continuous vector space, we hypothesize that a given KG, once converted to embeddings, can be used along with EL to improve NMT models. Our results suggest that with this proposed methodology, we are capable of enhancing the semantic feature extraction of neural models for gathering the correct translation of entities and consequently improving the translation quality.

To this end, we devised two strategies to address the issues stated above. In our first strategy, we annotate bilingual training data with a multilingual EL system using a reference KB. Then, we map the entities and relationships contained in the reference KB to a continuous vector space using a given KGEs technique. Finally, we concatenate the KGEs to the internal NMT embeddings, thus augmenting the embedding layer of NMT training. Given that EL can be time-consuming when faced with large training corpora, we skip the EL task in our second strategy and semantically enrich the KGEs by using the surface forms of entities to initialize the vector values at the embedding layer. Afterwards, we maximize the vector values of entities found in the bilingual corpora with the values of entities’ surface forms from the KGEs. Finally, we perform an extensive automatic and manual evaluation in order to analyze our hypothesis.

Our KG-augmented neural translation model, named KG-NMT, achieves significant and consistent improvements of +3 BLEU, ME-TEOR and chrF3 on average on the WMT *newstest* datasets between 2015 and 2018 for the English-German translation task, using a small set of two million parallel sentences. Also, we observed that the use of the reference KG contributes to the translation of domain-specific datasets and ontologies in the medical, financial and Information Technology (IT) domain. To the best of our knowledge, no previous work has investigated the augmentation of NMT by using KGs without affecting the NN architecture. Hence, the main contribution of this paper lies in the investigation of two different strategies

for integrating KGEs into neural translation models in order to maximize the probability score of the translation of entities. All data to train and augment the neural models along with its code are publicly available.<sup>4</sup>

## 2 RELATED WORK

In this section, we give an overview of related work on 1) using external structured knowledge within NMT, 2) challenges posed by NE in NMT and 3) the development of KGEs.

**External Structured Knowledge in MT.** The idea of using a structured KB in MT systems started with the works of Goodman and Nirenburg [12]. Still, only a few researchers have designed different strategies for benefiting of structured knowledge in MT architectures [2]. Recently, the idea of using KG into MT systems has gained renewed attention. Du et al. [9] created an approach to address the problem of OOV words by using BabelNet [30]. Their approach applies different methods of using BabelNet. In summary, they create additional training data and apply a post-editing technique, which replaces the OOV words while querying BabelNet. Shi et al. [39] have recently built a semantic embedding model reliant upon a specific KB to be used in NMT systems. The model relies on semantic embeddings to encode the key information contained in words so as to translate the meaning of sentences correctly. The work consists of mapping a source sentence to triples, which are then used to extract the intrinsic meaning of words to generate a target sentence. This mapping results in a semantic embedding model containing KB triples, which are responsible for gathering the key information of each word in the sentences.

**Named Entities in NMT.** Only a few works have investigated the NE translation issue. Some researchers worked on models specific to this problem, while others incorporated external information as features within NMT models. Wang et al. [46] rely on a NER tool to identify and align the NE pairs within the source and target sentences. Afterwards, the NE pairs are replaced with their corresponding NE-tags to train the model. In the translation phase, the targeted NE tags are then substituted with the original entities by a separate NE translation model or a bilingual NE dictionary. Ugawa et al. [44] used a similar architecture but included one more layer in the encoder to encode the NE-tags expressed as chunk tags at each time step. The disadvantages of the methods above include NE information loss and NE alignment errors. To overcome these problems, Li et al. [23] relied on an effective and simple method, which added the NE-tags as boundary information to the entities directly inserted by a NER tool in the source sentence. It does not require either any separate model or external resource, and it, therefore, does not affect the NN architecture while achieving good performance.

**Knowledge Graph Embeddings.** Annervaz et al. [17] classifies KGEs into two categories: (1) Structure-based, which encodes only entities and relations, (2) Semantically-enriched, which takes into account semantic information of entities, e.g., text, along with the entities and its relations. Manifold approaches, where relationships are interpreted as displacements operating on the low-dimensional embeddings of the entities, have been implemented so far, such as TransE [7]. Recently, Ristoski and Paulheim [35] presented RDF2Vec, which uses language modelling approaches

<sup>1</sup>In this paper, we use KG and Knowledge Base (KB) interchangeably.

<sup>2</sup>a string or a value with a unit

<sup>3</sup><http://dbpedia.org/page/USA>

<sup>4</sup><https://github.com/dice-group/KG-NMT>

for unsupervised feature extraction from sequences of words and adapts them to Resource Description Framework (RDF) graphs. In its subsequent extension, Cochez et al. [8] exploited the Global Vectors algorithm in RDF2Vec for computing embeddings from the co-occurrence matrix of entities and relations without generating the random walks. However, Joulin et al. [16] showed recently that a simple Bag-of-Words (BoW) based approach with the *fastText* algorithm [15] generates surprisingly good KGEs while achieving the state-of-the-art results. Wang et al. [47] proposed a technique of learning to embed structured and unstructured data (such as text) jointly in an effort to augment the prediction models. Additionally, Zhong et al. [48] introduced an alignment of entities and word embeddings considering the description of entities. More work on agglutinating the semantics with entities arose, such as LiteralE [22], which enriches the KGEs with numerical literals.

### 3 THE KG-NMT METHODOLOGY

KG-NMT is based on the observation that more than 150 billion facts referring to more than 3 billion entities are available in the form of KG on the Linked Open Data (LOD) Cloud.<sup>5</sup> Hence, the intuition behind our methodology is as follows: *Given that KGs describe real-world entities, we can use a KGs along with EL to optimize the embedding vector of entities and consequently to achieve a better translation quality of entities in text.* In the following, we give a formal overview of NMT and KGEs. Afterwards, we present how we use EL and KGEs to augment NMT models. Throughout the description of our methodology and our experiments, we use DBpedia [3] as reference KB due to its great coverage of languages [11] as well as EL systems have shown to perform best on DBpedia [27].

#### 3.1 Background

**Neural Machine Translation.** In this work, we use the Recurrent Neural Network (RNN) architecture. It consists of an encoder and a decoder, i.e., a two-tier architecture where the encoder reads an input sequence  $x = (x_1, \dots, x_n)$  and the decoder predicts a target sequence  $y = (y_1, \dots, y_n)$ . The encoder and decoder interact via a soft-attention mechanism [4, 26], which comprises of one or multiple attention layers. We follow the notations from Tang et al. [42] in the subsequent sections:  $h_i^l$  corresponds to the hidden state at step  $i$  of layer  $l$ .  $h_{i-1}^l$  represents the hidden state at the previous step of layer  $l$  while  $h_i^{l-1}$  means the hidden state at  $i$  of  $l-1$  layer.  $E \in \mathbb{R}^{m \times K_x}$  is a word embedding matrix,  $W \in \mathbb{R}^{n \times m}$ ,  $U \in \mathbb{R}^{n \times n}$  are weight matrices, with  $m$  being the word embedding size and  $n$  the number of hidden units.  $K_x$  is the vocabulary size of the source language. Thus,  $E_{x_i}$  refers to the embedding of  $x_i$ , and  $e_{pos,i}$  indicates the positional embedding at position  $i$ . In RNN models, networks change as new inputs (previous hidden state and the token in the line) come in, and each state is directly connected to the previous state only. Therefore, the path length of any two tokens with a distance of  $n$  in RNNs is exactly  $n$ . Its architecture enables adding more layers, whereby two adjoining layers are usually connected with residual connections in deeper configurations. Equation 1 displays  $h_i^l$ , where  $f_{rnn}$  is usually a function based on Gated recurrent unit (GRU) or Long Short-Term Memories (LSTM). The first layer

is then represented as  $h_i^0 = f_{rnn}(WE_{x_i}, Uh_{i-1}^0)$ . Additionally, the initial state of the decoder is commonly initialized with the average of the hidden states or the last hidden state of the encoder.

$$h_i^l = h_{i-1}^{l-1} + f_{rnn}(h_{i-1}^{l-1}, h_{i-1}^l) \quad (1)$$

**Knowledge Graph Embeddings.** The underlying concept of KGEs is that, in a given KB, each subject  $h$  or object  $t$  entity can be associated as a point in a continuous vector space whereby its relation  $r$  can be modelled as displacement vectors ( $h + r = t$ ) while preserving the inherent structure of the KG. In the methodology introduced by [16], named *fastText*, the model is based on BoW representation, which considers the subject  $h$  and object  $t$  entities along with its relation  $r$  as a unique discrete token. Thus, *fastText* models the co-occurrences of entities and its relations with a linear classifier, e.g., a linear regression [10], and standard cost functions. Hence, it allows theoretically creating either a structure-based or semantically-enriched KGEs. We reproduced the experiments from [16] along with a sub-set of DBpedia and *fastText* achieved the best results. Therefore, we decided to use it in our experiments,<sup>6 7 8</sup>

represented by the following Equation 2.

$$-\frac{1}{N} \sum_{n=1}^N y_n \log(f(WVz_n)), \quad (2)$$

#### 3.2 Methodology

Recent work has successfully devised strategies for incorporating different kinds of knowledge into NMT models, such as NE-tags [23]. Instead of training a given NMT model on a large amount of parallel data with the aim of improving the translation of entities, our idea relies on EL solutions, which can disambiguate the entities found in a text to translate by mapping them to a corresponding resource from a given reference KG. According to Koehn and Knowles [21], a large amount of training data improves the translation quality but is not able to translate entities if they rarely appear in training data. In turn, we hypothesize that a bilingual KG, such as DBpedia, may support the learning of a neural translation model through its graph structure, i.e., the translation of a given entity is easier to be learned via the graph's edges instead of estimating the few appearances of this entity along its neighbour words in a bilingual training data. Additionally, we reckon that the NE-tags are given implicitly by the resources and predicates contained in the KB. For example, *Angela Merkel* is typed as a PERSON in DBpedia. Figure 1 depicts the general idea of our methodology.

Formally, we substantiate our methodology on the two following definitions of EL and KB.<sup>9</sup>

**Definition 3.1.** Entity Linking: Let  $\mathcal{E}$  be a set of entities from a KB and  $\mathcal{D}$  be a document containing potential mentions of entities  $\mathbf{m} = (m_1, \dots, m_n)$ . The goal of an EL system is to generate an assignment  $\mathcal{F}$  of mentions to entities with  $\mathcal{F}(\mathbf{m}) \in (\mathcal{E})^n$  for the document  $\mathcal{D}$ .

**Definition 3.2.** Knowledge Base: We define KB  $K$  as a directed graph  $G_K = (V, R)$  where the nodes  $V$  are resources of  $K$ , the edges  $R$  are properties of  $K$  and  $h, t \in V, (h, t) \in R \Leftrightarrow \exists r : (h, r, t)$  is a triple in  $K$ .

<sup>6</sup><https://github.com/facebookresearch/fastText/tree/master/scripts/kbcompletion/>

<sup>7</sup>We could not use RDF2Vec in our work as its code was incomplete.

<sup>8</sup><https://git.io/KG-NMT-experiments-KGE>

<sup>9</sup>We assume that all mentions can be linked to entities in the KB.

<sup>5</sup><http://lod-cloud.net/>

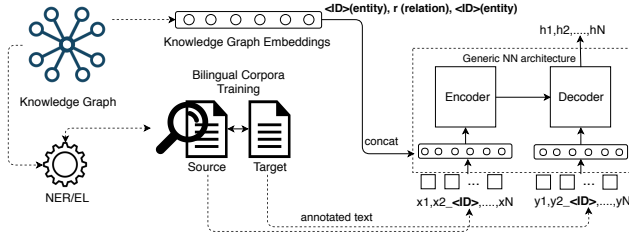

**Figure 1: Overview of the KG-NMT methodology.**

We devised two strategies to instantiate our methodology. In the first strategy, we link the NEs in the source and target texts to a reference KB, i.e., DBpedia, using MAG [28], a multilingual EL system. We then incorporate the Uniform Resource Identifier (URI)s of entities along with the tokens akin to Li et al. [23] with the NE-tags. For example, the word *Kiwi* can be annotated with *Kiwi* | *dbr\_Kiwi*<sup>10</sup> or *dbr\_Kiwi\_(people)*, depending on the context. Similarly, the word *cancer* can be annotated with *cancer* | *dbr\_Cancer*,<sup>11</sup> and its translation represented in the German part of the DBpedia KB (*dbr\_Krebs\_(Medizin)*). After incorporating the URIs, we embed the reference KB, using the *fastText* KGE algorithm. Once the KGEs are created, we concatenate their vectors to the internal vectors of NMT embeddings. The concatenation is possible as the annotations are present in the texts and consequently in the vocabulary. We chose to concatenate the vectors instead of leveraging their values because the concatenation preserves the values of KGEs while leveraging loses its original values. In case a given entity in the text does not have a vector in the KGEs, the concatenation inserts an empty vector, while the performance of NMT remains unaffected. For example, suppose the entity “USA” appears in the parallel training data, i.e., a 500 dimensional vectors space is learned. Likewise, it also appears in the KG, thus a vector space of the same dimension is learned. After concatenation, the *USA* embedding becomes 2x500 dimensions, whereby entities, which are not present in the KGEs are concatenated with an empty 500 dimensional vector. Formally, let the tokens from the source and target text be elements of a fixed vocabulary  $\mathcal{D}$ , which are used to train a given NMT model, while the assignments  $\mathcal{F}$  are the nodes  $V$  within KB  $K$ . The embeddings  $E'$  of  $K$  can be concatenated along with the internal embeddings of NMT  $E$  using a function  $concat(E, E')$ , thus resulting in a new vector  $E_c$ . With this modification the first layer of an RNN becomes  $h_i^0 = f_{rnn}(WE_{cx_i}, Uh_{i-1}^0)$ .

Although incorporating EL as a feature into NMT is interesting by itself, the annotation of entities in the training set and the post-editing task can be resource-intensive. Additionally, one limitation of structure-based KGEs is that it can only work with word-based models since the application of any segmentation model, such as BPE, on entities and relations may force the algorithm to assign wrong vectors to the entities. BPE is a form of data compression that iteratively replaces the most frequent pair of bytes in a sequence with a single, unused byte. For example, the entities *dbr:Leipzig* and *dbr:Leibniz*<sup>12</sup> can be similar when considering sub-word units (characters), however, the first is a location while

the second is a person. Both entities can be connected via the entity *dbr:University\_of\_Leipzig* but in this case, we are analyzing the sub-word units and not their graph connections. Thus, they should not be regarded as similar in the perspective of entities.

To overcome this limitation, we devise our second strategy, which uses only semantically-enriched KGEs and skips the EL part. Here, we enrich the structure-based KGEs with surface forms of the entities found in the DBpedia KB, thus decreasing the annotation effort and allowing the use of segmentation-models, i.e., sub-word information, on the surface forms differently from the first strategy, which considered only entities. Our hypothesis lies in the unsupervised learning capability of NNs, which can predict the annotation and alignment of the entities by itself. To generate the semantically-enriched KGEs, we rely on multinomial logistic regression [6] as a classifier in a supervised training implemented in *fastText* which assigns labels to the vector representations. The classification task creates inverse relations among the resources in order to map the relation of the subjects and objects in the triples and also it assigns a label, in this case, the entity’s URI, to the surface forms of entities and include them in the same vector space. The goal of the task is to predict the URIs of entities by their surface form. For example, we add to the triple,  $\langle \text{USA}, \text{type}, \text{Country} \rangle$  the following information,  $\langle \text{USA}, \text{surfaceForm}, \text{United States of America} \rangle$ . Thus, the training data looks `__label__dbr:USA United States America`.<sup>13</sup> The classifier creates an additional (hidden) relational vector between every entity (labels) and their associated words. Thus, the model when asked for the label of “United States of America” returns *dbr:USA*. However, we do not rely on the complete model rather we use the KGE generated output with the surface forms attached in it. The semantically-enriched-KGEs training jointly embeds entities and words into the same vector space, thus generating a vector for every word, which composes the entity’s label. Therefore, while learning the KGE along with the NMT vocabulary, the NN can retrieve from the lookup table the surface forms of entities and use their labels URIs to align both source and target entities. By enriching the KGEs with surface forms, it allows using these vectors to initialize the embedding layer’s weights of the NMT models. This initialization is similar to the one used with pre-trained monolingual embeddings in NMT [31]. But, instead of containing various words, the semantically-enriched KGEs has only the surface forms of the entities, which are also present in the NMT vocabulary. The default initialization of the embeddings layer is a function, which assigns random values to the weight matrix  $W$ , whereas, in our second strategy, the values from KGEs  $E'$  matrix are used to assign constant values to the matrix  $W$  using a function  $init(E')$ . Moreover, the employment of semantically-enriched KGEs prevents some errors from the alignment of entities from source and target texts. For example, the entity linker runs in two distinct instances for each language, thus in case a certain entity is annotated only on the source or on the target language side, the NMT approach is affected as the translation task requires aligned bilingual parallel texts for training.

<sup>10</sup><http://dbpedia.org/resource/Kiwi>

<sup>11</sup><http://dbpedia.org/resource/Cancer>

<sup>12</sup>Subword segmentation (BPE) - Leipzig: Le ■ ip ■ zig ; Leibniz: Le ■ ib ■ n ■ iz

<sup>13</sup>More than one surface forms can be assigned to the entities.

## 4 EXPERIMENTAL SETUP

Different NN architectures are hard to compare as they are susceptible to hyper-parameters. Therefore, we follow the idea of using a minimal reasonable configuration set to the NMT in order to fairly analyze the contributions of the used KG.

**NMT Framework.** For our overall experiments, we used a bi-directional RNN-LSTM 2-layer encoder-decoder model with attention mechanism [4]. The training uses a batch size of 32 and the stochastic gradient descent with an initial learning rate of 0.0002. We set a source and target word embeddings’ size of 500, and hidden layers to size 500, dropout = 0.3 (naive). We used a maximum sentence length of 80, a vocabulary of 50,000 words for the word based models and a beam size of 5. All experiments were performed with OpenNMT [18]. In addition, we used a copy mechanism for investigating the OOV words issue. This mechanism first tries to substitute the OOV words with target words that have the highest attention weight according to their source words [26]. When the words are not found, it copies the source words to the position of the not-found target word [14]. Moreover, we encoded words using BPE with 32,000 merge operations to achieve an open vocabulary as it has shown good results in previous work. Therefore, we created three kinds of baseline models (word-based, copyM, BPE32) using all the options mentioned above for evaluating the quality of the translation models. For training the NMT models, we attempted to be as generic as possible. Our training set consists of a merge of the initial one-third of JRC-Acquis 3.0 [41], Europarl [19], and OpenSubtitles2013 [43], obtaining a parallel training corpus of two million sentences, containing around 38M running words. We perform our experiments on the English-German language pair as it is one of the most evaluated language pairs in the evaluation campaigns and translating into German is challenging in itself, due to its complex morphology and compounding.

**NMT Augmentation.** For augmenting the three baseline models with our two KG-based strategies, we annotate the parallel bilingual corpora with MAG (first strategy), a multilingual EL system [28], which is language and KB agnostic. Although it does not require any training, it has shown competitive results according to the benchmarking platform GERBIL [36]. Afterwards, we trained the KGEs, with a vector dimension size of 500 and a window size of 50 using hierarchical softmax. For semantically-enriched KGEs, we added the surface forms whereby we used the same BPE models on it. For the sake of comparison, we dubbed the KG-NMT approach that relies on EL and structured-based KGEs (first strategy) as *KG-NMT (EL+KGE)* and the version with semantic information (second strategy) is named *KG-NMT (SemKGE)*. For overcoming both limitations of *fastText*, which are having a clean KB and information of local graph connectivity, we relied on specific sub-sets of the English and Germany DBpedia KG which contain transitive and Concise Bounded Description (CBD) resources along with their surface forms.<sup>14</sup> The English KB contains 4.2 million entities, 661 relations, and 2.1 million surface forms, while the German version has 1 million entities, 249 relations, and 0.5 million surface forms.

**Evaluation Metrics.** We used three automatic MT standard metrics to ensure a consistent and clear evaluation on the common evaluation datasets of the WMT evaluation shared tasks, named

*newstest*, between 2015 and 2018 as well as on the domain-specific datasets. BLEU [32] uses a modified precision metric for comparing the MT output with the reference (human) translation. The precision is calculated by measuring the n-gram similarity ( $n=1,...,4$ ) at the word level. BLEU also applies a brevity penalty by comparing the length of the MT output with the reference translation. METEOR [5] was mainly introduced to overcome the semantic weakness of BLEU. To this end, METEOR considers stemming and paraphrasing along with standard exact word (or phrase) matching. chrF3 [33] exploits the use of character n-gram precision and recall (F-score) for automatic evaluation of MT outputs. chrF3 has shown a good correlation with human rankings of different MT outputs and is simple and does not require any additional information. Moreover, we carried out a manual analysis of outputs for assuring the contribution from KGs, DBpedia, and we investigated the use of KG in other settings as follows:

**Monolingual Embeddings vs. KGEs.** Here, we aim to compare the performance of an NMT using pre-trained monolingual embeddings with the semantically-enriched KGEs as both can be used to initialize the internal vectors’ values of an NMT model. Our focus is to analyze if the KGEs with fewer vectors can perform better than the monolingual embeddings for addressing the translation of entities and terminologies. Commonly, pre-trained monolingual word embeddings are used when the bilingual training data of a given language pair is scarce. These monolingual embeddings can be used to maximize the vector values of both, source or target languages as they usually are trained on a large monolingual corpus. Thus, we used a pre-trained monolingual embeddings model, which has 9.2 billion words for English and another with 1.3 billion words for German from [13]. The NMT model maximized the pre-trained monolingual embedding is dubbed as *biRNN+MonoE*.

### Continuous Training on Domain-Specific Parallel Datasets.

A recent survey [29] showed that the LOD cloud contains a variety of multilingual KGs from diverse domains, which may be used to improve the quality of MT systems. Therefore, our goal is to inspect the capability of improving the domain-specific translations using KGs since they document domain-specific information. To this end, we relied on the continued training technique [24] to adapt a generic NMT system to the financial, medical and IT domain. For the financial domain, we used the International Financial Reporting Standards (IFRS) ontology and divided the documented labels into training (for continued training), development and test set, containing 1,000 labels each. Similarly, we used the International Classification of Diseases (ICD)-10 ontology, with 1,000 labels in the medical domain for the continued training, development and test set. Finally, for the IT domain, we used the IT-WMT16<sup>15</sup> sets. The continued training set contains 50,121, the development 2,000 and test 1,000 sentences. We followed the same methodology described in section 3.2 to insert the DBpedia KG in the domain adapted models. The adapted models are named *KG-NMT(EL+KGE)\_adapt* and *KG-NMT(SemKGE)\_adapt* respectively.

<sup>14</sup>The files are mappingbased\_objects, labels, and interlinking\_languages

<sup>15</sup><http://www.statmt.org/wmt16/it-translation-task.html>

**Table 1: Results in BLEU, METEOR, chrF3 on WMT newstest datasets.**

| Models            |                     | newstest2015 |              |              | newstest2016 |              |              | newstest2017 |              |              | newstest2018 |              |              |
|-------------------|---------------------|--------------|--------------|--------------|--------------|--------------|--------------|--------------|--------------|--------------|--------------|--------------|--------------|
|                   |                     | BLEU         | METEOR       | chrF3        | BLEU         | METEOR       | chrF3        | BLEU         | METEOR       | chrF3        | BLEU         | METEOR       | chrF3        |
| Word-based models | biRNN-lstm baseline | 16.77        | 35.20        | 41.11        | 18.55        | 36.62        | 42.54        | 15.10        | 33.75        | 39.52        | 20.53        | 39.02        | 43.92        |
|                   | KG-NMT(EL+KGE)      | 19.86        | 38.25        | 42.92        | 22.38        | 40.40        | 45.18        | 18.04        | 36.94        | 41.55        | 24.87        | 43.49        | 46.88        |
|                   | KG-NMT(SemKGE)      | <b>21.49</b> | <b>40.19</b> | <b>44.72</b> | <b>24.01</b> | <b>42.47</b> | <b>46.84</b> | <b>19.66</b> | <b>38.89</b> | <b>43.11</b> | <b>27.02</b> | <b>45.77</b> | <b>48.70</b> |
| CopyM models      | biRNN-lstm baseline | 19.63        | 39.20        | 46.38        | 21.37        | 40.90        | 47.85        | 17.88        | 37.89        | 44.85        | 24.22        | 43.96        | 50.15        |
|                   | KG-NMT(EL+KGE)      | 22.46        | 41.67        | 48.28        | 25.05        | 44.23        | 50.66        | 20.77        | 40.58        | 47.04        | 28.44        | 47.86        | 53.25        |
|                   | KG-NMT(SemKGE)      | <b>24.08</b> | <b>43.43</b> | <b>49.72</b> | <b>26.70</b> | <b>46.08</b> | <b>52.05</b> | <b>22.30</b> | <b>42.37</b> | <b>48.36</b> | <b>30.55</b> | <b>49.92</b> | <b>54.71</b> |
| BPE models        | biRNN-lstm baseline | 15.89        | 36.51        | 45.97        | 21.95        | 42.88        | 52.68        | 16.80        | 39.12        | 49.35        | 23.85        | 45.85        | 54.98        |
|                   | KG-NMT(EL+KGE)      | N/A          | N/A          | N/A          | N/A          | N/A          | N/A          | N/A          | N/A          | N/A          | N/A          | N/A          | N/A          |
|                   | KG-NMT(SemKGE)      | <b>21.74</b> | <b>41.41</b> | <b>50.04</b> | <b>24.86</b> | <b>44.32</b> | <b>53.59</b> | <b>20.45</b> | <b>40.62</b> | <b>49.45</b> | <b>28.02</b> | <b>47.51</b> | <b>55.16</b> |

## 5 EVALUATION

In this section, we report the results of our experiments and perform a manual analysis of each experimental setting to answer the following research questions:

- Q1: Can an NMT model enhanced with a bilingual KG improve translation quality?
- Q2: Which method performs best on NMT, supervised annotation with EL + KGEs or unsupervised annotation with only semantically-enriched KGEs?
- Q3: Are KGEs more effective than pre-trained monolingual word embeddings for improving the translation of entities in NMT?
- Q4: Can KGEs be employed for translating domain-specific knowledge?

**Overall Results.** Table 1 shows the results for *KG-NMT* models in comparison to the baselines on the *newstest* dataset between 2015 and 2018. Using KGEs leads to a clear improvement over the baseline as it significantly improved the translation quality in terms of BLEU (+3), METEOR (+4) and chrF3 (+3) metrics. *KG-NMT (SemKGE)* outperformed *KG-NMT (EL+KGE)* by around +1.3 in BLEU and chrF3, while we observed a +2 point improvement for METEOR. This difference between the contribution of KGE types is directly related to the EL performance, which did not manage to annotate all kind of entities present in the text. Consequently, the RNN was not able to learn the translations of entities from the DBpedia KG. A different EL which is able to disambiguate more types of entities can improve the results of *KG-NMT (EL+KGE)*, but still its training time is considerable longer than *KG-NMT (SemKGE)*. The augmented model on BPE, *KG-NMT (SemKGE)*, presented consistent improvements showing that the model was capable of learning the segmentation applied on surface forms when translating to morphologically complex languages, such as German. We observed that the copy mechanism can be beneficial for named entities, which were not found in KG. These entities were copied from the source language and added consequently as a translation to the target language. For example, *Chad Johnston* was copied from the source into the target languages as a translation, since this name was not found in the KB.

A detailed study of our results showed that the number of OOV words decreased considerably with the augmentation through KGEs. Table 2 shows the number of OOV words generated by the models across all WMT *newstest* datasets. The statistics cannot ensure that every OOV word that became a known word was essentially an entity presented in DBpedia KG. Thus, we chose the *newstest2015*

**Table 2: Number of OOV words across a baseline NMT model and KG-NMT models on the *newstest* dataset.**

| Models              | 2015  | 2016  | 2017  | 2018  |
|---------------------|-------|-------|-------|-------|
| biRNN-lstm baseline | 6,004 | 9,559 | 9,707 | 9,383 |
| KG-NMT(EL+KGE)      | 4,427 | 6,524 | 6,603 | 6,914 |
| KG-NMT(SemKGE)      | 4,067 | 5,990 | 6,130 | 6,236 |

for a manual analysis.<sup>16</sup> We observed that many OOV words, which became known were in fact entities contained in the KG. As an example (*newstest2015* line 1265), the acronym *UK* was not translated by the *biRNN-lstm* baseline even when the copy mechanism (*UK*) or BPE (*Britische*) was used. However, it was correctly translated into German as *Großbritannien* by both KGEs augmented models. Similarly, the entity *Coastguard* (line 1540) was not translated correctly by the baseline models, whereby both KGEs models were able to translate it correctly into *Küstenwache*. Moreover, *KG-NMT (EL+KGE)* was able to translate the word *teacher* (line 438) correctly into *Lehrer* using the knowledge acquired from KG.<sup>17</sup> This human evaluation confirms our hypothesis and answer the **Q1** and **Q2** research questions by showing that the KG-augmented RNN models were able to correctly learn the translation of entities through the relations found in KGEs and that *KG-NMT (SemKGE)* improved generally the translation quality in comparison to other NMT models, which means a supervised annotation of entities with EL is not entirely necessary.

**Time-Performance.** The NMT baseline model with around two million parallel sentences took in average three days using GPU 1080i 6G for training. Regarding the training time of each strategy, the *KG-NMT (EL+KGE)* took approximately five more days than *KG-NMT (SemKGE)*, which was trained in four days (baseline time and an additional day for training the semantically-enriched KGE). The difference is regarded to the task of entity linking. Although MAG has a polynomial time complexity and annotated around five sentences per second, the overall annotation was time-consuming in a corpus of two million sentences. The semantically-enriched KGE took 12 hours more in comparison to the structured-KGE, which was caused by the classification task.

**Monolingual Embeddings vs KGEs.** Table 3 reports no significant difference between monolingual embeddings and KGEs in terms of BLEU, METEOR and chrF3. This finding is interesting since the monolingual embeddings contain billions of words, compared to the DBpedia KG with 4.2 million entities. Taking a deeper

<sup>16</sup> our full analysis of the entities' translation can be found in <https://git.io/KG-NMT-experiments-entities>

<sup>17</sup> <http://dbpedia.org/resource/Teacher>

Table 3: Comparison between pre-trained monolingual embeddings and KGEs.

| Models            |                  | newtest2015 |        |       | newtest2016 |        |       | newtest2017 |        |       | newtest2018 |        |       |
|-------------------|------------------|-------------|--------|-------|-------------|--------|-------|-------------|--------|-------|-------------|--------|-------|
|                   |                  | BLEU        | METEOR | chrF3 | BLEU        | METEOR | chrF3 | BLEU        | METEOR | chrF3 | BLEU        | METEOR | chrF3 |
| Word-based models | biRNN-lstm+MonoE | 21.59       | 40.54  | 45.37 | 24.12       | 42.82  | 47.37 | 20.05       | 39.42  | 43.90 | 27.15       | 46.13  | 49.35 |
|                   | KG-NMT(SemKGE)   | 21.49       | 40.19  | 44.72 | 24.01       | 42.47  | 46.84 | 19.66       | 38.89  | 43.11 | 27.02       | 45.77  | 48.70 |
| CopyM models      | biRNN-lstm+MonoE | 24.21       | 43.81  | 50.32 | 26.97       | 46.52  | 52.61 | 22.61       | 42.87  | 49.01 | 30.77       | 50.39  | 55.41 |
|                   | KG-NMT(SemKGE)   | 24.08       | 43.43  | 49.72 | 26.70       | 46.08  | 52.05 | 22.30       | 42.37  | 48.36 | 30.55       | 49.92  | 54.71 |
| BPE Models        | biRNN-lstm+MonoE | 19.65       | 39.24  | 47.58 | 25.13       | 44.66  | 53.54 | 20.93       | 41.41  | 50.33 | 28.42       | 48.00  | 55.98 |
|                   | KG-NMT(SemKGE)   | 21.74       | 41.41  | 50.04 | 24.86       | 44.32  | 52.59 | 20.45       | 40.62  | 49.45 | 28.02       | 47.51  | 55.16 |

Table 4: Results of models in BLEU, METEOR, chrF3 on domain-specific testsets.

| Models            |                           | ICD-10 |        |       | IFRS  |        |       | IT    |        |       |
|-------------------|---------------------------|--------|--------|-------|-------|--------|-------|-------|--------|-------|
|                   |                           | BLEU   | METEOR | chrF3 | BLEU  | METEOR | chrF3 | BLEU  | METEOR | chrF3 |
| Word-based models | biRNN-lstm baseline_adapt | 15.31  | 23.27  | 29.63 | 52.59 | 60.59  | 62.04 | 11.57 | 28.04  | 30.50 |
|                   | KG-NMT(EL+KGE)_adapt      | 21.08  | 31.07  | 36.93 | 52.38 | 60.55  | 61.86 | 21.78 | 40.29  | 42.75 |
|                   | KG-NMT(SemKGE)_adapt      | 20.79  | 30.70  | 37.00 | 51.58 | 59.18  | 60.05 | 23.41 | 41.71  | 44.42 |
| CopyM models      | biRNN-lstm baseline_adapt | 16.59  | 26.49  | 39.12 | 52.91 | 61.68  | 64.34 | 13.87 | 31.61  | 36.10 |
|                   | KG-NMT(EL+KGE)_adapt      | 22.59  | 34.54  | 46.89 | 52.72 | 61.97  | 64.65 | 25.31 | 44.24  | 48.96 |
|                   | KG-NMT(SemKGE)_adapt      | 22.24  | 34.10  | 46.74 | 51.91 | 60.33  | 62.51 | 26.84 | 45.81  | 50.38 |
| BPE Models        | biRNN-lstm baseline_adapt | 41.98  | 50.81  | 66.87 | 66.74 | 74.83  | 84.52 | 27.83 | 47.01  | 55.91 |
|                   | KG-NMT(EL+KGE)_adapt      | N/A    | N/A    | N/A   | N/A   | N/A    | N/A   | N/A   | N/A    | N/A   |
|                   | KG-NMT(SemKGE)_adapt      | 41.44  | 50.54  | 66.12 | 66.21 | 74.45  | 84.07 | 28.04 | 47.30  | 55.68 |

look, our manual analysis showed that the OOV words addressed by the monolingual embeddings were not in fact entities, but common words and the entities remained unknown. As an example, the *RNN+MonoE* model translated incorrectly the entity *Principal* into *Wichtigste*, while the *KG-NMT (SemKGE)* used the knowledge documented in the KGs.<sup>18</sup> Moreover, *RNN+MonoE* was not able to translate the entities *UK* and *Coastguard* while the *KG-NMT (SemKGE)* generated the right translations. Therefore, answering the Q3, KGEs leverage the world knowledge better than pre-trained monolingual word embeddings for translating entities and we envisage that a combination of both is promising and may lead to further translation improvements.

#### Continuous Training on Domain-Specific Parallel Datasets.

Table 4 shows that the knowledge documented in KGs is able to improve significantly the word-based models +5 BLEU, METEOR and chrF3 on the ICD-10 ontology and IT domain. However, no improvement is seen in the IFRS ontology (Financial domain) and all BPE models. Going into the data and results manually, we perceived that although the terminological expressions infrequently appear in the DBpedia KG, e.g. 14,051 entities in the medical domain in comparison to 4.2 million in the whole graph, its application in the word-based models improved fairly the translations. The same applies to the IT domain, where the evaluation metric calculates a BLEU score of 11.57 for the baseline system and 23.41 for the semantically-enriched KGEs. However, the lack of improvement in the IFRS ontology was caused by the in-domain training data used in the continued training (domain adaptation). For example, the IFRS data used for continuous training already contained terminological expressions and therefore the adapted models ignored the values from the KGEs. Differently, in the in-domain training of ICD-10 ontology and IT data, the terminological expressions do not appear. Therefore, the IFRS adapted models ignored the values from the KGEs. For this reason, no improvement is seen in the word-based models for the financial domain. Regarding the BPE models,

the explanation lies in the capability of NNs for estimating the translation of rarely seen terminological expressions when BPE is applied. Basically, the operations applied by BPE were not common due to very specific NE, for example, names of diseases, for which the NMT system was incapable of learning the translations from the KGEs. In summary, KGEs contribute to the translation of very domain-specific data, which answers our last research question Q4. However, a further investigation of BPE models in combination with KG-NMT methods is required, as they did not show consistent improvements across the targeted domains.

## 6 CONCLUSION

In this paper, we introduced an augmentation methodology, which relies on the use of KGs to improve the performance of NMT systems for translating domain-specific expressions and named entities. We devised two strategies for incorporating KGEs into NMT models, which works on word- and sub-word units-based models. Additionally, we carried out an extensive evaluation with a manual analysis, which showed consistent translation improvements provided by incorporating DBpedia KG in NMT. The overall methodology can be applied to any NMT model since it does not modify the main NMT model structure and also allows replacing different EL systems. Furthermore, our proposed methodology is language-agnostic, which allows the use of other language-based KGs. As future work, we aim at exploiting the incorporation of distinct KGEs, EL and language models, such as BERT, in other NN architectures. Additionally, we plan to investigate our methodology in the context of low-resource scenarios.

## ACKNOWLEDGMENTS

This work was supported by the German Federal Ministry of Economics and Technology (BMWi) in the project RAKI (no. 01MD19012D) and by the H2020 KnowGraphs (GA no. 860801). This work has also been supported by the German Federal Ministry of Transport and Digital Infrastructure (BMVI) in the project OPAL (no. 19F2028A)

<sup>18</sup>[http://dbpedia.org/resource/Principal\\_\(school\)](http://dbpedia.org/resource/Principal_(school)) to translate the entity correctly



as well as by the Brazilian National Council for Scientific and Technological Development (CNPq) (no. 206971/2014-1) and by Science Foundation Ireland (SFI) under Grant Number SFI/12/RC/2289, co-funded by the European Regional Development Fund.

## REFERENCES

- [1] Mihael Arcan, Mauro Dragoni, and Paul Buitelaar. 2016. Translating ontologies in real-world settings. In *Proceedings of the International Semantic Web Conference (ISWC)*. Kobe, Japan.
- [2] Mihael Arcan, Marco Turchi, and Paul Buitelaar. 2015. Knowledge Portability with Semantic Expansion of Ontology Labels. In *Proceedings of the 53rd Annual Meeting of the Association for Computational Linguistics (ACL)*. Beijing, China.
- [3] Sören Auer, Christian Bizer, Georgi Kobilarov, Jens Lehmann, Richard Cyganiak, and Zachary Ives. 2007. Dbpedia: A nucleus for a web of open data. In *The semantic web*. Springer, 722–735.
- [4] Dzmitry Bahdanau, Kyunghyun Cho, and Yoshua Bengio. 2014. Neural machine translation by jointly learning to align and translate. *arXiv preprint arXiv:1409.0473* (2014).
- [5] Satandeep Banerjee and Alon Lavie. 2005. METEOR: An Automatic Metric for MT Evaluation with Improved Correlation with Human Judgments. In *Proceedings of the ACL Workshop on Intrinsic and Extrinsic Evaluation Measures for MT and/or Summarization*. ACL, 65–72.
- [6] Dankmar Böhning. 1992. Multinomial logistic regression algorithm. *Annals of the Institute of Statistical Mathematics* 1 (1992), 197–200.
- [7] Antoine Bordes, Nicolas Usunier, Alberto Garcia-Duran, Jason Weston, and Oksana Yakhnenko. 2013. Translating embeddings for modeling multi-relational data. In *Advances in Neural Information Processing Systems*. 2787–2795.
- [8] Michael Cochez, Petar Ristoski, Simone Paolo Ponzetto, and Heiko Paulheim. 2017. Global rdf vector space embeddings. In *International Semantic Web Conference*. Springer, 190–207.
- [9] Jinhua Du, Andy Way, and Andrzej Zydron. 2016. Using BabelNet to Improve OOV Coverage in SMT. In *Proceedings of the Tenth International Conference on Language Resources and Evaluation, Portorož, Slovenia, May 23-28*. 9–15.
- [10] Rong-En Fan, Kai-Wei Chang, Cho-Jui Hsieh, Xiang-Rui Wang, and Chih-Jen Lin. 2008. LIBLINEAR: A library for large linear classification. *Journal of machine learning research* 9, Aug (2008), 1871–1874.
- [11] Michael Färber, Frederic Bartscherer, Carsten Menne, and Achim Rettinger. 2016. Linked data quality of dbpedia, freebase, openpyc, wikidata, and yago. *Semantic Web* 1, Preprint (2016), 1–53.
- [12] Kenneth Goodman and Sergei Nirenburg. 1991. *The KBMT Project: A case study in knowledge-based machine translation*. Elsevier.
- [13] Edouard Grave, Piotr Bojanowski, Prakhar Gupta, Armand Joulin, and Tomas Mikolov. 2018. Learning Word Vectors for 157 Languages. In *Proceedings of the International Conference on Language Resources and Evaluation (LREC)*.
- [14] Jiatao Gu, Zhengdong Lu, Hang Li, and Victor OK Li. 2016. Incorporating Copying Mechanism in Sequence-to-Sequence Learning. In *Proceedings of the 54th Annual Meeting of the Association for Computational Linguistics*, Vol. 1. 1631–1640.
- [15] Armand Joulin, Edouard Grave, Piotr Bojanowski, Maximilian Nickel, and Tomas Mikolov. 2017. Fast Linear Model for Knowledge Graph Embeddings. In *The NIPS 2017 AKBC Workshop*.
- [16] Annavaz K M, Somnath Basu Roy Chowdhury, and Ambedkar Dukkipati. 2018. Learning beyond Datasets: Knowledge Graph Augmented Neural Networks for Natural Language Processing. In *Proceedings of the 2018 Conference of NAACL-HLT*. ACL, 313–322.
- [17] Guillaume Klein, Yoon Kim, Yuntian Deng, Jean Senellart, and Alexander M. Rush. 2017. OpenNMT: Open-Source Toolkit for Neural Machine Translation. *Proceedings of the 55th Annual Meeting of the Association for Computational Linguistics System Demonstrations* (2017), 67–72.
- [18] Philipp Koehn. 2005. Europarl: A Parallel Corpus for Statistical Machine Translation. In *Proceedings of the 10th Machine Translation Summit*. Phuket, Thailand.
- [19] Philipp Koehn, Hieu Hoang, Alexandra Birch, Chris Callison-Burch, Marcello Federico, Nicola Bertoldi, Brooke Cowan, Wade Shen, Christine Moran, Richard Zens, et al. 2007. Moses: Open source toolkit for statistical machine translation. In *Proceedings of the 45th annual meeting of the ACL*. 177–180.
- [20] Philipp Koehn and Rebecca Knowles. 2017. Six Challenges for Neural Machine Translation. In *Proceedings of the First Workshop on Neural Machine Translation*.
- [21] Agustinus Kristiadi, Mohammad Asif Khan, Denis Lukovnikov, Jens Lehmann, and Asja Fischer. 2018. Incorporating literals into knowledge graph embeddings. *arXiv preprint arXiv:1802.00934* (2018).
- [22] Zhongwei Li, Xuancong Wang, AiTi Aw, Eng Siong Chng, and Haizhou Li. 2018. Named-Entity Tagging and Domain adaptation for Better Customized Translation. In *Proceedings of the Seventh Named Entities Workshop*. ACL, 41–46.
- [23] Minh-Thang Luong and Christopher D Manning. 2015. Stanford neural machine translation systems for spoken language domains. In *Proceedings of the International Workshop on Spoken Language Translation*. 76–79.
- [24] Minh-Thang Luong and Christopher D. Manning. 2016. Achieving Open Vocabulary Neural Machine Translation with Hybrid Word-Character Models. In *Proceedings of the 54th Annual Meeting of the Association for Computational Linguistics*. ACL, 1054–1063.
- [25] Thang Luong, Hieu Pham, and Christopher D. Manning. 2015. Effective Approaches to Attention-based Neural Machine Translation. In *Proceedings of the Conference on Empirical Methods in Natural Language Processing*. ACL, 1412–1421.
- [26] Jose L. Martinez-Rodriguez, Aidan Hogan, and Ivan Lopez-Arevalo. 2018. Information extraction meets the semantic web: a survey. *Semantic Web Preprint* (2018), 1–81.
- [27] Diego Moussallem, Ricardo Usbeck, Michael Röder, and Axel-Cyrille Ngonga Ngomo. 2017. MAG: A Multilingual, Knowledge-base Agnostic and Deterministic Entity Linking Approach. In *Proceedings of the Knowledge Capture Conference*. ACM, 9.
- [28] Diego Moussallem, Matthias Wauer, and Axel-Cyrille Ngonga Ngomo. 2018. Machine Translation Using Semantic Web Technologies: A Survey. *Journal of Web Semantics* 51 (2018), 1–19.
- [29] Roberto Navigli and Simone Paolo Ponzetto. 2012. BabelNet: The automatic construction, evaluation and application of a wide-coverage multilingual semantic network. *Artificial Intelligence* 193 (2012), 217–250.
- [30] Masato Neishi, Jin Sakuma, Satoshi Tohda, Shonosuke Ishiwatari, Naoki Yoshinaga, and Masashi Toyoda. 2017. A bag of useful tricks for practical neural machine translation: Embedding layer initialization and large batch size. In *Proceedings of the 4th Workshop on Asian Translation*. 99–109.
- [31] Kishore Papineni, Salim Roukos, Todd Ward, and Wei-Jing Zhu. 2002. BLEU: a method for automatic evaluation of machine translation. In *Proceedings of the 40th annual meeting on Association for Computational Linguistics*.
- [32] Maja Popović. 2017. chrF++: words helping character n-grams. In *Proceedings of the Second Conference on Machine Translation*. 612–618.
- [33] Ye Qi, Devendra Sachan, Matthieu Felix, Sarguna Padmanabhan, and Graham Neubig. 2018. When and Why Are Pre-Trained Word Embeddings Useful for Neural Machine Translation?. In *Proceedings of the 2018 Conference of the North American Chapter of the Association for Computational Linguistics: Human Language Technologies*, Vol. 2. 529–535.
- [34] Petar Ristoski and Heiko Paulheim. 2016. Rdf2vec: Rdf graph embeddings for data mining. In *International Semantic Web Conference*. Springer, 498–514.
- [35] Michael Röder, Ricardo Usbeck, and Axel-Cyrille Ngonga Ngomo. 2018. Gerbil-benchmarking named entity recognition and linking consistently. *Semantic Web* 9, 5 (2018), 605–625.
- [36] Rico Sennrich, Barry Haddow, and Alexandra Birch. 2016. Improving Neural Machine Translation Models with Monolingual Data. In *Proceedings of the 54th Annual Meeting of the Association for Computational Linguistics*, Vol. 1. 86–96.
- [37] Rico Sennrich, Barry Haddow, and Alexandra Birch. 2016. Neural Machine Translation of Rare Words with Subword Units. In *Proceedings of the 54th Annual Meeting of the Association for Computational Linguistics*. ACL, 1715–1725.
- [38] Chen Shi, Shujie Liu, Shuo Ren, Shi Feng, Mu Li, Ming Zhou, Xu Sun, and Houfeng Wang. 2016. Knowledge-Based Semantic Embedding for Machine Translation. In *Proceedings of the 54th Annual Meeting of the Association for Computational Linguistics*, Vol. 1. 2245–2254.
- [39] Daniil Sorokin and Iryna Gurevych. 2018. Modeling Semantics with Gated Graph Neural Networks for Knowledge Base Question Answering. In *Proceedings of the 27th International Conference on Computational Linguistics*. ACL, 3306–3317.
- [40] Ralf Steinberger, Bruno Pouliquen, Anna Widiger, Camelia Ignat, Tomaz Erjavec, Dan Tufis, and Dániel Varga. 2006. The JRC-Acquis: A multilingual aligned parallel corpus with 20+ languages. *arXiv preprint cs/0609058* (2006).
- [41] Gongbo Tang, Mathias Müller, Annette Rios, and Rico Sennrich. 2018. Why Self-Attention? A Targeted Evaluation of Neural Machine Translation Architectures. In *Proceedings of the 2018 Conference on Empirical Methods in Natural Language Processing*. 4263–4272.
- [42] Jörg Tiedemann. 2012. Parallel Data, Tools and Interfaces in OPUS. In *Proceedings of the Eight International Conference on Language Resources and Evaluation (LREC)* (23–25). European Language Resources Association (ELRA), Istanbul, Turkey.
- [43] Arata Ugawa, Akihiro Tamura, Takashi Ninomiya, Hiroya Takamura, and Manabu Okumura. 2018. Neural Machine Translation Incorporating Named Entity. In *Proceedings of the 27th International Conference on Computational Linguistics*.
- [44] Ashish Vaswani, Noam Shazeer, Niki Parmar, Jakob Uszkoreit, Llion Jones, Aidan N Gomez, Łukasz Kaiser, and Illia Polosukhin. 2017. Attention is all you need. In *Advances in Neural Information Processing Systems*. 5998–6008.
- [45] Yuguang Wang, Xiang Li, Shanbo Cheng, Liyang Jiang, Jiajun Yang, Wei Chen, Lin Shi, Yanfeng Wang, and Hongtao Yang. 2017. Sogou Neural Machine Translation Systems for WMT17. In *Proceedings of the Second Conference on Machine Translation, Volume 2: Shared Task Papers*. Association for Computational Linguistics, Copenhagen, Denmark. <http://www.aclweb.org/anthology/W17-4742>
- [46] Zhen Wang, Jianwen Zhang, Jianlin Feng, and Zheng Chen. 2014. Knowledge Graph and Text Jointly Embedding. In *EMNLP*. Citeseer, 1591–1601.



[48] Huaping Zhong, Jianwen Zhang, Zhen Wang, Hai Wan, and Zheng Chen. 2015. Aligning knowledge and text embeddings by entity descriptions. In *Proceedings*

*of the Conference on Empirical Methods in Natural Language Processing*, 267–272.
