# Supplementary material for: Knowledge Graphs for Multilingual Language Translation and Generation
Source: arXiv:2009.07715 source file (2020-09-16)
Supplement: Supplementary file 7 [file NeuralREG.pdf]

# NeuralREG: An end-to-end approach to referring expression generation

Thiago Castro Ferreira<sup>1</sup> Diego Moussallem<sup>2,3</sup> Ákos Kádár<sup>1</sup> Sander Wubben<sup>1</sup> Emiel Krahmer<sup>1</sup>

<sup>1</sup>Tilburg center for Cognition and Communication (TiCC), Tilburg University, The Netherlands

<sup>2</sup>AKSW Research Group, University of Leipzig, Germany

<sup>3</sup>Data Science Group, University of Paderborn, Germany

{tcastrof, a.kadar, s.wubben, e.j.krahmer}@tilburguniversity.edu  
moussallem@informatik.uni-leipzig.de

## Abstract

Traditionally, Referring Expression Generation (REG) models first decide on the form and then on the content of references to discourse entities in text, typically relying on features such as salience and grammatical function. In this paper, we present a new approach (NeuralREG), relying on deep neural networks, which makes decisions about form and content in one go without explicit feature extraction. Using a delexicalized version of the WebNLG corpus, we show that the neural model substantially improves over two strong baselines. Data and models are publicly available<sup>1</sup>.

## 1 Introduction

Natural Language Generation (NLG) is the task of automatically converting non-linguistic data into coherent natural language text (Reiter and Dale, 2000; Gatt and Krahmer, 2017). Since the input data will often consist of entities and the relations between them, generating references for these entities is a core task in many NLG systems (Dale and Reiter, 1995; Krahmer and van Deemter, 2012). Referring Expression Generation (REG), the task responsible for generating these references, is typically presented as a two-step procedure. First, the referential form needs to be decided, asking whether a reference at a given point in the text should assume the form of, for example, a proper name (“Frida Kahlo”), a pronoun (“she”) or description (“the Mexican painter”). In addition, the REG model must account for the different ways in which a particular referential form can be realized. For example, both “Frida” and

“Kahlo” are name-variants that may occur in a text, and she can alternatively also be described as, say, “the famous female painter”.

Most of the earlier REG approaches focus either on selecting referential form (Orita et al., 2015; Castro Ferreira et al., 2016), or on selecting referential content, typically zooming in on one specific kind of reference such as a pronoun (e.g., Henschel et al., 2000; Callaway and Lester, 2002), definite description (e.g., Dale and Haddock, 1991; Dale and Reiter, 1995) or proper name generation (e.g., Siddharthan et al., 2011; van Deemter, 2016; Castro Ferreira et al., 2017b). Instead, in this paper, we propose NeuralREG: an end-to-end approach addressing the full REG task, which given a number of entities in a text, produces corresponding referring expressions, simultaneously selecting both form and content. Our approach is based on neural networks which generate referring expressions to discourse entities relying on the surrounding linguistic context, without the use of any feature extraction technique.

Besides its use in traditional pipeline NLG systems (Reiter and Dale, 2000), REG has also become relevant in modern “end-to-end” NLG approaches, which perform the task in a more integrated manner (see e.g. Konstas et al., 2017; Gardent et al., 2017b). Some of these approaches have recently focused on inputs which references to entities are delexicalized to general tags (e.g., ENTITY-1, ENTITY-2) in order to decrease data sparsity. Based on the delexicalized input, the model generates outputs which may be likened to templates in which references to the discourse entities are not realized (as in “The ground of ENTITY-1 is located in ENTITY-2.”).

While our approach, dubbed as NeuralREG, is compatible with different applications of REG models, in this paper, we concentrate on the last one, relying on a specifically constructed set of

<sup>1</sup><https://github.com/ThiagoCF05/NeuralREG>

78,901 referring expressions to 1,501 entities in the context of the semantic web, derived from a (delexicalized) version of the WebNLG corpus (Gardent et al., 2017a,b). Both this data set and the model will be made publicly available. We compare NeuralREG against two baselines in an automatic and human evaluation, showing that the integrated neural model is a marked improvement.

## 2 Related work

In recent years, we have seen a surge of interest in using (deep) neural networks for a wide range of NLG-related tasks, as the generation of (first sentences of) Wikipedia entries (Lebret et al., 2016), poetry (Zhang and Lapata, 2014), and texts from abstract meaning representations (e.g., Konstas et al., 2017; Castro Ferreira et al., 2017a). However, the usage of deep neural networks for REG has remained limited and we are not aware of any other integrated, end-to-end model for generating referring expressions in discourse.

There is, however, a lot of earlier work on selecting the form and content of referring expressions, both in psycholinguistics and in computational linguistics. In psycholinguistic models of reference, various linguistic factors have been proposed as influencing the form of referential expressions, including cognitive status (Gundel et al., 1993), centering (Grosz et al., 1995) and information density (Jaeger, 2010). In models such as these, notions like *salience* play a central role, where it is assumed that entities which are salient in the discourse are more likely to be referred to using shorter referring expressions (like a pronoun) than less salient entities, which are typically referred to using longer expressions (like full proper names).

Building on these ideas, many REG models for generating references in texts also strongly rely on the concept of salience and factors contributing to it. Reiter and Dale (2000) for instance, discussed a straightforward rule-based method based on this notion, stating that full proper names can be used for initial references, typically less salient than subsequent references, which, according to the study, can be realized by a pronoun in case there is no mention to any other entity of same person, gender and number between the reference and its antecedents. More recently, Castro Ferreira et al. (2016) proposed a data-driven, non-deterministic model for generating referential forms, taking into

account salience features extracted from the discourse such as grammatical position, givenness and recency of the reference. Importantly, these models do not specify which contents a particular reference, be it a proper name or description, should have. To this end, separate models are typically used, including, for example, Dale and Reiter (1995) for generating descriptions, and Sidharthan et al. (2011); van Deemter (2016) for proper names.

Of course, when texts are generated in practical settings, both form and content need to be chosen. This was the case, for instance, in the GREC shared task (Belz et al., 2010), which aimed to evaluate models for automatically generated referring expressions grounded in discourse. The input for the models were texts in which the referring expressions to the topic of the relevant Wikipedia entry were removed and appropriate references throughout the text needed to be generated (by selecting, for each gap, from a list of candidate referring expressions of different forms and with different contents). Some participating systems approached this with traditional pipelines for selecting referential form, followed by referential content, while others proposed more integrated methods. More details about the models can be seen on Belz et al. (2010).

In sum, existing REG models for text generation strongly rely on abstract features such as the salience of a referent for deciding on the form or content of a referent. Typically, these features are extracted automatically from the context, and engineering relevant ones can be complex. Moreover, many of these models only address part of the problem, either concentrating on the choice of referential form or on deciding on the contents of, for example, proper names or definite descriptions. In contrast, we introduce NeuralREG, an end-to-end approach based on neural networks which generates referring expressions to discourse entities directly from a delexicalized/wikified text fragment, without the use of any feature extraction technique. Below we describe our model in more detail, as well as the data on which we develop and evaluate it.

## 3 Data and processing

### 3.1 WebNLG corpus

Our data is based on the WebNLG corpus (Gardent et al., 2017a), which is a parallel resource ini-

| Subject                | Predicate      | Object                               |
|------------------------|----------------|--------------------------------------|
| 108_St.Georges.Terrace | location       | Perth                                |
| Perth                  | country        | Australia                            |
| 108_St.Georges.Terrace | completionDate | 1988@year                            |
| 108_St.Georges.Terrace | cost           | 120 million (Australian dollars)@USD |
| 108_St.Georges.Terrace | floorCount     | 50@Integer                           |

↓

108 St Georges Terrace was completed in 1988 in Perth, Australia. It has a total of 50 floors and cost 120m Australian dollars.

Figure 1: Example of a set of triples (top) and corresponding text (bottom).

tially released for the eponymous NLG challenge. In this challenge, participants had to automatically convert non-linguistic data from the Semantic Web into a textual format (Gardent et al., 2017b). The source side of the corpus are sets of *Resource Description Framework* (RDF) triples. Each RDF triple is formed by a Subject, Predicate and Object, where the Subject and Object are constants or Wikipedia entities, and predicates represent a relation between these two elements in the triple. The target side contains English texts, obtained by *crowdsourcing*, which describe the source triples. Figure 1 depicts an example of a set of 5 RDF triples and the corresponding text.

The corpus consists of 25,298 texts describing 9,674 sets of up to 7 RDF triples (an average of 2.62 texts per set) in 15 domains (Gardent et al., 2017b). In order to be able to train and evaluate our models for referring expression generation (the topic of this study), we produced a delexicalized version of the original corpus.

### 3.2 Delexicalized WebNLG

We delexicalized the training and development parts of the WebNLG corpus by first automatically mapping each entity in the source representation to a general tag. All entities that appear on the left and right side of the triples were mapped to AGENTS and PATIENTs, respectively. Entities which appear on both sides in the relations of a set were represented as BRIDGEs. To distinguish different AGENTS, PATIENTs and BRIDGEs in a set, an ID was given to each entity of each kind (PATIENT-1, PATIENT-2, etc.). Once all entities in the text were mapped to different roles, the first two authors of this study manually replaced the referring expressions in the original target texts by their respective tags. Figure 2 shows the entity mapping and the delexicalized template for the example in Figure 1 in its versions representing the references with general tags and Wikipedia IDs.

We delexicalized 20,198 distinct texts describing 7,812 distinct sets of RDF triples, resulting in 16,628 distinct templates. While this dataset (which we make available) has various uses, we used it to extract a collection of referring expressions to Wikipedia entities in order to evaluate how well our REG model can produce references to entities throughout a (small) text.

### 3.3 Referring expression collection

Using the delexicalized version of the WebNLG corpus, we automatically extracted all referring expressions by tokenizing the original and delexicalized versions of the texts and then finding the non overlapping items. For instance, by processing the text in Figure 1 and its delexicalized template in Figure 2, we would extract referring expressions like “108 St Georges Terrace” and “It” to  $\langle \text{AGENT-1}, 108\_St\_Georges\_Terrace \rangle$ , “Perth” to  $\langle \text{BRIDGE-1}, Perth \rangle$ , “Australia” to  $\langle \text{PATIENT-1}, Australia \rangle$  and so on.

Once all texts were processed and the referring expressions extracted, we filtered only the ones referring to Wikipedia entities, removing references to constants like dates and numbers, for which no references are generated by the model. In total, the final version of our dataset contains 78,901 referring expressions to 1,501 Wikipedia entities, in which 71.4% (56,321) are proper names, 5.6% (4,467) pronouns, 22.6% (17,795) descriptions and 0.4% (318) demonstrative referring expressions. We split this collection in training, developing and test sets, totaling 63,061, 7,097 and 8,743 referring expressions in each one of them.

Each instance of the final dataset consists of a truecased tokenized referring expression, the target entity (distinguished by its Wikipedia ID), and the discourse context preceding and following the relevant reference (we refer to these as the pre- and pos-context). Pre- and pos-contexts are the lowercased, tokenized and delexicalized

| Tag       | Entity                                 |
|-----------|----------------------------------------|
| AGENT-1   | 108_St_Georges_Terrace                 |
| BRIDGE-1  | Perth                                  |
| PATIENT-1 | Australia                              |
| PATIENT-2 | 1988@year                              |
| PATIENT-3 | “120 million (Australian dollars)”@USD |
| PATIENT-4 | 50@Integer                             |

AGENT-1 was completed in PATIENT-2 in BRIDGE-1, PATIENT-1. AGENT-1 has a total of PATIENT-4 floors and cost PATIENT-3.

↓*Wiki*

108\_St\_Georges\_Terrace was completed in 1988 in Perth, Australia. 108\_St\_Georges\_Terrace has a total of 50 floors and cost 20\_million\_(Australian\_dollars).

Figure 2: Mapping between tags and entities for the related delexicalized/wikified templates.

pieces of text before and after the target reference. References to other discourse entities in the pre- and pos-contexts are represented by their Wikipedia ID, whereas constants (numbers, dates) are represented by a one-word ID removing quotes and replacing white spaces with underscores (e.g., *120\_million\_(Australian\_dollars)* for “120 million (Australian dollars)” in Figure 2).

Although the references to discourse entities are represented by general tags in a delexicalized template produced in the generation process (AGENT-1, BRIDGE-1, etc.), for the purpose of disambiguation, NeuralREG’s inputs have the references represented by the Wikipedia ID of their entities. In this context, it is important to observe that the conversion of the general tags to the Wikipedia IDs can be done in constant time during the generation process, since their mapping, like the first representation in Figure 2, is the first step of the process. In the next section, we show in detail how NeuralREG models the problem of generating a referring expression to a discourse entity.

## 4 NeuralREG

NeuralREG aims to generate a referring expression  $y = \{y_1, y_2, \dots, y_T\}$  with  $T$  tokens to refer to a target entity token  $x^{(wiki)}$  given a discourse pre-context  $X^{(pre)} = \{x_1^{(pre)}, x_2^{(pre)}, \dots, x_m^{(pre)}\}$  and pos-context  $X^{(pos)} = \{x_1^{(pos)}, x_2^{(pos)}, \dots, x_l^{(pos)}\}$  with  $m$  and  $l$  tokens, respectively. The model is implemented as a multi-encoder, attention-decoder network with bidirectional (Schuster and Paliwal, 1997) Long-Short Term Memory Layers (LSTM) (Hochreiter and Schmidhuber, 1997) sharing the same input word-embedding matrix  $V$ , as explained further.

### 4.1 Context encoders

Our model starts by encoding the pre- and pos-contexts with two separate bidirectional LSTM encoders (Schuster and Paliwal, 1997; Hochreiter and Schmidhuber, 1997). These modules learn feature representations of the text surrounding the target entity  $x^{(wiki)}$ , which are used for the referring expression generation. The pre-context  $X^{(pre)} = \{x_1^{(pre)}, x_2^{(pre)}, \dots, x_m^{(pre)}\}$  is represented by forward and backward hidden-state vectors  $(\vec{h}_1^{(pre)}, \dots, \vec{h}_m^{(pre)})$  and  $(\overleftarrow{h}_1^{(pre)}, \dots, \overleftarrow{h}_m^{(pre)})$ . The final annotation vector for each encoding timestep  $t$  is obtained by the concatenation of the forward and backward representations  $h_t^{(pre)} = [\vec{h}_t^{(pre)}, \overleftarrow{h}_t^{(pre)}]$ . The same process is repeated for the pos-context resulting in representations  $(\vec{h}_1^{(pos)}, \dots, \vec{h}_l^{(pos)})$  and  $(\overleftarrow{h}_1^{(pos)}, \dots, \overleftarrow{h}_l^{(pos)})$  and annotation vectors  $h_t^{(pos)} = [\vec{h}_t^{(pos)}, \overleftarrow{h}_t^{(pos)}]$ . Finally, the encoding of target entity  $x^{(wiki)}$  is simply its entry in the shared input word-embedding matrix  $V_{wiki}$ .

### 4.2 Decoder

The referring expression generation module is an LSTM decoder implemented in 3 different versions: Seq2Seq, CAtt and HierAtt. All decoders at each timestep  $i$  of the generation process take as input features their previous state  $s_{i-1}$ , the target entity-embedding  $V_{wiki}$ , the embedding of the previous word of the referring expression  $V_{y_{i-1}}$  and finally the summary vector of the pre- and pos-contexts  $c_i$ . The difference between the decoder variations is the method to compute  $c_i$ .

**Seq2Seq** models the context vector  $c_i$  at each timestep  $i$  concatenating the pre- and pos-context



annotation vectors averaged over time:

$$\hat{h}^{(pre)} = \frac{1}{N} \sum_i^N h_i^{(pre)} \quad (1)$$

$$\hat{h}^{(pos)} = \frac{1}{N} \sum_i^N h_i^{(pos)} \quad (2)$$

$$c_i = [\hat{h}^{(pre)}, \hat{h}^{(pos)}] \quad (3)$$

**CAtt** is an LSTM decoder augmented with an attention mechanism (Bahdanau et al., 2014) over the pre- and pos-context encodings, which is used to compute  $c_i$  at each timestep. We compute energies  $e_{ij}^{(pre)}$  and  $e_{ij}^{(pos)}$  between encoder states  $h_i^{(pre)}$  and  $h_i^{(post)}$  and decoder state  $s_{i-1}$ . These scores are normalized through the application of the softmax function to obtain the final attention probability  $\alpha_{ij}^{(pre)}$  and  $\alpha_{ij}^{(post)}$ . Equations 4 and 5 summarize the process with  $k$  ranging over the two encoders ( $k \in [pre, pos]$ ), being the projection matrices  $W_a^{(k)}$  and  $U_a^{(k)}$  and attention vectors  $v_a^{(k)}$  trained parameters.

$$e_{ij}^{(k)} = v_a^{(k)T} \tanh(W_a^{(k)} s_{i-1} + U_a^{(k)} h_j^{(k)}) \quad (4)$$

$$\alpha_{ij}^{(k)} = \frac{\exp(e_{ij}^{(k)})}{\sum_{n=1}^N \exp(e_{in}^{(k)})} \quad (5)$$

In general, the attention probability  $\alpha_{ij}^{(k)}$  determines the amount of contribution of the  $j$ th token of  $k$ -context in the generation of the  $i$ th token of the referring expression. In each decoding step  $i$ , a final summary-vector for each context  $c_i^{(k)}$  is computed by summing the encoder states  $h_j^{(k)}$  weighted by the attention probabilities  $\alpha_{ij}^{(k)}$ :

$$c_i^{(k)} = \sum_{j=1}^N \alpha_{ij}^{(k)} h_j^{(k)} \quad (6)$$

To combine  $c_i^{(pre)}$  and  $c_i^{(pos)}$  into a single representation, this model simply concatenate the pre- and pos-context summary vectors  $c_i = [c_i^{(pre)}, c_i^{(pos)}]$ .

**HierAtt** implements a second attention mechanism inspired by Libovický and Helcl (2017) in order to generate attention weights for the pre- and pos-context summary-vectors  $c_i^{(pre)}$  and  $c_i^{(pos)}$  instead of concatenate them. Equations 7, 8 and 9 depict the process, being the projection matrices

$W_b^{(k)}$  and  $U_b^{(k)}$  as well as attention vectors  $v_b^{(k)}$  trained parameters ( $k \in [pre, pos]$ ).

$$e_i^{(k)} = v_b^{(k)T} \tanh(W_b^{(k)} s_{i-1} + U_b^{(k)} c_i^{(k)}) \quad (7)$$

$$\beta_i^{(k)} = \frac{\exp(e_i^{(k)})}{\sum_n \exp(e_i^{(n)})} \quad (8)$$

$$c_i = \sum_k \beta_i^{(k)} U_b^{(k)} c_i^{(k)} \quad (9)$$

**Decoding** Given the summary-vector  $c_i$ , the embedding of the previous referring expression token  $V_{y_{i-1}}$ , the previous decoder state  $s_{i-1}$  and the entity-embedding  $V_{wiki}$ , the decoders predict their next state which later is used to compute a probability distribution over the tokens in the output vocabulary for the next timestep as Equations 10 and 11 show.

$$s_i = \Phi_{\text{dec}}(s_{i-1}, [c_i, V_{y_{i-1}}, V_{wiki}]) \quad (10)$$

$$p(y_i | y_{<i}, X^{(pre)}, x^{(wiki)}, X^{(pos)}) = \text{softmax}(W_c s_i + b) \quad (11)$$

In Equation 10,  $s_0$  and  $c_0$  are zero-initialized vectors. In order to find the referring expression  $y$  that maximizes the likelihood in Equation 11, we apply a beam search with length normalization with  $\alpha = 0.6$  (Wu et al., 2016):

$$lp(y) = \frac{(5 + |y|)^\alpha}{(5 + 1)^\alpha} \quad (12)$$

The decoder is trained to minimize the negative log likelihood of the next token in the target referring expression:

$$J(\theta) = - \sum_i \log p(y_i | y_{<i}, X^{(pre)}, x^{(wiki)}, X^{(pos)}) \quad (13)$$

## 5 Models for Comparison

We compared the performance of NeuralREG against two baselines: *OnlyNames* and a model based on the choice of referential form method of Castro Ferreira et al. (2016), dubbed *Ferreira*.

**OnlyNames** is motivated by the similarity among the Wikipedia ID of an element and a proper name reference to it. This method refers to each entity by their Wikipedia ID, replacing each underscore in the ID for whitespaces (e.g., *Appleton International Airport* to “*Appleton International Airport*”).

**Ferreira** works by first choosing whether a reference should be a proper name, pronoun, description or demonstrative. The choice is made by a Naive Bayes method as Equation 14 depicts.

$$P(f | X) \propto \frac{P(f) \prod_{x \in X} P(x | f)}{\sum_{f' \in F} P(f') \prod_{x \in X} P(x | f')} \quad (14)$$

The method calculates the likelihood of each referential form  $f$  given a set of features  $X$ , consisting of grammatical position and information status (new or given in the text and sentence). Once the choice of referential form is made, the most frequent variant is chosen in the training corpus given the referent, syntactic position and information status. In case a referring expression for a wiki target is not found in this way, a back-off method is applied by removing one factor at a time in the following order: sentence information status, text information status and grammatical position. Finally, if a referring expression is not found in the training set for a given entity, the same method as *OnlyNames* is used. Regarding the features, syntactic position distinguishes whether a reference is the subject, object or subject determiner (genitive) in a sentence. Text and sentence information statuses mark whether a reference is a initial or a subsequent mention to an entity in the text and the sentence, respectively. All features were extracted automatically from the texts using the sentence tokenizer and dependency parser of Stanford CoreNLP (Manning et al., 2014).

## 6 Automatic evaluation

**Data** We evaluated our models on the training, development and test referring expression sets described in Section 3.3.

**Metrics** We compared the referring expressions produced by the evaluated models with the gold-standard ones using accuracy and String Edit Distance (Levenshtein, 1966). Since pronouns are highlighted as the most likely referential form to be used when a referent is salient in the discourse, as argued in the introduction, we also computed pronoun accuracy, precision, recall and F1-score in order to evaluate the performance of the models for capturing discourse salience. Finally, we lexicalized the original templates with the referring expressions produced by the models and compared them with the original texts in the corpus using accuracy and BLEU score (Papineni et al.,

2002) as a measure of fluency. Since our model does not handle referring expressions for constants (dates and numbers), we just copied their source version into the template.

Post-hoc McNemar’s and Wilcoxon signed ranked tests adjusted by the Bonferroni method were used to test the statistical significance of the models in terms of accuracy and string edit distance, respectively. To test the statistical significance of the BLEU scores of the models, we used a bootstrap resampling together with an approximate randomization method (?)<sup>2</sup>.

**Settings** NeuralREG was implemented using Dynet (Neubig et al., 2017). Source and target word embeddings were 300D each and trained jointly with the model, whereas hidden units were 512D for each direction, totaling 1024D in the bidirection layers. All non-recurrent matrices were initialized following the method of Glorot and Bengio (2010). Models were trained using stochastic gradient descent with Adadelta (Zeiler, 2012) and mini-batches of size 40. We ran each model for 60 epochs, applying early stopping for model selection based on accuracy on the development set with patience of 20 epochs. For each decoding version (Seq2Seq, CAtt and HierAtt), we searched for the best combination of drop-out probability of 0.2 or 0.3 in both the encoding and decoding layers, using beam search with a size of 1 or 5 with predictions up to 30 tokens or until 2 ending tokens were predicted (EOS). The results described in the next section were obtained on the test set by the NeuralREG version with the highest accuracy on the development set over the epochs.

**Results** Table 1 summarizes the results for all models on all metrics on the test set and Table 2 depicts a text example lexicalized by each model. The first thing to note in the results of the first table is that the baselines in the top two rows performed quite strong on this task, generating more than half of the referring expressions exactly as in the gold-standard. The method based on Castro Ferreira et al. (2016) performed statistically better than *OnlyNames* on all metrics due to its capability, albeit to a limited extent, to predict pronominal references (which *OnlyNames* obviously cannot).

We reported results on the test set for NeuralREG+Seq2Seq and NeuralREG+CAtt using

<sup>2</sup><https://github.com/jhclark/multeval>

|                   | All References      |                     | Pronouns          |       |      |         | Text                |                      |
|-------------------|---------------------|---------------------|-------------------|-------|------|---------|---------------------|----------------------|
|                   | Acc.                | SED                 | Acc.              | Prec. | Rec. | F-Score | Acc.                | BLEU                 |
| <i>OnlyNames</i>  | 0.53 <sup>D</sup>   | 4.05 <sup>D</sup>   | -                 | -     | -    | -       | 0.15 <sup>D</sup>   | 69.03 <sup>D</sup>   |
| <i>Ferreira</i>   | 0.61 <sup>C</sup>   | 3.18 <sup>C</sup>   | 0.43 <sup>B</sup> | 0.57  | 0.54 | 0.55    | 0.19 <sup>C</sup>   | 72.78 <sup>C</sup>   |
| NeuralREG+Seq2Seq | 0.74 <sup>A,B</sup> | 2.32 <sup>A,B</sup> | 0.75 <sup>A</sup> | 0.77  | 0.78 | 0.78    | 0.28 <sup>B</sup>   | 79.27 <sup>A,B</sup> |
| NeuralREG+CAtt    | 0.74 <sup>A</sup>   | 2.25 <sup>A</sup>   | 0.75 <sup>A</sup> | 0.73  | 0.78 | 0.75    | 0.30 <sup>A</sup>   | 79.39 <sup>A</sup>   |
| NeuralREG+HierAtt | 0.73 <sup>B</sup>   | 2.36 <sup>B</sup>   | 0.73 <sup>A</sup> | 0.74  | 0.77 | 0.75    | 0.28 <sup>A,B</sup> | 79.01 <sup>B</sup>   |

Table 1: (1) Accuracy (Acc.) and String Edit Distance (SED) results in the prediction of all referring expressions; (2) Accuracy (Acc.), Precision (Prec.), Recall (Rec.) and F-Score results in the prediction of pronominal forms; and (3) Accuracy (Acc.) and BLEU score results of the texts with the generated referring expressions. Rankings were determined by statistical significance.

dropout probability 0.3 and beam size 5, and NeuralREG+HierAtt with dropout probability of 0.3 and beam size of 1 selected based on the highest accuracy on the development set. Importantly, the three NeuralREG variant models statistically outperformed the two baseline systems. They achieved BLEU scores, text and referential accuracies as well as string edit distances in the range of 79.01-79.39, 28%-30%, 73%-74% and 2.25-2.36, respectively. This means that NeuralREG predicted 3 out of 4 references completely correct, whereas the incorrect ones needed an average of 2 post-edition operations in character level to be equal to the gold-standard. When considering the texts lexicalized with the referring expressions produced by NeuralREG, at least 28% of them are similar to the original texts. Especially noteworthy was the score on pronoun accuracy, indicating that the model was well capable of predicting when to generate a pronominal reference in our dataset.

The results for the different decoding methods for NeuralREG were similar, with the NeuralREG+CAtt performing slightly better in terms of the BLEU score, text accuracy and String Edit Distance. The more complex NeuralREG+HierAtt yielded the lowest results, even though the differences with the other two models were small and not even statistically significant in many of the cases.

## 7 Human Evaluation

Complementary to the automatic evaluation, we performed an evaluation with human judges, comparing the quality judgments of the original texts to the versions generated by our various models.

**Material** We quasi-randomly selected 24 instances from the delexicalized version of the WebNLG corpus related to the test part of the re-

ferring expression collection. For each of the selected instances, we took into account its source triple set and its 6 target texts: one original (randomly chosen) and its versions with the referring expressions generated by each of the 5 models introduced in this study (two baselines, three neural models). Instances were chosen following 2 criteria: the number of triples in the source set (ranging from 2 to 7) and the differences between the target texts.

For each size group, we randomly selected 4 instances (of varying degrees of variation between the generated texts) giving rise to 144 trials (= 6 triple set sizes \* 4 instances \* 6 text versions), each consisting of a set of triples and a target text describing it with the lexicalized referring expressions highlighted in yellow.

**Method** The experiment had a latin-square design, distributing the 144 trials over 6 different lists such that each participant rated 24 trials, one for each of the 24 corpus instances, making sure that participants saw equal numbers of triple set sizes and generated versions. Once introduced to a trial, the participants were asked to rate the fluency (“does the text flow in a natural, easy to read manner?”), grammaticality (“is the text grammatical (no spelling or grammatical errors)?”) and clarity (“does the text clearly express the data?”) of each target text on a 7-Likert scale, focussing on the highlighted referring expressions. The experiment is available on the website of the author<sup>3</sup>.

**Participants** We recruited 60 participants, 10 per list, via Mechanical Turk. Their average age was 36 years and 27 of them were females. The majority declared themselves native speakers of

<sup>3</sup><https://ilk.uvt.nl/~tcastrof/acl2018/evaluation/>

| Model            | Text                                                                                                                                                                                                                                   |
|------------------|----------------------------------------------------------------------------------------------------------------------------------------------------------------------------------------------------------------------------------------|
| <i>OnlyNames</i> | alan shepard was born in new hampshire on 1923-11-18 . before alan shepard death in california alan shepard had been awarded distinguished service medal (united states navy) an award higher than department of commerce gold medal . |
| <i>Ferreira</i>  | alan shepard was born in new hampshire on 1923-11-18 . before alan shepard death in california him had been awarded distinguished service medal an award higher than department of commerce gold medal .                               |
| <i>Seq2Seq</i>   | alan shepard was born in new hampshire on 1923-11-18 . before his death in california him had been awarded the distinguished service medal by the united states navy an award higher than the department of commerce gold medal .      |
| <i>CAtt</i>      | alan shepard was born in new hampshire on 1923-11-18 . before his death in california he had been awarded the distinguished service medal by the us navy an award higher than the department of commerce gold medal .                  |
| <i>HierAtt</i>   | alan shephard was born in new hampshire on 1923-11-18 . before his death in california he had been awarded the distinguished service medal an award higher than the department of commerce gold medal .                                |
| <i>Original</i>  | alan shepard was born in new hampshire on 18 november 1923 . before his death in california he had been awarded the distinguished service medal by the us navy an award higher than the department of commerce gold medal .            |

Table 2: Example of text with references lexicalized by each model.

|                   | Fluency             | Grammar             | Clarity             |
|-------------------|---------------------|---------------------|---------------------|
| <i>OnlyNames</i>  | 4.74 <sup>C</sup>   | 4.68 <sup>B</sup>   | 4.90 <sup>B</sup>   |
| <i>Ferreira</i>   | 4.74 <sup>C</sup>   | 4.58 <sup>B</sup>   | 4.93 <sup>B</sup>   |
| NeuralREG+Seq2Seq | 4.95 <sup>B,C</sup> | 4.82 <sup>A,B</sup> | 4.97 <sup>B</sup>   |
| NeuralREG+CAtt    | 5.23 <sup>A,B</sup> | 4.95 <sup>A,B</sup> | 5.26 <sup>A,B</sup> |
| NeuralREG+HierAtt | 5.07 <sup>B,C</sup> | 4.90 <sup>A,B</sup> | 5.13 <sup>A,B</sup> |
| <i>Original</i>   | 5.41 <sup>A</sup>   | 5.17 <sup>A</sup>   | 5.42 <sup>A</sup>   |

Table 3: Fluency, Grammaticality and Clarity results obtained in the human evaluation. Rankings were determined by statistical significance.

English (44), while 14 and 2 self-reported as fluent or having a basic proficiency, respectively.

**Results** Table 3 summarizes the results. Inspection of the Table reveals a clear pattern: all three neural models scored higher than the baselines on all metrics, with especially NeuralREG+CAtt approaching the ratings for the original sentences, although – again – differences between the neural models were small. Concerning the size of the triple sets, we did not find any clear pattern.

To test the statistical significance of the pairwise comparisons, we used the Wilcoxon signed-rank test corrected for multiple comparisons using the Bonferroni method. Different from the automatic evaluation, the results of both baselines were not statistically significant for the three metrics. In comparison with the neural models, NeuralREG+CAtt significantly outperformed the baselines in terms of fluency, whereas the other comparisons between baselines and neural models were not statistically significant. The results for

the 3 different decoding methods of NeuralREG also did not reveal a significant difference. Finally, the original texts were rated significantly higher than both baselines in terms of the three metrics, also than NeuralREG+Seq2Seq and NeuralREG+HierAtt in terms of fluency, and than NeuralREG+Seq2Seq in terms of clarity.

## 8 Discussion

This study introduced NeuralREG, an end-to-end approach based on neural networks which tackles the full Referring Expression Generation process. It generates referring expressions for discourse entities by simultaneously selecting form and content without any need of feature extraction techniques. The model was implemented using an encoder-decoder approach where a target referent and its surrounding linguistic contexts were first encoded and combined into a single vector representation which subsequently was decoded into a referring expression to the target, suitable for the specific discourse context. In an automatic evaluation on a collection of 78,901 referring expressions to 1,501 Wikipedia entities, the different versions of the model all yielded better results than the two (competitive) baselines. Later in a complementary human evaluation, the texts with referring expressions generated by a variant of our novel model were considered statistically more fluent than the texts lexicalized by the two baselines.

**Data** The collection of referring expressions used in our experiments was extracted from a novel, delexicalized and publicly available version



of the WebNLG corpus (Gardent et al., 2017a,b), where the discourse entities were replaced with general tags for decreasing the data sparsity. Besides the REG task, these data can be useful for many other tasks related to, for instance, the NLG process (Reiter and Dale, 2000; Gatt and Krahmer, 2017) and Wikification (Moussallem et al., 2017).

**Baselines** We introduced two strong baselines which generated roughly half of the referring expressions identical to the gold standard in an automatic evaluation. These baselines performed relatively well because they frequently generated full names, which occur often for our wikified references. However, they performed poorly when it came to pronominalization, which is an important ingredient for fluent, coherent text. *OnlyNames*, as the name already reveals, does not manage to generate any pronouns. However, the approach of Castro Ferreira et al. (2016) also did not perform well in the generation of pronouns, revealing a poor capacity to detect highly salient entities in a text.

**NeuralREG** was implemented with 3 different decoding architectures: Seq2Seq, CAtt and HierAtt. Although all the versions performed relatively similar, the concatenative-attention (CAtt) version generated the closest referring expressions from the gold-standard ones and presented the highest textual accuracy in the automatic evaluation. The texts lexicalized by this variant were also considered statistically more fluent than the ones generated by the two proposed baselines in the human evaluation.

Surprisingly, the most complex variant (HierAtt) with a hierarchical-attention mechanism gave lower results than CAtt, producing lexicalized texts which were rated as less fluent than the original ones and not significantly more fluent from the ones generated by the baselines. This result appears to be not consistent with the findings of Libovický and Helcl (2017), who reported better results on multi-modal machine translation with hierarchical-attention as opposed to the flat variants (Specia et al., 2016).

Finally, our NeuralREG variant with the lowest results were our ‘vanilla’ sequence-to-sequence (Seq2Seq), whose the lexicalized texts were significantly less fluent and clear than the original ones. This shows the importance of the attention mechanism in the decoding step of NeuralREG

in order to generate fine-grained referring expressions in discourse.

**Conclusion** We introduced a deep learning model for the generation of referring expressions in discourse texts. NeuralREG decides both on referential form and on referential content in an integrated, end-to-end approach, without using explicit features. Using a new delexicalized version of the WebNLG corpus (made publicly available), we showed that the neural model substantially improves over two strong baselines in terms of accuracy of the referring expressions and fluency of the lexicalized texts.

## Acknowledgments

This work has been supported by the National Council of Scientific and Technological Development from Brazil (CNPq) under the grants 203065/2014-0 and 206971/2014-1.

## References

- Dzmitry Bahdanau, Kyunghyun Cho, and Yoshua Bengio. 2014. Neural machine translation by jointly learning to align and translate. *arXiv preprint arXiv:1409.0473*.
- Anja Belz, Eric Kow, Jette Viethen, and Albert Gatt. 2010. Empirical methods in natural language generation. Springer-Verlag, Berlin, Heidelberg, chapter Generating Referring Expressions in Context: The GREC Task Evaluation Challenges, pages 294–327.
- Charles B. Callaway and James C. Lester. 2002. Pronominalization in generated discourse and dialogue. In *Proceedings of the 40th Annual Meeting on Association for Computational Linguistics*. Association for Computational Linguistics, Stroudsburg, PA, USA, ACL ’02, pages 88–95.
- Thiago Castro Ferreira, Iacer Calixto, Sander Wubben, and Emiel Krahmer. 2017a. Linguistic realisation as machine translation: Comparing different mt models for amr-to-text generation. Association for Computational Linguistics, pages 1–10.
- Thiago Castro Ferreira, Emiel Krahmer, and Sander Wubben. 2016. Towards more variation in text generation: Developing and evaluating variation models for choice of referential form. In *Proceedings of the 54th Annual Meeting of the Association for Computational Linguistics (Volume 1: Long Papers)*. Association for Computational Linguistics, pages 568–577.
- Thiago Castro Ferreira, Emiel Krahmer, and Sander Wubben. 2017b. Generating flexible proper name references in text: Data, models and evaluation. In

- Proceedings of the 15th Conference of the European Chapter of the Association for Computational Linguistics: Volume 1, Long Papers*. Association for Computational Linguistics, pages 655–664.
- Robert Dale and Nicholas Haddock. 1991. Generating referring expressions involving relations. In *Proceedings of the fifth conference on European chapter of the Association for Computational Linguistics*. Association for Computational Linguistics, Stroudsburg, PA, USA, EACL '91, pages 161–166.
- Robert Dale and Ehud Reiter. 1995. Computational interpretations of the gricean maxims in the generation of referring expressions. *Cognitive science* 19(2):233–263.
- Claire Gardent, Anastasia Shimorina, Shashi Narayan, and Laura Perez-Beltrachini. 2017a. Creating training corpora for nlg micro-planners. In *Proceedings of the 55th Annual Meeting of the Association for Computational Linguistics (Volume 1: Long Papers)*. Association for Computational Linguistics, pages 179–188.
- Claire Gardent, Anastasia Shimorina, Shashi Narayan, and Laura Perez-Beltrachini. 2017b. The webnlg challenge: Generating text from rdf data. Association for Computational Linguistics, pages 124–133.
- Albert Gatt and Emiel Krahmer. 2017. Survey of the state of the art in natural language generation: Core tasks, applications and evaluation. *arXiv preprint arXiv:1703.09902*.
- Xavier Glorot and Yoshua Bengio. 2010. Understanding the difficulty of training deep feedforward neural networks. In Yee Whye Teh and Mike Titterton, editors, *Proceedings of the Thirteenth International Conference on Artificial Intelligence and Statistics*. PMLR, Chia Laguna Resort, Sardinia, Italy, volume 9 of *Proceedings of Machine Learning Research*, pages 249–256.
- Barbara J. Grosz, Scott Weinstein, and Aravind K. Joshi. 1995. Centering: A framework for modeling the local coherence of discourse. *Computational Linguistics* 21(2).
- Jeanette K. Gundel, Nancy Hedberg, and Ron Zacharski. 1993. Cognitive status and the form of referring expressions in discourse. *Language* 69(2):274–307.
- Renate Henschel, Hua Cheng, and Massimo Poesio. 2000. Pronominalization revisited. In *Proceedings of the 18th conference on Computational linguistics-Volume 1*. Association for Computational Linguistics, pages 306–312.
- Sepp Hochreiter and Jürgen Schmidhuber. 1997. Long short-term memory. *Neural computation* 9(8):1735–1780.
- T Florian Jaeger. 2010. Redundancy and reduction: Speakers manage syntactic information density. *Cognitive psychology* 61(1):23–62.
- I. Konstas, S. Iyer, M. Yatskar, Y. Choi, and L. Zettlemoyer. 2017. Neural AMR: Sequence-to-Sequence Models for Parsing and Generation. *ArXiv e-prints*.
- Emiel Krahmer and Kees van Deemter. 2012. Computational generation of referring expressions: A survey. *Computational Linguistics* 38(1):173–218.
- Rémi Lebret, David Grangier, and Michael Auli. 2016. Neural text generation from structured data with application to the biography domain. In *Proceedings of the 2016 Conference on Empirical Methods in Natural Language Processing*. Association for Computational Linguistics, pages 1203–1213.
- V. I. Levenshtein. 1966. Binary Codes Capable of Correcting Deletions, Insertions and Reversals. *Soviet Physics Doklady* 10:707.
- Jindřich Libovický and Jindřich Helcl. 2017. Attention strategies for multi-source sequence-to-sequence learning. *arXiv preprint arXiv:1704.06567*.
- Christopher D. Manning, Mihai Surdeanu, John Bauer, Jenny Finkel, Steven J. Bethard, and David McClosky. 2014. The Stanford CoreNLP natural language processing toolkit. In *Association for Computational Linguistics (ACL) System Demonstrations*. pages 55–60.
- D. Moussallem, R. Usbeck, M. Röder, and A.-C. Ngonga Ngomo. 2017. MAG: A Multilingual, Knowledge-base Agnostic and Deterministic Entity Linking Approach. *ArXiv e-prints*.
- G. Neubig, C. Dyer, Y. Goldberg, A. Matthews, W. Ammar, A. Anastasopoulos, M. Ballesteros, D. Chiang, D. Clothiaux, T. Cohn, K. Duh, M. Faruqui, C. Gan, D. Garrette, Y. Ji, L. Kong, A. Kuncoro, G. Kumar, C. Malaviya, P. Michel, Y. Oda, M. Richardson, N. Saphra, S. Swayamdipta, and P. Yin. 2017. DyNet: The Dynamic Neural Network Toolkit. *ArXiv e-prints*.
- Naho Orita, Eliana Vornov, Naomi Feldman, and Hal Daumé III. 2015. Why discourse affects speakers’ choice of referring expressions. In *Proceedings of the 53rd Annual Meeting of the Association for Computational Linguistics and the 7th International Joint Conference on Natural Language Processing (Volume 1: Long Papers)*. Association for Computational Linguistics, pages 1639–1649.
- Kishore Papineni, Salim Roukos, Todd Ward, and Wei-Jing Zhu. 2002. Bleu: a method for automatic evaluation of machine translation. In *Proceedings of 40th Annual Meeting of the Association for Computational Linguistics*. Association for Computational Linguistics, Philadelphia, Pennsylvania, USA, pages 311–318.
- Ehud Reiter and Robert Dale. 2000. *Building natural language generation systems*. Cambridge University Press, New York, NY, USA.

- Mike Schuster and Kuldip K Paliwal. 1997. Bidirectional recurrent neural networks. *IEEE Transactions on Signal Processing* 45(11):2673–2681.
- Advaith Siddharthan, Ani Nenkova, and Kathleen McKeown. 2011. Information status distinctions and referring expressions: An empirical study of references to people in news summaries. *Computational Linguistics* 37(4):811–842.
- Lucia Specia, Stella Frank, Khalil Sima'an, and Desmond Elliott. 2016. A shared task on multi-modal machine translation and crosslingual image description. In *WMT*, pages 543–553.
- Kees van Deemter. 2016. Designing algorithms for referring with proper names. Association for Computational Linguistics, pages 31–35.
- Yonghui Wu, Mike Schuster, Zhifeng Chen, Quoc V. Le, Mohammad Norouzi, Wolfgang Macherey, Maxim Krikun, Yuan Cao, Qin Gao, Klaus Macherey, Jeff Klingner, Apurva Shah, Melvin Johnson, Xiaobing Liu, Łukasz Kaiser, Stephan Gouws, Yoshikiyo Kato, Taku Kudo, Hideto Kazawa, Keith Stevens, George Kurian, Nishant Patil, Wei Wang, Cliff Young, Jason Smith, Jason Riesa, Alex Rudnick, Oriol Vinyals, Greg Corrado, Macduff Hughes, and Jeffrey Dean. 2016. Google’s neural machine translation system: Bridging the gap between human and machine translation. *CoRR* abs/1609.08144.
- Matthew D. Zeiler. 2012. ADADELTA: An Adaptive Learning Rate Method. *CoRR* abs/1212.5701.
- Xingxing Zhang and Mirella Lapata. 2014. Chinese poetry generation with recurrent neural networks. In *Proceedings of the 2014 Conference on Empirical Methods in Natural Language Processing (EMNLP)*. Association for Computational Linguistics, pages 670–680.
