# Supplementary material for: Knowledge Graphs for Multilingual Language Translation and Generation
Source: arXiv:2009.07715 source file (2020-09-16)
Supplement: Supplementary file 8 [file RDF2PT.pdf]

# RDF2PT: Generating Brazilian Portuguese Texts from RDF Data

Diego Moussallem<sup>1,2</sup>, Thiago Castro Ferreira<sup>2</sup>, Marcos Zampieri<sup>3</sup>,  
Maria Claudia Cavalcanti<sup>4</sup>, Geraldo Xexéo<sup>5</sup>, Mariana Neves<sup>6</sup>, Axel-Cyrille Ngonga Ngomo<sup>1,7</sup>

<sup>1</sup>University of Leipzig - Germany, <sup>2</sup>Tilburg University - The Netherlands,

<sup>3</sup>University of Wolverhampton - United Kingdom, <sup>4</sup>Military Institute of Engineering - Brazil,

<sup>5</sup>Federal University of Rio de Janeiro - Brazil, <sup>6</sup>German Federal Institute for Risk Assessment - Germany

<sup>7</sup>Paderborn University - Germany

<sup>1</sup>lastname@informatik.uni-leipzig.de

## Abstract

The generation of natural language from Resource Description Framework (RDF) data has recently gained significant attention due to the continuous growth of Linked Data. A number of these approaches generate natural language in languages other than English, however, no work has been proposed to generate Brazilian Portuguese texts out of RDF. We address this research gap by presenting RDF2PT, an approach that verbalizes RDF data to Brazilian Portuguese language. We evaluated RDF2PT in an open questionnaire with 44 native speakers divided into experts and non-experts. Our results suggest that RDF2PT is able to generate text which is similar to that generated by humans and can hence be easily understood.

**Keywords:** natural language generation, verbalization, semantic web

## 1. Introduction

Natural Language Generation (NLG) is the process of generating coherent natural language text from non-linguistic data (Reiter and Dale, 2000). Despite community agreement on the actual text and speech output of these systems, there is far less consensus on what the input should be (Gatt and Krahmer, 2017). A large number of inputs have been taken for NLG systems, including images (Xu et al., 2015), numeric data (Gkatzia et al., 2014), semantic representations (Theune et al., 2001) and Semantic Web (SW) data (Ngonga Ngomo et al., 2013; Bouayad-Agha et al., 2014).

Presently, the generation of natural language from SW, more precisely from RDF data, has gained substantial attention (Bouayad-Agha et al., 2014; Staykova, 2014). Some challenges have been proposed to investigate the quality of automatically generated texts from RDF (Colin et al., 2016). Moreover, RDF has demonstrated a promising ability to support the creation of NLG benchmarks (Gardent et al., 2017). However, English is the only language which has been widely targeted. Even though there are studies which explore the generation of content in languages other than English, to the best of our knowledge, no work has been proposed to generate texts in Brazilian Portuguese from RDF data.

In this paper, we propose RDF2PT, a rule-based approach to verbalize RDF data to Brazilian Portuguese. While the exciting avenue of using deep learning techniques in NLG approaches (Gatt and Krahmer, 2017) is open to this task and deep learning has already shown promising results for RDF data (Sleimi and Gardent, 2016), the morphological richness of Portuguese led us to develop a rule-based approach. This was to ensure that we could identify the challenges imposed by this language from the SW perspective before applying Machine Learning (ML) algorithms.

RDF2PT is able to generate either a single sentence or a summary of a given resource. In order to validate our

approach, we evaluated RDF2PT using experts in Natural Language Processing (NLP) and SW as well as non-experts who are lay users or non-users of SW technologies. Both groups are native speakers of Brazilian Portuguese. The results suggest that RDF2PT generates texts which can be easily understood by humans and also help to identify some of the challenges related to the automatic generation of Brazilian Portuguese (especially from RDF). The version of RDF2PT used in this paper, all experimental results and the texts generated for the experiments are publicly available.<sup>1</sup>

## 2. Related Work

According to Staykova (2014) and Bouayad-Agha et al. (2014), there has been a plenty of works which investigated the generation of Natural Language (NL) texts from Semantic Web Technologies (SWT) as an input data. However, the subject of research has only recently gained significant momentum. This attention comes from the great number of published works such as (Cimiano et al., 2013; Duma and Klein, 2013; Ell and Harth, 2014; Biran and McKeown, 2015) which used RDF as an input data and achieved promising results. Also, the works published in the WebNLG (Colin et al., 2016) challenge, which used deep learning techniques such as (Sleimi and Gardent, 2016; Mrabet et al., 2016), also contributed to this interest. RDF has also been showing promising benefits to the generation of benchmarks for evaluating NLG systems (Gardent et al., 2017; Perez-Beltrachini et al., 2016; Mohammed et al., 2016; Schwitter et al., 2004; Hewlett et al., 2005; Sun and Mellish, 2006).

Despite the plethora of works written on handling SWT data, only a few have exploited the generation of languages other than English, for instance, Keet and Khumalo (2017) to Zulu language. Additionally, a considerable number of NLG approaches can be found to European or Brazilian

<sup>1</sup><https://github.com/dice-group/RDF2PT>

Portuguese languages (Pereira and Paraboni, 2008; Cuevas and Paraboni, 2008; de Novais et al., 2009; de Novais et al., 2010; de Novais et al., 2012; de Novais and Paraboni, 2013; De Oliveira and Sripada, 2014; Pereira et al., 2015), however, none of them have exploited the generation of NL from RDF. Therefore, to the best of our knowledge, RDF2PT is the first proposed approach to this end.

### 3. The RDF2PT approach

In this section, we first give a brief description of how RDF data is able to represent useful linguistic information and we detail our approach RDF2PT in a sequence.

#### 3.1. Preliminary RDF concepts

Although previous works such as Sun and Mellish (2006) have already introduced how a single RDF statement contains linguistic information, we briefly explain the concept for a better understanding of RDF2PT.

RDF (RDF Working Group, 25 February 2014) statements are based on graph data models for representing knowledge. Thus, an RDF graph is a set of facts. Facts are expressed as so-called triples in the form (subject predicate object). The *subjects* and *predicates* are Internationalized Resource Identifiers (IRI)s and *objects* are either IRIs or literals. Literals, in general, have a datatype that defines its kind of values. For example, a literal can be a date, a number, a measure, a word or a group of words. On the other hand, a predicate denotes a binary relation between the *subject* and *object* as an argument. Additionally, RDF vocabulary comprises some built-in properties. The most common one is `rdf:type`, which states that a resource denoted by the subject is an instance of the class specified by the object of the triple. For example, the Listing 1 shows a fragment of Albert Einstein DBpedia’s resource<sup>2</sup> which represents the following information: “*Albert Einstein was a scientist who worked in physics area. He was born in Ulm and died in Princeton.*”.

```
:Albert_Einstein rdf:type dbo:Scientist
:Albert_Einstein dbo:field :Physics
:Albert_Einstein dbo:birthPlace :Ulm
:Albert_Einstein dbo:deathPlace :Princeton
```

Listing 1: An excerpt of RDF triples.

#### 3.2. Approach

RDF2PT approach is akin to the approach SPARQL2NL (Ngonga Ngomo et al., 2013) from which the project SemWeb2NL<sup>3</sup> originated. SemWeb2NL comprises rule-based and template-based approaches which aim to verbalize texts and concepts not only from RDF triples but also from ontologies and SPARQL queries into English. In addition, SemWeb2NL is able to produce automatically educational Question Answering (QA) systems for self-assessment (Bühmann et al., 2015). Despite the RDF2PT approach being capable of generating single sentences from distinct RDF triples, for the sake of space,

our description focuses on how RDF2PT can output a simplified summary of a given resource.

A generic NLG pipeline is composed by three tasks which are *Document Planning*, *Micro Planning* and *Realization*. RDF2PT operates mostly at the level of the first two and to the *Realization* task, RDF2PT uses an adaption of SimpleNLG to Brazilian Portuguese (De Oliveira and Sripada, 2014).

In the following sections, we describe the RDF2PT steps according to an NLG system pipeline (Gatt and Krahmer, 2017). We then use the Portuguese version of DBpedia as a Knowledge Base (KB) (Auer et al., 2007; Lehmann et al., 2015) and as source for our examples.

#### 3.3. Document Planning

This initial phase is divided into two sub-tasks. First, *Content determination*, which is responsible for deciding what information a certain NLG system should include in the generated text. Second, *Discourse planning* (also known as Text structuring), which determines the order of the information in paragraphs and its rhetorical relation.

**Content determination** RDF2PT assumes the description of a resource to be the set of RDF statements of which this resource is the subject. Hence, given a resource, RDF2PT first performs a SPARQL query to get its most specific class through the predicate `rdf:type`. Afterward, RDF2PT gets all resources which belong to this specific class and ranks their predicates by using Page Rank (Page et al., 1999) over the KB. By these means, our approach can determine the most popular facts of this specific class.<sup>4</sup> Once the predicates are ranked, RDF2PT considers only the top seven most popular predicates of the class to describe the input resource.<sup>5</sup> For example, given `dbp:Albert_Einstein` as a resource, RDF2PT determines its most specific class to be `dbo:Scientist`. Then, it ranks all the predicates used by this class per popularity according to its resources (see Listing 2).

```
rdf:type                dbo:field
dbo:deathPlace          dbo:almaMater
dbo:knownFor            dbo:award
dbo:doctoralStudent
```

Listing 2: Most popular predicates of a scientist.

**Discourse planning** In this step, RDF2PT clusters and orders the triples. The subjects are ordered with respect to the number of their occurrences, thus assigning them to those input triples that mention them. RDF2PT processes the input in descending order with respect to the frequency of the variables they contain, starting with the projection variables and only after that, turning to other variables. This method has already been used by other approaches and is the most effective method to follow regarding rule-based approaches to RDF (Bouayad-Agha et al., 2014). As an example, consider the following triples in Listing 3.

```
:Albert_Einstein  dbo:deathPlace :Princeton.
:Princeton        dbo:Country    :USA.
```

<sup>2</sup>[http://dbpedia.org/resource/Albert\\_Einstein](http://dbpedia.org/resource/Albert_Einstein)

<sup>3</sup><https://github.com/AKSW/SemWeb2NL>

<sup>4</sup>The predicates can vary according to the classes and KB

<sup>5</sup>This choice was based on Gardent et al. (2017) which states that seven triples is a reasonable number for describing a resource.

```
:Albert_Einstein rdf:type :Scientist.
:Albert_Einstein dbo:knownFor :General_relativity.
:Albert_Einstein dbo:knownFor :Brownian_motion.
:Albert_Einstein dbo:birthPlace :Ulm.
:Ulm rdf:type :City.
:Ulm dbo:Country :Germany.
```

Listing 3: Example of triples before planning

Listing 3 presents three subjects, `:Albert_Einstein`, `:Ulm` and `:Princeton`. As `:Albert_Einstein` is assigned to more triples than the others, it takes the first place in the discourse, followed by `:Ulm`, `:Princeton` respectively (see Listing 4). However, RDF2PT still considers the popularity of predicates from the previous steps and organizes triples based on it, for instance, `rdf:type` comes before others due to its frequency in the KB.

```
:Albert_Einstein rdf:type :Scientist
:Albert_Einstein dbo:birthPlace :Ulm
:Albert_Einstein dbo:deathPlace :Princeton
:Albert_Einstein dbo:knownFor :General_relativity.
:Albert_Einstein dbo:knownFor :Brownian_motion.
:Ulm rdf:type :City
:Ulm dbo:Country :Germany
:Princeton dbo:Country :USA
```

Listing 4: Example of triples after planning

### 3.4. Micro Planning

This step is concerned with the planning of a sentence. It comprises three sub-tasks. Firstly, *Sentence aggregation* decides whether information will be presented individually or separately. Second, *Lexicalization* chooses the right words and phrases in natural language for expressing the semantics about the data. Third, *Coreference generation* (also known as *Referring expression*) is the task responsible for generating syntagms (references) to discourse entities, for example, whether the text should refer to an entity using a definite description, a pronoun or a proper noun (Ferreira et al., 2016). In the following, we describe the challenges behind the tasks entailed.

**Sentence aggregation** This task is based on Ngonga Ngomo et al. (2013). It is divided into two phases, *subject grouping* and *object grouping*. *Subject grouping* collapses the predicates and objects of two triples if their subjects are the same. *Object grouping* collapses the subjects of two triples if the predicates and objects of the triples are the same.

The common elements are usually subject noun phrases and verb phrases (verbs together with object noun phrases). In order to maximize the grouping effects, we additionally collapse common prefixes and suffixes of triples, irrespective of whether they are full subject noun phrases or complete verb phrases.

In Listing 5, the predicate `dbo:knownFor` shares the same subject `:Albert_Einstein` and also has two objects, `:General_relativity` and `:Brownian_motion`. Additionally, the predicate `dbo:birthPlace` shares the same object `:Ulm` and has two subjects, `:Albert_Einstein` and `:Gabriel_Steiner`. They therefore can be collapsed using a conjunction AND, thus organizing and omitting repetitive triples. Moreover, we remove repetitions that arise when triples’ verbalizations lead to the same natural language representation.

```
:Albert_Einstein dbo:knownFor :General_relativity.
:Albert_Einstein dbo:knownFor :Brownian_motion.
:Albert_Einstein dbo:birthPlace :Ulm.
:Gabriel_Steiner dbo:birthPlace :Ulm.
```

Listing 5: Grouping subjects and objects

**Lexicalization** This step comprises the main contribution of RDF2PT for verbalizing the triples in Brazilian Portuguese. In contrast to English, Brazilian Portuguese is a morphologically rich language which contains the grammatical gender of words. Grammatical gender plays a key role because it affects the generation of determiners and pronouns. It also influences the inflection of nouns and verbs. For instance, the passive expression of the verb *nascer* (en: “be born”) is *nascida* if the subject is feminine or *nascido* if masculine. Thus, the gender of words is essential for comprehending the semantics of a given Portuguese text. Also, Brazilian Portuguese has different possibilities in the expression of subject possessives. Hence, RDF2PT has to deal with the following phenomena while lexicalizing:

- **Grammatical gender** - In Portuguese, the gender varies between masculine and feminine. This variation leads to supplementary challenges when lexicalizing words automatically. For example, a gender may be represented by articles “um” and “o” (masculine) or “uma” and “a” (feminine). However, the gender also affects the inflection of words. For instance, for the word “cantor” (en: “singer”), if the subject is feminine, the word becomes “cantora”. However, there are words which do not inflect, e.g., the word “gerente” (en: “manager”). If the subject is a woman, we only refer to it by using the article “a”, i.e., “a gerente”. Therefore, there are some challenges to tackle for recognizing the gender and assigning it correctly. A tricky example to solve automatically is “O Rio de Janeiro é uma cidade” (en: Rio de Janeiro is a city). In this case, the subject is masculine but its complement is feminine. Devising handcrafted rules to handle these phenomena can become a hard task. To address this challenge, we use a Part-Of-Speech tagger (TreeTagger in our case) as it retrieves the gender along with the parts of speech.<sup>6</sup> All the obtained genders are attached along with the lexicalizations for supporting the realization step.
- **Classes and resources** - The lexicalization of classes and resources is carried by using a SPARQL query to get their Portuguese labels through the `rdfs:label predicate`<sup>7</sup>. In case such a label does not exist, we use either the fragment of their URI (the string after the # character) if it exists, or the string after the last occurrence of “/”. Finally, this natural language representation is lexicalized as a noun phrase. Afterwards, RDF2PT recognizes the gender. In case the

<sup>6</sup>see the POS tags <http://www.cis.uni-muenchen.de/~schmid/tools/TreeTagger/data/Portuguese-Tagset.html>

<sup>7</sup>Note that it could be any property which returns a natural language representation of the given URI, see (Ell et al., 2011).

resource is recognized as a person, RDF2PT applies a string similarity measure (0.8 threshold) between the lexicalized word with a list of names provided by SemWeb2NL. This list is divided by masculine and feminine which in turn results in the gender. If the resource is not a person, we use Tree-tagger.

- **Properties** - The lexicalization of properties relies on one of the results of Ngonga Ngomo et al. (2013), i.e., that most property labels are either nouns or verbs. To determine which lexicalization to use automatically, we rely on the insight that the first and last words of a property label in Portuguese are commonly the key to determining the type of property. We then use the Tree-Tagger to get the part of speech of predicates. Properties whose label begins with a verb are lexicalized as verbs. For example, the predicate `dbo:knownFor`, which Portuguese label is “conhecido por”, has the first word identified as an inflection of the verb “conhecer” (en:know). Therefore, RDF2PT lexicalizes and sets it as a verb. We devised a set of rules to capture this behavior, which we omit due to space restrictions.<sup>8</sup> Moreover, RDF2PT uses some pre-defined templates for improving the quality of lexicalization. For example, the predicate `dbo:birthPlace`, RDF2PT uses the verb “nascer” (eng: be born) along with the predicate “em” (en: “in”), so this predicate can be lexicalized as “nasceu em” (en: was born in).

For predicates which are recognized as nouns, RDF2PT relies on labels. For instance, `dbo:birthDate` is labeled as “data de nascimento” and recognized as a noun phrase because of its first word “data”. RDF2PT also uses the first word of predicates to set the gender. For example, `dbo:deathPlace` is transliterated as “local de falecimento”. “local” is masculine. Hence, the determiner to be used in front of this predicate needs to be “o”. In contrast to `dbo:birthDate` (“data de nascimento”), the word “data” is feminine, thus the determiner must be “a”.

- **Literals** - In an RDF graph, literals usually consist of a *lexical form* `LF` and a *datatype IRI* `DT`. If the datatype is `rdf:langString`, a non-empty *language tag* is specified and the literal is denoted as a *language-tagged string*.<sup>9</sup> Accordingly, the lexicalization of strings with language tags is carried by using simply the lexical form, while omitting the language tag. For example, “Albert Einstein”@pt is lexicalized as “Albert Einstein” or “Alemanha”@pt (“Germany”@en) is lexicalized as “Alemanha”. For other types of literals, we differentiate between built-in<sup>10</sup> and user-defined datatypes. For built-in literals, we use the lexical form, e.g., “123”^^xsd:int ⇒ “123”. User-defined types are processed by us-

ing the literal value together with the (pluralized) natural language representation of the datatype IRI. Thus, we lexicalize “123”^^dt:squareKilometre as “123 quilômetros quadrados” (en: “123 square kilometres”).

**Coreference generation** In this step, RDF2PT relies on the number of subjects contained by the RDF statements and only uses other expressions to refer to a given subject in case there is more than one mention of it. RDF2PT replaces the subject by possessive or personal pronouns with the corresponding gender depending on the predicates. For instance, given a triple `dbr: Albert_Einstein dbo:birthPlace dbr:Ulm`, the predicate is a noun phrase then the subject is replaced by a possessive form which is “seu” (en:“his”). However, Brazilian Portuguese has two different ways to express possession and this variation exists due to the necessity of handling complex syntaxes in some sentences and also because the gender of pronouns agrees with objects instead of subjects. For example, “A professora proibiu que o aluno utilizasse seu dicionário.” (eng: “The teacher forbade the student to use his/her dictionary”). The possessive pronoun *seu* in this sentence does not indicate explicitly to whom the dictionary belongs, if it belongs to the *professora* (eng:teacher) or *aluno* (eng:student). Thus, we have explicitly to define the possessive pronoun in order to decrease the ambiguity in texts and it is obviously important when generating text from data. If this sentence was translated into English, we would have indicated to whom the dictionary belonged, *her* or *his*. To this end, we handle the ambiguity of possessive pronouns by interspersing the alternative forms, e.g., *dele* (eng:his) or *dela* (eng: her)” which agrees with the subject. However, it is used just in case more than one subject exists in the same description. In case the predicate is recognized as a verb (e.g, `dbr: Albert_Einstein dbo:knownFor dbr:General_relativity`), the subject is replaced by its respective personal pronoun *ele* (eng: “he”). While setting the pronouns, RDF2PT recognizes the gender’s subject. The `dbo:knownFor` is a verb phrase, thus the subject is replaced by the personal pronoun “:ele”(see Table 1).

#### Triples before co-reference

- 1 - (Albert Einstein, ser, cientista)
- 2 - (Albert Einstein, local de nascimento, Ulm)
- 3 - (Albert Einstein, ser conhecido por, teoria da relatividade.)

#### Triples after co-reference

- 1 - (Albert Einstein, ser, cientista)
- 2 - (**seu**, local de nascimento, Ulm.)
- 3 - (**ele**, ser conhecido por, teoria da relatividade).

Table 1: Example of triples in the coreference generation task.

### 3.5. Linguistic realisation

This last step is responsible for mapping the obtained descriptions of sentences from the aforementioned tasks and

<sup>8</sup>All rules can be found in our code.

<sup>9</sup>In RDF 1.0 literals have been divided into “plain” literals with no type and optional language tags, and typed literals.

<sup>10</sup>List of data types:<http://tinyurl.com/y95mxyxa>

verbalizing them syntactically, morphologically and orthographically into a correct natural language text. To this end, we perform this step by relying on a Brazilian adaptation of SimpleNLG (De Oliveira and Sripada, 2014).<sup>11</sup>

The realization of a triple  $(s, p, o)$  depends mostly on the lexicalization of its predicate  $p$ . If  $p$  can be realized as a noun phrase, then a possessive clause can be used to express the semantics of  $(s, p, o)$ . For example, if  $(p)$  is a relational noun like `deathPlace` e.g. in the triple  $(\text{:Albert\_Einstein} : \text{deathPlace} : \text{Princeton})$ , then the verbalization is `O local de falecimento de Albert Einstein foi Princeton.` (eng: The death place of Albert Einstein was Princeton) which formally can be expressed as in equation 1. In case there is a previous triple which shares the same subject, it would be `seu local de falecimento foi Princeton` (eng: his death place was Princeton).

$$\rho(s, p, o) \Rightarrow \text{poss}(\rho(p), \rho(s)) \wedge \text{subj}(\text{BE}, \rho(p)) \wedge \text{doobj}(\text{BE}, \rho(o)) \quad (1)$$

In case  $p$ 's lexicalization is a verb, then the triple is verbalized setting the predicate as a verb. For example, in  $(\text{:Albert\_Einstein} : \text{influenced} : \text{Nathan\_Rosen})$   $\rho(p)$  is the verb `influenciar` (en: influence), thus, the verbalization is `Albert Einstein influenciou Nathan Rosen` (eng: Albert Einstein influenced Nathan Rosen) and may be formalized as in equation 2.

$$\rho(s, p, o) \Rightarrow \text{subj}(\text{BE}, \rho(p)) \wedge \text{doobj}(\text{BE}, \rho(o)) \quad (2)$$

RDF2PT is able to merge sentences that were derived from the same cluster for generating a readable summary, thus resulting in coordinate sentences. For example, for the triples  $(\text{:Albert\_Einstein} : \text{birthPlace} : \text{Ulm})$  and  $(\text{:Albert\_Einstein} : \text{deathPlace} : \text{Princeton})$ , if  $p_1$  and  $p_2$  can be verbalized as nouns, then we apply the following rule:

$$\begin{aligned} &\rho(s, p_1, o_1) \wedge \rho(s, p_2, o_2) \Rightarrow \\ &\quad \text{conj}(\text{poss}(\rho(p_1), \rho(s)) \\ &\quad \wedge \text{subj}(\text{BE}_1, \rho(p_1)) \wedge \text{doobj}(\text{BE}_1, \rho(o_1)) \wedge \text{poss}(\rho(p_2), \\ &\quad \rho(\text{pronoun}(s))) \wedge \text{subj}(\text{BE}_2, \rho(p_2)) \\ &\quad \wedge \text{doobj}(\text{BE}_2, \rho(o_2))) \end{aligned} \quad (3)$$

Note that `pronoun(s)` returns the correct pronoun for a resource based on its type and gender (see subsection 3.4.). Therewith, we can generate `O local de nascimento de Albert Einstein Ulm e seu local de falecimento é Princeton.` (eng: Albert Einstein's birthplace is Ulm and his death place is Princeton). In addition, in case the KB provides the ending date of a given resource through some predicate, for example `dbo:deathDate`, RDF2PT is able to lexicalize all the verbs in the past tense.

<sup>11</sup>See the complete list of dependency parsing tags in Ngonga Ngomo et al. (2013).

## 4. Evaluation

We based our evaluation methodology on Gardent et al. (2017) and Ferreira et al. (2016). Our main goal was to evaluate how well RDF2PT represents the information obtained from the data. We hence divided our evaluation set into expert and non-expert users. Both sets were made up of native speakers of Brazilian Portuguese. We selected six DBpedia categories like Gardent et al. (2017) for selecting the topic of texts. The categories were Astronaut, Scientist, Building, WrittenWork, City, and University. We detail below how we carried out both evaluation sets.

**Experts** - We aimed to evaluate the adequacy and fluency of the generated texts from the perspective of experts. All experts hold at least a master degree in the fields NLP or SW. In the questionnaire, we used the same two questions as Gardent et al. (2017): (1) Adequacy: Does the text contain only and all the information from the data? (2) Fluency: Does the text sound fluent and natural? We asked the 10 experts to evaluate 12 texts distributed across the aforementioned DBpedia categories, with two pieces of text from each category. All texts were generated automatically by the RDF2PT approach. The answers were on a scale from 1 to 5.<sup>12</sup>

**Non-experts** - We evaluated the clarity and fluency of the generated texts. To this end, we created three types of texts. First, the texts were generated using a baseline of RDF2PT approach, which removes the functional words and also does not apply coreference rules. This version served as baseline as there is no other work pertaining to generating Brazilian Portuguese from RDF. Second, we used the texts generated using the RDF2PT approach outline at section 3. The third type of texts were created manually by three different human annotators. Table 2 depicts an example of text in the three versions.

In total, we created three versions of 18 texts (one text per resource) selected randomly from the aforementioned DBpedia categories (total: 54 texts). These texts were distributed over three lists, such that each list contained one variant of each text, and there was an equal number of texts from the three types (Baseline, RDF2PT, Human). The experiment was run on CrowdFlower and is publicly available.<sup>13</sup>

The experiment was performed by 30 participants (10 per list). They were asked to rate each text considering the clarity and fluency based on two questions from Ferreira et al. (2016) on a scale from 1 (Very Bad) to 5 (Very Good). The questions were: (1) Fluency: Does the text present a consistent, logical flow? (2) Clarity: Is the text easy to understand?

### 4.1. Results

**Experts** Figure 1 displays the average fluency and clarity of the texts. The results suggest that RDF2PT is able to capture and represent the information from data adequately. Also, the generated texts are fluent enough to be understood by humans.

<sup>12</sup>Questionnaire: <http://tinyurl.com/y9vegl4g>

<sup>13</sup><https://ilk.uvt.nl/~tcastrof/semPT/evaluation/>

| Version  | Text                                                                                                                                                                                                                                                                                                                            |
|----------|---------------------------------------------------------------------------------------------------------------------------------------------------------------------------------------------------------------------------------------------------------------------------------------------------------------------------------|
| Baseline | Albert Einstein é cientista, Albert Einstein campo é física, Albert Einstein lugar falecimento Princeton. Albert Einstein ex-instituição é Universidade Zurique, Albert Einstein é conhecido Equivalência massa-energia, Albert Einstein prêmio é Medalha Max Planck, Albert Einstein estudante doutorado é Ernst Gabor Straus. |
| RDF2PT   | Albert Einstein foi um cientista, o campo dele foi a física e ele faleceu no Princeton. Além disso, sua ex-instituição foi a Universidade de Zurique, ele é conhecido pela Equivalência massa-energia, o prêmio dele foi a Medalha Max Planck e o estudante de doutorado dele foi o Ernst Gabor Straus.                         |
| Human    | Albert Einstein era um cientista, que trabalhava na área de Física. Era conhecido pela fórmula de equivalência entre massa e energia. Formou-se na Universidade de Zurique. Einstein ganhou a medalha Max Planck por seu trabalho. Em Princeton, onde morreu, teve sob sua orientação Ernst Gabor Straus.                       |

Table 2: Example of text in the Baseline, RDF2PT approach and Human version.

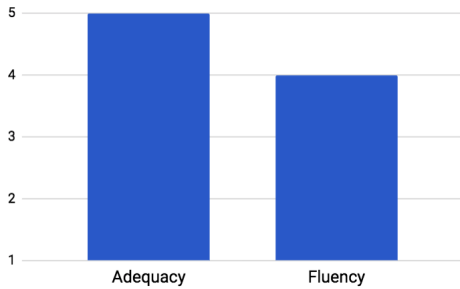

Figure 1: RDF2PT results in experts survey

**Non-experts** Figure 2 depicts the average fluency and clarity of the texts where their topics are described by *Baseline*, *RDF2PT* and *Human* approaches respectively. Inspection of this figure clearly shows that *Baseline* texts are rated lower than both the *RDF2PT* and *Human* texts, in fact, *RDF2PT* is superior to *Baseline* and close to *Human*.

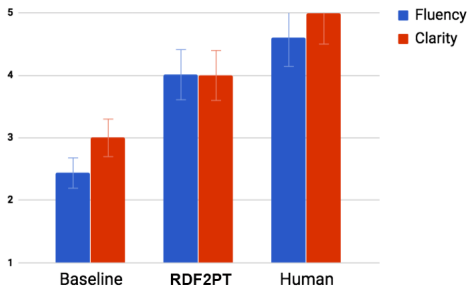

Figure 2: Results in non-experts experiment

We performed a statistical analysis in order to measure the significance of the difference between the types (Baseline, RDF2PT, Human). First, we carried out a Friedman test (Friedman, 1937) which resulted in a significant difference in the fluency ( $\chi^2 = 193.61$ ,  $\rho < 0.0001$ ) and clarity ( $\chi^2 = 180.9$ ,  $\rho < 0.0001$ ) for the three kinds of texts. Afterward, we conducted a post-hoc analysis with Wilcoxon signed-rank test corrected for multiple comparisons using the Bonferroni method, resulting in a significance level set at  $\rho < 0.017$ . Texts of the Baseline are hence significantly less statistically understandable ( $Z=525$  and  $\rho < 0.017$ ) and fluent ( $Z=275.5$  and  $\rho < 0.017$ ) than those generated by the RDF2PT approach. However, RDF2PT also generates texts less comprehensible ( $Z=1617.5$  and  $\rho < 0.017$ )

and fluent ( $Z=1640.0$  and  $\rho < 0.017$ .) than those generated by humans. Clearly, humans were superior to Baseline in terms of comprehensibility ( $Z=234.5$  and  $\rho < 0.017$ .) and fluency ( $Z=264.0$  and  $\rho < 0.017$ .), as we expected. Therefore, there is a significant difference among all models, being baseline < model < human.

## 4.2. Discussion

During the development of RDF2PT, some challenges to our rule-based algorithm became clear. The first challenge was to identify when the object of a predicate is an adjective. Consider the following triple, (`:Albert.Einstein` `dbo:nationality` `:Áustria`), its object `Áustria` is a demonym and should be lexicalized as an adjective. However, it is lexicalized as a noun because the part-of-speech recognized by RDF2PT considers only the label `Austria`, which is a noun, and does not consider the predicate `nationality`, which is an important part, thus decreasing the quality of the generated texts. Second, RDF2PT's algorithm is totally dependent on ontology terms, thus when a given ontology contains wrong labels, RDF2PT is not able to recognize by itself the error and lexicalizes the terms wrongly. Third, the gender continues to be a hard task and RDF2PT sometimes presents poor results. For example, “Os Lusíadas é uns obra literária”, the determiner `uns` should be feminine and singular, because `obra` is singular and has a feminine gender. However, it is accorded to the subject `Os Lusíadas`. This example is similar to the example presented in section 3.4. We hence envision the use of ML algorithms for improving the gender recognition and generation. The last challenge observed was the generation of coordinated sentences by RDF2PT which helped the users in our experimental setup recognize if a given text was generated by RDF2PT or humans. This behavior is because humans are likely to write subordinate sentences. For example, while RDF2PT is able to generate `Albert Einstein foi um cientista e ele nasceu em Ulm.` (eng: Albert Einstein was a scientist and he was born in Ulm), a human would write this same sentence in the following way, `Albert Einstein foi um cientista que/cujo nasceu em Ulm` (eng: Albert Einstein was a scientist who was born in Ulm). This difference was crucial in the perspective of our evaluators. Therefore, the generation of subordinate sentences in Portuguese must be investigated in the near

future.

## 5. Further Application Scenarios

We envision two promising applications using RDF2PT. The first aims to support the automatic creation of benchmarking datasets to Named Entity Recognition (NER) and Entity Linking (EL) tasks. In Brazilian Portuguese, there is a lack of gold standards datasets for these tasks, which makes the investigation of these problems difficult for the scientific community. Our aim is to create Brazilian Portuguese silver standard datasets which are able to be uploaded into GERBIL(Usbeck et al., 2015) for an easy evaluation. To this end, we aim to implement RDF2PT in BENGAL (Ngomo et al., 2017), which is an approach for automatically generating NER benchmarks based on RDF triples and Knowledge Graphs. This application has already resulted in promising datasets which we have used to investigate the capability of multilingual entity linking systems<sup>14</sup> for recognizing and disambiguating entities in Brazilian Portuguese texts. The second appealing application of RDF2PT is the generation of automatic QA systems based on RDF for self-assessment. Therefore, the aim is to develop a Portuguese version of ASSES (Bühmann et al., 2015), which is a self-assessment platform for students based on DBpedia.

## 6. Conclusion

We presented the RDF2PT approach which verbalizes RDF data to Brazilian Portuguese texts. The results demonstrated that RDF2PT generates texts with a good quality of fluency and clarity compared to human texts. In addition, we identified important challenges for generating Brazilian Portuguese texts from RDF using a rule-based approach. We intend to exploit the application of ML models along with other Brazilian Portuguese resources<sup>15</sup> to produce more fluent results and also to investigate the usage of ML classification algorithms to improve the choice of grammatical gender of words.

Moreover, we aim to create a multilingual version of RDF2PT which will consist of French, German, Italian and Spanish. To this end, we will exploit the similarity among their syntaxes in the micro-planning task and we will reuse their respective SimpleNLG versions (Mazzei et al., 2016; Bollmann, 2011; Vaudry and Lapalme, 2013; Ramos-Soto et al., 2017) for the realization task.

## Acknowledgments

This work has been supported by the H2020 project HOB-BIT (GA no. 688227) and supported by the Brazilian National Council for Scientific and Technological Development (CNPq) (no. 206971/2014-1 and no. 203065/2014-0.). This research has also been supported by the German Federal Ministry of Transport and Digital Infrastructure (BMVI) in the projects LIMBO (no. 19F2029I), OPAL

(no. 19F2028A) and GEISER (no. 01MD16014E) as well as by the BMBF project SOLIDE (no. 13N14456).

## Bibliographical References

- Auer, S., Bizer, C., Kobilarov, G., Lehmann, J., Cyganiak, R., and Ives, Z. (2007). Dbpedia: A nucleus for a web of open data. *The semantic web*, pages 722–735.
- Biran, O. and McKeown, K. (2015). Discourse planning with an n-gram model of relations. In *EMNLP*, pages 1973–1977.
- Bollmann, M. (2011). Adapting simplenlg to german. In *Proceedings of the 13th European Workshop on Natural Language Generation*, pages 133–138. Association for Computational Linguistics.
- Bouayad-Agha, N., Casamayor, G., and Wanner, L. (2014). Natural language generation in the context of the semantic web. *Semantic Web*, 5(6):493–513.
- Bühmann, L., Usbeck, R., and Ngomo, A.-C. N. (2015). Assess automatic self-assessment using linked data. In *International Semantic Web Conference*, pages 76–89. Springer, Cham.
- Cimiano, P., Lüker, J., Nagel, D., and Unger, C. (2013). Exploiting ontology lexica for generating natural language texts from rdf data. In *Proceedings of the 14th European Workshop on Natural Language Generation*, pages 10–19, Sofia, Bulgaria, August. Association for Computational Linguistics.
- Colin, E., Gardent, C., Mrabet, Y., Narayan, S., and Perez-Beltrachini, L. (2016). The webnlg challenge: Generating text from dbpedia data. In *Proceedings of the 9th International Natural Language Generation conference*, pages 163–167.
- Cuevas, R. R. M. and Paraboni, I. (2008). A machine learning approach to portuguese pronoun resolution. In *Ibero-American Conference on Artificial Intelligence*, pages 262–271. Springer, Berlin, Heidelberg.
- de Novais, E. M. and Paraboni, I. (2013). Portuguese text generation using factored language models. *Journal of the Brazilian Computer Society*, 19(2):135–146.
- de Novais, E. M., de Oliveira, R. L., Pereira, D. B., Tadeu, T. D., and Paraboni, I. (2009). A testbed for portuguese natural language generation. In *Information and Human Language Technology (STIL), 2009 Seventh Brazilian Symposium in*, pages 154–157. IEEE.
- de Novais, E. M., Tadeu, T. D., and Paraboni, I. (2010). Text generation for brazilian portuguese: the surface realization task. In *Proceedings of the NAACL HLT 2010 Young Investigators Workshop on Computational Approaches to Languages of the Americas*, pages 125–131. Association for Computational Linguistics.
- de Novais, E. M., Paraboni, I., and da Silva Junior, D. F. (2012). Portuguese text generation from large corpora. In *LREC*.
- De Oliveira, R. and Sripada, S. (2014). Adapting simplenlg for brazilian portuguese realisation. In *INLG*, pages 93–94.
- Duma, D. and Klein, E. (2013). Generating natural language from linked data: Unsupervised template extraction. In *IWCS*, pages 83–94.

<sup>14</sup><http://gerbil.aksw.org/gerbil/experiment?id=201801050040> and <http://gerbil.aksw.org/gerbil/experiment?id=201801110012>

<sup>15</sup>Resources: <http://www.nilc.icmc.usp.br/nilc/index.php/tools-and-resources>

- Ell, B. and Harth, A. (2014). A language-independent method for the extraction of rdf verbalization templates. In *INLG*, pages 26–34.
- Ell, B., Vrandečić, D., and Simperl, E. P. B. (2011). Labels in the web of data. In *Proceedings of ISWC*, volume 7031, pages 162–176. Springer.
- Ferreira, T. C., Krahmer, E., and Wubben, S. (2016). Towards more variation in text generation: Developing and evaluating variation models for choice of referential form. In *ACL (1)*.
- Friedman, M. (1937). The use of ranks to avoid the assumption of normality implicit in the analysis of variance. *Journal of the american statistical association*, 32(200):675–701.
- Gardent, C., Shimorina, A., Narayan, S., and Perez-Beltrachini, L. (2017). Creating training corpora for nl micro-planning. In *Proceedings of ACL*.
- Gatt, A. and Krahmer, E. (2017). Survey of the state of the art in natural language generation: Core tasks, applications and evaluation. *arXiv preprint arXiv:1703.09902*.
- Gkatzia, D., Hastie, H. F., and Lemon, O. (2014). Comparing multi-label classification with reinforcement learning for summarisation of time-series data. In *ACL (1)*, pages 1231–1240.
- Hewlett, D., Kalyanpur, A., Kolovski, V., and Halaschek-Wiener, C. (2005). Effective nl paraphrasing of ontologies on the semantic web. In *Workshop on end-user semantic web interaction, 4th int. semantic web conference, galway, ireland*.
- Keet, C. M. and Khumalo, L. (2017). Toward a knowledge-to-text controlled natural language of isizulu. *Language Resources and Evaluation*, 51(1):131–157.
- Lehmann, J., Isele, R., Jakob, M., Jentzsch, A., Kontokostas, D., Mendes, P. N., Hellmann, S., Morsey, M., Van Kleef, P., Auer, S., et al. (2015). Dbpedia—a large-scale, multilingual knowledge base extracted from wikipedia. *Semantic Web*, 6(2):167–195.
- Mazzei, A., Battaglini, C., and Bosco, C. (2016). Simplenlg-it: adapting simplenlg to italian. In *INLG*, pages 184–192.
- Mohammed, R., Perez-Beltrachini, L., and Gardent, C. (2016). Category-driven content selection. In *Proceedings of the 9th International Natural Language Generation conference*, pages 94–98.
- Mrabet, Y., Vougiouklis, P., Kilicoglu, H., Gardent, C., Demner-Fushman, D., Hare, J., and Simperl, E. (2016). Aligning texts and knowledge bases with semantic sentence simplification. *WebNLG 2016*.
- Ngomo, A. N., Röder, M., Moussallem, D., Usbeck, R., and Speck, R. (2017). Automatic generation of benchmarks for entity recognition and linking. *CoRR*, abs/1710.08691.
- Ngonga Ngomo, A.-C., Bühlmann, L., Unger, C., Lehmann, J., and Gerber, D. (2013). Sorry, i don’t speak sparql: translating sparql queries into natural language. In *Proceedings of the 22nd international conference on World Wide Web*, pages 977–988. ACM.
- Page, L., Brin, S., Motwani, R., and Winograd, T. (1999). The pagerank citation ranking: Bringing order to the web. Technical report, Stanford InfoLab.
- Pereira, D. and Paraboni, I. (2008). Statistical surface realisation of portuguese referring expressions. *Advances in Natural Language Processing*, pages 383–392.
- Pereira, J. C., Teixeira, A., and Pinto, J. S. (2015). Towards a hybrid nlg system for data2text in portuguese. In *Information Systems and Technologies (CISTI), 2015 10th Iberian Conference on*, pages 1–6. IEEE.
- Perez-Beltrachini, L., Sayed, R., and Gardent, C. (2016). Building rdf content for data-to-text generation. In *COLING*, pages 1493–1502.
- Ramos-Soto, A., Janeiro-Gallardo, J., and Bugarín, A. (2017). Adapting SimpleNLG to spanish. In *10th International Conference on Natural Language Generation*.
- RDF Working Group, W. (25 February 2014). *RDF 1.1 Concepts and Abstract Syntax*. W3C Recommendation. Available at <https://www.w3.org/TR/rdf11-concepts/>.
- Reiter, E. and Dale, R. (2000). *Building natural language generation systems*. Cambridge university press.
- Schwitler, R., Tilbrook, M., et al. (2004). Controlled natural language meets the semantic web. In *Proceedings of the Australasian Language Technology Workshop*, volume 2, pages 55–62.
- Sleimi, A. and Gardent, C. (2016). Generating paraphrases from dbpedia using deep learning. *WebNLG 2016*, page 54.
- Staykova, K. (2014). Natural language generation and semantic technologies. *Cybernetics and Information Technologies*, 14(2):3–23.
- Sun, X. and Mellish, C. (2006). Domain independent sentence generation from rdf representations for the semantic web. In *Combined Workshop on Language-Enabled Educational Technology and Development and Evaluation of Robust Spoken Dialogue Systems, European Conference on AI, Riva del Garda, Italy*.
- Theune, M., Klabbers, E., de Pijper, J.-R., Krahmer, E., and Odijk, J. (2001). From data to speech: a general approach. *Natural Language Engineering*, 7(1):47–86.
- Usbeck, R., Röder, M., Ngonga Ngomo, A.-C., Baron, C., Both, A., Brümmer, M., Ceccarelli, D., Cornolti, M., Cherix, D., Eickmann, B., Ferragina, P., Lemke, C., Moro, A., Navigli, R., Piccinno, F., Rizzo, G., Sack, H., Speck, R., Troncy, R., Waitelonis, J., and Wesemann, L. (2015). GERBIL – general entity annotation benchmark framework. In *24th WWW conference*.
- Vaudry, P.-L. and Lapalme, G. (2013). Adapting simplenlg for bilingual english-french realisation. In *ENLG*, pages 183–187.
- Xu, K., Ba, J., Kiros, R., Cho, K., Courville, A., Salakhudinov, R., Zemel, R., and Bengio, Y. (2015). Show, attend and tell: Neural image caption generation with visual attention. In *International Conference on Machine Learning*, pages 2048–2057.
