# Supplementary material for: Knowledge Graphs for Multilingual Language Translation and Generation
Source: arXiv:2009.07715 source file (2020-09-16)
Supplement: Supplementary file 9 [file THOTH.pdf]

# THOTH: Neural Translation and Enrichment of Knowledge Graphs

Diego Moussallem<sup>1</sup>, Tommaso Soru<sup>2</sup>, and Axel-Cyrille Ngonga Ngomo<sup>1</sup>

<sup>1</sup> Data Science Group, University of Paderborn, Germany  
first.lastname@upb.de

<sup>2</sup> AKSW Research Group, University of Leipzig, Germany  
lastname@informatik.uni-leipzig.de

**Abstract.** Knowledge Graphs are used in an increasing number of applications. Although considerable human effort has been invested into making knowledge graphs available in multiple languages, most knowledge graphs are in English. Additionally, regional facts are often only available in the language of the corresponding region. This lack of multilingual knowledge availability clearly limits the porting of machine learning models to different languages. In this paper, we aim to alleviate this drawback by proposing THOTH, an approach for translating and enriching knowledge graphs. THOTH extracts bilingual alignments between a source and target knowledge graph and learns how to translate from one to the other by relying on two different recurrent neural network models along with knowledge graph embeddings. We evaluated THOTH extrinsically by comparing the German DBpedia with the German translation of the English DBpedia on two tasks: fact checking and entity linking. In addition, we ran a manual intrinsic evaluation of the translation. Our results show that THOTH is a promising approach which achieves a translation accuracy of 88.56%. Moreover, its enrichment improves the quality of the German DBpedia significantly, as we report +18.4% accuracy for fact validation and +19% F<sub>1</sub> for entity linking.

## 1 Introduction

A recent survey estimates that more than 3.7 billion humans use the internet every day and produce nearly 2.5 quintillion bytes of data on the Web each day.<sup>3</sup> The availability of such large amounts of data is commonly regarded as one of the motors for the current lapses in the development of Artificial Intelligence (AI)-powered solutions. In this paper, we focus on the portion of data made available in the form of Knowledge Graph (KG). Recent works have shown the benefits of exploiting KGs to improve Natural Language Processing (NLP) tasks such as Natural Language Inference (NLI) [20] and Question Answering (QA) [35]. A given KG (especially Resource Description Framework (RDF) KG) commonly stores knowledge in triples. Each triple consists of (i) a subject—often an entity, (ii) a relation—often called property—and (iii) an object—an entity or a literal.<sup>4</sup> For example, `<Edmund_Hillary, birthPlace,`

<sup>3</sup> <https://tinyurl.com/statswebdata>

<sup>4</sup> a string or a value with a unit

Auckland>,<sup>5</sup> represents the information that “Edmund Hillary was born in Auckland”.

Considerable amounts of partly human effort has been invested in making KGs available across languages. However, even popular KGs like DBpedia and Wikidata are largest in their English version [25]. Additionally, region-specific facts are often limited to the KG specific to the region from which they emanate or to the KG in the language spoken in said region [1]. This lack of multilingual knowledge availability limits the porting of Machine Learning (ML) models to different languages. The Semantic Web (SW) community has been trying to alleviate this bottleneck by creating different approaches for enriching the Linked Open Data (LOD) cloud with multilingual content. However, it is a difficult endeavor as the majority of ML algorithms for extracting knowledge from raw data only support English.

Previous works have tried to address this problem by using Machine Translation (MT) systems [27, 2]. However, these works focused only on translating the labels of domain-specific KGs from English into a target language. This kind of approach ignores an essential part of a KG, namely its graph structure. For example, while translating a highly ambiguous label such as *Kiwi*, an MT system has to predict in which domain this word has to be translated in the target language. Otherwise, the translation of *Kiwi* can be the common term for inhabitants of New Zealand,<sup>6</sup> a fruit,<sup>7</sup> a bird,<sup>8</sup> or a computer program.<sup>9</sup> These domains can be derived in KGs through predicates such as type predicates (i.e., `rdf:type` in RDF). Clearly, taking the graph structure of KG into account can support an MT system when spotting the correct translation for ambiguous labels.

RDF KGs rely on Uniform Resource Identifier (URI)s for the unique identification of relations (predicates) and resources (entities).<sup>10</sup> While some KGs use encoded URIs with numeric IDs (e.g., Wikidata), most KGs use language-based URIs, which allows humans to derive the semantics behind the URI by reading it. For example, the Multilingual KG DBpedia is composed of independent KGs in different languages interlinked by `owl:sameAs` relations. We argue that if a KG uses human-legible URI, then an enrichment approach for language-based KGs should not simply translate only the labels of its resources and maintain or change its URI prefixes by adding a language code. It should also be able to generate correct URIs during the translation process. For instance, changing an English DBpedia resource `<http://dbpedia.org/resource/United_Kingdom>` to a German DBpedia resource `<http://de.dbpedia.org/resource/United_Kingdom>` is inherently incorrect since this entity already exists with another URI in the German DBpedia (i.e., `<http://de.dbpedia.org/resource/Vereinigtes_Königreich>`). Consequently, a simple translation of labels without a translation of URIs would assign a supplementary URI to an existing resource, hence breaking the uniqueness of URIs within single KGs. Thus, an approach for translating KGs must be capable of translating labels and URIs.

<sup>5</sup> [http://dbpedia.org/page/Edmund\\_Hillary](http://dbpedia.org/page/Edmund_Hillary)

<sup>6</sup> [http://dbpedia.org/resource/Kiwi\\_\(people\)](http://dbpedia.org/resource/Kiwi_(people))

<sup>7</sup> <http://dbpedia.org/resource/Kiwifruit>

<sup>8</sup> <http://dbpedia.org/resource/Kiwi>

<sup>9</sup> <http://dbpedia.org/resource/KiwiIRC>

<sup>10</sup> <https://www.w3.org/TR/cooluris>

In this work, we focus on translating and enriching KGs with language-based URIs to provide KGs in different languages. To this end, we present THOTH, an approach which considers the graph structure of the KG while translating its URIs along with their labels. First, THOTH extracts bilingual alignments between a source and target KG using SPARQL queries. Afterwards, THOTH uses the acquired bilingual knowledge to train two different Neural Machine Translation (NMT) models based on an Recurrent Neural Network (RNN), (1) triple- and (2) text-based. The triple-based RNN model is trained only on triples represented by `<resource, predicate, resource>` while the text-based RNN model, is trained on generic bilingual parallel corpora and is able to translate triples which contain literals (texts), i.e., `<resource, predicate, literal>`. Both models are enriched with Knowledge Graph Embeddings (KGE) created from the source and target KGs. We envision that THOTH can benefit and support the multilinguality in the LOD cloud and the SW.

With this aim, we apply THOTH on the English and German DBpedia [4]. We hence evaluate the enriched German DBpedia both extrinsically and intrinsically. The extrinsic evaluation is carried out on the tasks of fact checking and Entity Linking (EL). The intrinsic evaluation is carried out by means of a manual error analysis of a sample of the data. The main contributions of this paper can be summarized as follows:

- We present a novel approach based on Neural Network (NN)s along with KGEs for translating and enriching KGs across languages.
- THOTH is a promising approach which achieves a translation accuracy of 88.56% across all elements of a triple. Also, its enrichment improves the quality of the original German DBpedia significantly in both the fact checking and the EL tasks: We achieve improvements of 18.4% for fact validation and 19% for EL.

The version of THOTH used in this paper and also all experimental data are publicly available.<sup>11</sup>

## 2 Related Work

A wide range of works have investigated the enrichment of KGs through different techniques, for example, MT [16], cross-lingual knowledge interlinking and alignment [11], natural language generation [21] and KGE [12]. In this section, we briefly describe recent approaches which exploited the enrichment of KGs from the MT aspect and also worked on the development of KGE which is an important part of our approach.

**KG Translation** According to a recent survey [30], the translation of KGs has been carried out through a localization task which relies on Statistical Machine Translation (SMT) systems for translating the labels of KGs and domain-specific ontologies into target languages. Recently, Arčan and Buitelaar [3] performed the translation of domain-specific expressions from medical and financial domains represented by English KGs into other languages by relying on an NMT architecture. They showed that

<sup>11</sup> <https://github.com/dice-group/THOTH>

the results of NMT surpassed the SMT. As a way of overcoming the weakness of previous works, Feng et al. [16] presented an NN approach, which learns continuous triple representation with a gated NN for translating an English KG into Chinese. The authors built their approach upon a subset of Freebase [7] and mapped the source and target triples in the same semantic vector space. Consequently, their technique was capable of learning the KG structure for translating the terms. Their adapted NN approach improved the translation accuracy over a strong NMT baseline and showed that considering a KG structure is essential for performing a KG translation and leads to a better disambiguation quality for ambiguous terms.

**Knowledge Graph Embeddings** Manifold approaches interpret relationships as displacements operating on low-dimensional embeddings of entities, e.g. TransE [8]. More recently, Nickel et al. [31] proposed HolE, which relies on holographic models of associative memory by employing a circular correlation to create compositional representations. Ristoski and Paulheim [33] presented RDF2Vec, which uses language modeling approaches for unsupervised feature extraction from sequences of words and adapts them to RDF graphs. RDF2Vec has been extended to reduce the computational time and bias of random walking [13]. In its subsequent extension, Cochez et al. [14] exploited the Global Vectors algorithm in RDF2Vec for computing embeddings from the co-occurrence matrix of entities and relations without generating the random walks. However, Joulin et al. [19] showed recently that a simple Bag-of-Words (BoW) based approach with the *fastText* algorithm [18] generates surprisingly good KGE while achieving state-of-the-art results.

### 3 Preliminaries

In the following, we present preliminary concepts of NMT and KGE for a better understanding of THOTH approach.

**Neural Machine Translation** In this work, we use the RNN architecture. It consists of an encoder and a decoder, i.e., a two-tier architecture where the encoder reads an input sequence  $x = (x_1, \dots, x_n)$  and the decoder predicts a target sequence  $y = (y_1, \dots, y_n)$ . Encoder and decoder interact via a soft-attention mechanism [5, 26], which comprises one or multiple attention layers. We follow the notations from Tang et al. [36] in the subsequent sections:  $h_i^l$  corresponds to the hidden state at step  $i$  of layer  $l$ .  $h_{i-1}^l$  represents the hidden state at the previous step of layer  $l$  while  $h_i^{l-1}$  means the hidden state at  $i$  of  $l-1$  layer.  $E \in \mathbb{R}^{m \times K_x}$  is a word embedding matrix,  $W \in \mathbb{R}^{n \times m}$ ,  $U \in \mathbb{R}^{n \times n}$  are weight matrices, with  $m$  being the word embedding size and  $n$  the number of hidden units.  $K_x$  is the vocabulary size of the source language. Thus,  $E_{x_i}$  refers to the embedding of  $x_i$ , and  $e_{pos,i}$  indicates the positional embedding at position  $i$ . In RNN models, networks change as new inputs (previous hidden state and the token in the line) come in, and each state is directly connected to the previous state only. Therefore, the path length of any two tokens with a distance of  $n$  in RNNs is exactly  $n$ . Its architecture enables adding more layers, whereby two adjoining layers are usually connected with residual connections in deeper configurations. Equation 1 displays  $h_i^l$ , where  $f_{rnn}$  is usually a

function based on Gated recurrent unit (GRU) or Long Short-Term Memories (LSTM). The first layer is then represented as  $h_i^0 = f_{rnn}(WE_{x_i}, Uh_{i-1}^0)$ . Additionally, the initial state of the decoder is commonly initialized with the average of the hidden states or the last hidden state of the encoder.

$$h_i^l = h_i^{l-1} + f_{rnn}(h_i^{l-1}, h_{i-1}^l) \quad (1)$$

**Knowledge Graph Embeddings** The underlying concept of KGE is that, in a given KG, each subject entity  $h$  or object entity  $t$  can be associated with a vector in a continuous vector space whereby its relation  $r$  can be modelled as displacement vectors ( $h + r = t$ ) while preserving the inherent structure of the KG. In fastText [19], the model is based on BoW representation which considers the subject entities  $h$  and object entities  $t$  along with their relation  $r$  as a unique discrete token. Thus, fastText models the co-occurrences of entities and its relations with a linear classifier and standard cost functions. Hence, it allows theoretically creating either a structure-based or semantically-enriched KGE. Therefore, we use fastText models in our experiments.<sup>12</sup> The aim of the algorithm is represented by the following equation:

$$-\frac{1}{N} \sum_{n=1}^N y_n \log(f(WVz_n)), \quad (2)$$

The normalized BoW of the  $x_n$  input set is represented as  $z_n$ ,  $y_n$  as the label.  $V$  is a matrix, which is used as a look-up table over the discrete tokens and a matrix  $W$  is used for the classifier. The representations of the discrete tokens are averaged into BoW representation, which is in turn fed to a linear classifier.  $f$  is used to compute the probability distribution over the classes, and  $N$  input sets for discrete tokens.

## 4 The THOTH Approach

NNs have shown an impressive capability of parsing and translating natural language sentences. For example, the application of NN within MT systems led to a remarkable performance over well-established Phrase-based SMT approaches [22]. Consequently, the interest in NMT for devising new solutions to translation problems increased. The underlying idea behind our approach, THOTH, is based on the formal description of a translation problem as follows: *Given that KGs are composed of facts extracted from text, we can consider the facts (i.e., triples) as sentences where URIs are tokens and train a NMT model to translate the facts from one language into another.* The enrichment process implemented by THOTH consists of two phases. The data gathering and preprocessing steps occur in the training phase, while the enrichment per se is carried out during the translation phase and consists of two steps: 1) translation and 2) enrichment. All steps carried out in THOTH are language-agnostic, which allow the use of other language-based KGs. An overview can be found in Figure 1.

<sup>12</sup> We could not use RDF2Vec in our work as its code was incomplete.

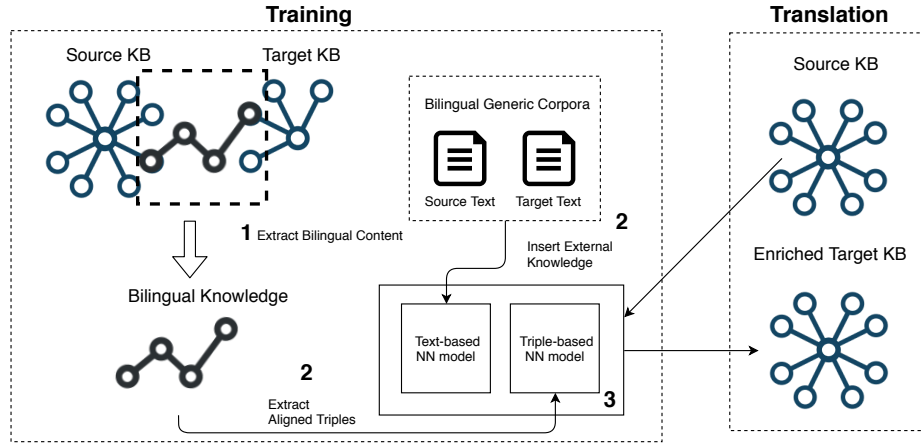

Fig. 1: Overview of THOTH.

#### 4.1 Training Phase

While devising our approach, we perceived that one crucial requirement is that all resources and predicates in the source and target KGs must have at least one label via a common predicate such as `rdfs:label`.<sup>13</sup> This avoids the generation of inadequate resources. After establishing this, we divide THOTH into two models in order to take into account the challenge of translating datatype property values (i.e., texts) and object property values (i.e., entities). Trying to tackle both kinds of statements with a single model is likely to fail as labels can easily reach a length of 50 characters. Therefore, we divide the data gathering process into two blocks in order to be able to train 2 models.

**Data gathering process.** First, we upload the source and target KG into a SPARQL endpoint and query both graphs by looking for resources which have the same “identity”. Identical resources are usually connected via `owl:sameAs` links. However, aligned triples must not contain `owl:sameAs` as predicates in themselves (see line 7 in Listing 1.1). Second, we perform another SPARQL query for gathering only the labels of the aligned resources. Thus, we generate two bilingual training files, one with triples and another with labels (see Listing 1.2 for an example). Once both training files are created, we split them into training, development, and test sets.

**Preprocessing.** Before we start training the triple- and text-based models, we tokenize both training data files. Subsequently, we apply Byte Pair Encoding (BPE) models on them for dealing with out-of-vocabulary (OOV) words [34]. BPE is a form of data compression that iteratively replaces the most frequent pair of bytes in a sequence with a single, unused byte. The symbol vocabulary is initialized with the character vocabulary, and each word is represented as a sequence of characters-plus a special end-of-word

<sup>13</sup> <https://www.w3.org/TR/webont-req/#section-requirements>

```

1 SELECT *
2 WHERE {
3     ?s1 ?p1 ?o1 .
4     ?s2 ?p2 ?o2 .
5     ?s1 owl:sameAs ?s2 .
6     ?o1 owl:sameAs ?o2 .
7 FILTER(?p1 != owl:sameAs && ?p2 != owl:sameAs)
8 } ORDER BY ?s1 ?o1 LIMIT 1000000

```

Listing 1.1: A SPARQL query for retrieving aligned bilingual triples

```

1 EN: dbr:crocodile_dundee_ii dbo:country dbr:united_states
2 DE: dbr_de:crocodile_dundee_ii dbo:country dbr_de:vereinigte_staaten
3 EN: dbr:til_there_was_you dbo:writer dbr:winnie_holzman
4 DE: dbr_de:zwei_singles_in_l.a. dbo:writer dbr_de:winnie_holzman

```

Listing 1.2: Sample of the triple-based training data

symbol, which allows restoring the original tokenization after the translation step. For example, suppose we have the entity or label “Auckland”, after the BPE, i.e., the sub-word information, it becomes Au■ ck■ la■ nd.<sup>14</sup> Applying BPE on the training data allows the translation models to translate words and sub-words and consequently improve their translation performance. It is a well-known technique from the MT community for handling the open vocabulary problem.

**Knowledge Graph Embeddings.** Based on recent findings [28], we generate KGEs from the aligned triples along with their labels by using *fastText*. We rely on multinomial logistic regression [6] as a classifier in a supervised training implemented in *fastText*. It assigns the entity’s URI to its surface forms. For example, the triple with literal, `<dbr:ISWC, rdfs:label, International Semantic Web Conference>` becomes `<__label__dbr:ISWC International Semantic Web Conference>` for training the KGE<sup>15</sup>. This technique enables the NN to retrieve from KGE the surface form of the entities through their URIs.

**Training.** Both triple- and text-based models rely on a standard RNN model described in section 3. The difference between both models is the training data format. The Triple-based model is trained only with the aligned triples, while the text-based was trained with an external generic bilingual corpora. Additionally, both models are augmented with a KGE model. The idea of using KGE is to maximize the vector values of the triple-based and text-based NMT embeddings layers while training their models. An overview of the training phase can be found in Figure 2 for a better understanding.

<sup>14</sup> The black squares represents how the model splits the frequent tokens in a sequence for a better translation process.

<sup>15</sup> More than one surface forms can be assigned to the entities.

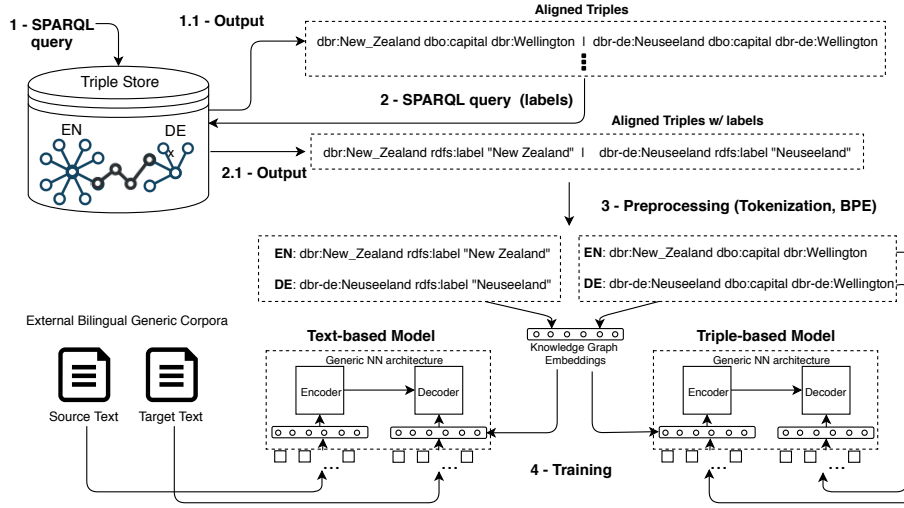

Fig. 2: Training phase overview

## 4.2 Translation Phase

Here, THOTH expects the entire source KG as an input to be translated and enriched into the target language as an output. To this end, THOTH first relies on a script which is responsible for splitting the KG triples which comprises only the resources in one file and the triples which contain literals as objects in a different file. Once the division is done, and two set files are generated, THOTH starts translating the triples only with resources. After that, THOTH has to deal with the triples which have labels, and they are handled differently. The subject and predicate of the triples are sent to the Triple-based model along with a special character in the place of its object. For example, suppose THOTH is parsing the following triple, `<dbr:ISWC, rdfs:label, International Semantic Web Conference>`, it is sent to the Triple-based model as `<dbr:ISWC, rdfs:label, ▲`. This special character simply tells the model to ignore the value and copy it to the target. In turn, the Text-based NMT model translates only the object; in this case, the label *International Semantic Web Conference*. We argue that the Text-based model can translate the labels correctly since its model was augmented with a KGE model representing the URIs of both KGs, source and target. We hence hypothesize that since neural models learn translations in a continuous vector space, they can assimilate and link the labels with the entities and correctly translate the labels. Afterwards, subject and predicate are attached with their object literal in a triple again. Finally, the two different files are combined into one again resulting in a translated KG. Once the translation step is complete, THOTH gets the translated KG, and the original target (German) KG used in the training part and combines both into a single KG. The idea here is to enrich the original KG with translated triples. When conflicts of values, for example, the triples match partially, and duplicated triples appear between the original KG and the translated KG, we opt to maintain the triples from the



original KG as THOTH’s aim is not to produce a newly translated KG but enrich the original one.

## 5 Evaluation

### 5.1 Goals

In our evaluation, we plan to address the following research questions:

- Q1: Can NNs along with KGE support a full (triples and labels) translation of KGs?
- Q2: How accurate are the triples generated by THOTH?
- Q3: Can an artificially enriched KG improve the performance of a system on NLP tasks?

To this end, we designed our evaluation in three-fold set. First, we measure the performance of THOTH using an automatic MT evaluation metric, BLEU, along with its translation accuracy. Second, we evaluated THOTH extrinsically by comparing the German DBpedia with the German translation of the English DBpedia on two tasks: Fact Validation and Entity Linking. Third, we ran a manual intrinsic evaluation of the translation. We choose German as a target language because of the abundance of benchmarking systems and datasets for this pair.

### 5.2 Experimental Setup

In our experiments, we based the parameters on previous literature [24]. Both the triple-based and the text-based NMT models are built upon an RNN architecture using a bi-directional 2-layer LSTM encoder-decoder model with attention mechanism [5]. The training uses a batch size of 32 and the stochastic gradient descent with an initial learning rate of 0.0002. We set the dimension of the word embeddings to 500 and the internal embeddings of hidden layers to size 500. The dropout is set to 0.3 (naive). We use a maximum sentence length of 50, a vocabulary of 50,000 words and a beam size of 5. All experiments are performed with the OpenNMT framework [23]. In addition, we encode the triples and words using BPE [34] with 32,000 merge operations.

For training the text-based model, our training set consists of a merge of all parallel training data provided by the Workshop on Machine Translation (WMT) tasks<sup>16</sup>, obtaining after preprocessing a corpus of five million sentences with 79M running words. In the triple-based model, we use the bilingual alignments from the English, and German versions of DBpedia<sup>17</sup> for training. This alignment contains 346,373 subjects, 292 relations and 208,079 objects in 1,012,681 triples. We divide this data into 80% training, 10% development and 10% test. Overall, the English KG contains 4.2 million entities, 661 relations, and 2.1 million surface forms, while the German version has 1 million entities, 249 relations, and 0.5 million surface forms. Additionally, we train the KGE

<sup>16</sup> <http://www.statmt.org/wmt18/translation-task.html>

<sup>17</sup> We selected the subsets of mapping-based objects and labels to evaluate the quality of our approach since they are the most used ones for training Linked-Data NLP approaches.

on both DBpedia versions using the *fastText* algorithm (Equation 2) with a vector dimension size of 500 and a window size of 50 by using 12 threads with hierarchical softmax.

The overall enrichment quality of THOTH is measured by working through different steps. Firstly, we evaluate the translations automatically by computing a translation accuracy with BLEU [32] score which is a cost-effective and standard MT evaluation metric. BLEU uses a modified precision metric to compare the MT output with the reference (i.e., human) translation. This automatic evaluation is done with a bilingual aligned triples test set. In the subsequent evaluation steps, we investigate THOTH’s performance on a full KG translation setting. In this case, we use THOTH models for translating and enriching all Concise Bounded Description (CBD) resources of English DBpedia to an enriched-German DBpedia version. The further extrinsic evaluation steps are described below.

**Fact validation task** In line with the data quality metrics proposed in Zaveri et al. [39], our KG translation approach can address the dimension of the completeness of KGs. An area in which completeness has a significant impact is fact validation. Hence, fact validation benchmarks can be used as a proxy for measuring our translation quality as they provide both true and false facts. We selected FactBench—a multilingual benchmark dataset for the evaluation of fact validation algorithms [17]—for our experiments. FactBench contains positive and negative facts. We only use the 750 positive facts distributed over 10 relations as reference data in our experiment. Our aim is to check the number of true facts which existed in the original KG (i.e., in the German version of DBpedia) and how many true triples THOTH was able to add to the KG through enrichment. We used 5 of the 10 predicates in our evaluation data set, i.e., *award*, *birthplace*, *deathplace*, *leader*, *starring* because the other predicates do not lead to sufficient training data. Overall, our evaluation dataset consists of a total count of 375 facts.

**NLP task.** One of the most important NLP techniques for extracting knowledge automatically from unstructured data is Entity Linking, also known as Named Entity Disambiguation (NED). The goal of an EL approach is as follows: Given a piece of text, a reference knowledge graph  $K$  and a set of entity mentions in that text, map each entity mention to the corresponding resource in  $K$ . Our idea here is to exploit the graphs connections from the enriched-German DBpedia (THOTH) KG to improve a given EL system on a disambiguation task. We chose MAG, a multilingual EL system introduced by [29], which is language- and KG-agnostic. MAG does not require any training while showing competitive results. Also, we selected GERBIL [37] as a benchmarking platform because it has been widely used for evaluating different NLP tasks. In this task, we had to make the URIs of the gold standard datasets lowercase before performing our experiment since the THOTH translation models produces lower-cased URIs. The URI case sensitivity is dependent on the implementation of the web server<sup>18</sup>. Thus, converting all URIs to lowercase is valid and does not produce false results. As the

<sup>18</sup> <https://tools.ietf.org/html/rfc3986#section-3.1>

evaluation is on the German language, we uploaded four German datasets to GERBIL (see Table 1). The **VoxEL** dataset is a manually annotated gold standard. This dataset has two versions: (i) a strict version *VoxEL-strict* where entities correspond to a restricted definition of entity, as a mention of a person, place or organization, and (ii) a relaxed version *VoxEL-relaxed*, where a broader selection of mentions referring to entities described by Wikipedia is maintained. The **N<sup>3</sup> news.de** dataset is a real-world dataset collected from 2009 to 2011, which contains documents from the German news portal `news.de`. Finally, **DBpedia Abstracts** is a large, multilingual corpus generated from enriched Wikipedia data of annotated Wikipedia abstracts [9]. This corpus stems from Wikipedia annotations which were created manually.<sup>19</sup>

Table 1: Dataset statistics.

| Corpus                 | Language | Topic | Documents | Entities |
|------------------------|----------|-------|-----------|----------|
| VoxEL-strict           | German   | news  | 15        | 204      |
| VoxEL-relaxed          | German   | news  | 15        | 674      |
| N <sup>3</sup> news.de | German   | news  | 53        | 627      |
| German Abstract        | German   | mixed | 38,197    | 346,448  |

### 5.3 Results

In this section, we report the results of THOTH’s enrichment in the German DBpedia on the settings mentioned above. Also, we aim to answer the three research questions defined in Section 5.1 and carried out a thorough manual analysis of our results.

**Translation results.** We evaluated our translation on the test set of the bilingual data we extracted via SPARQL queries (see Section 5.2). To this end, we used the THOTH models for translating source English triples to German triples. First, we computed the BLEU score by comparing THOTH’s output with the corresponding target (German) side of the bilingual test set. THOTH achieved a BLEU score of 65.47, which is superior to the state-of-the-art translation scores achieved on natural language [15].

Given that it is not possible to infer the quality of a given translation only relying on one automatic evaluation metric, we created an additional evaluation script which computes the exact string match of subjects, predicates, and objects between an output and a reference translation triple. Additionally, we also computed the overall triple accuracy. For example, given the following triple from THOTH’s output, `<dbr_de:iago_falque dbo:club dbr_de:fc_turin>`, we measure if its subject, predicate and object are equal to the ones of the reference translation; in this case, we found it to be the same. However, in the case where some of them are different, the accuracy of the triple is 0 because the meaning of the triple is wrong in comparison to its reference. Figure 3 depicts the accuracy results of THOTH’s output in comparison

<sup>19</sup> We reduced our testset to the first subset of provided abstracts due to evaluation platform limits

to the German test set. THOTH achieved up to 80% accuracy for subjects, predicates, and objects. As expected, THOTH’s accuracy decreased to 68.83% while measuring entire triples. We analyzed the results manually to understand this drop in the performance. Our manual analysis suggests that the poorer performance w.r.t. triples is linked to the partially weak disambiguation power of the underlying KGE model, which assigned the same vector value for similar predicates. We discuss this particular challenge along with other findings in Section 5.4. Regarding **Q1**, our results confirm that NNs along KGE can support a full KG translation by considering the consistent quality of THOTH translations.

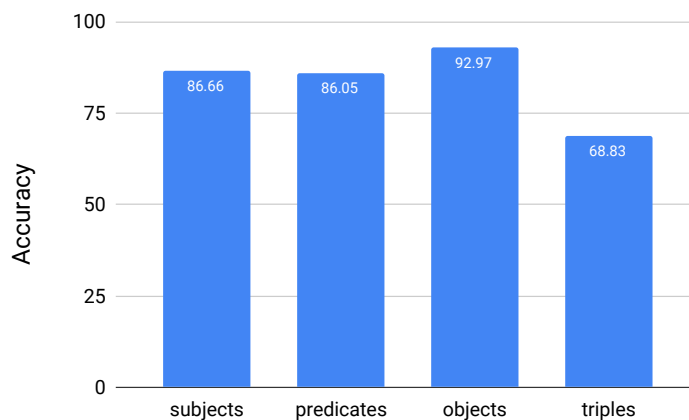

Fig. 3: Overall translation accuracy

**Fact validation results.** Here, we used THOTH to translate the entire English DBpedia to German. In this case, we do not have a gold standard translation to compare automatically. Therefore, we evaluated the THOTH’s enrichment capability in the perspective of a fact-validation task. The main goal here was to check if THOTH could enrich the original German KG with new correct facts which were not present in its original version. Figure 4 reports an improvement of 18.4% across all predicates. Interestingly, the original German DBpedia KG did not contain any fact with the predicate `award` from the FactBench dataset. However, after THOTH’s enrichment, its coverage of FactBench increased to 28%. We also noticed an improvement of 48% w.r.t. the `leader` predicate. Further (even if smaller) increases can be seen in the `birthPlace`, `deathPlace`, and `starring` predicates, where we achieve an average enhancement of 4%. Delving into the data shows that the predicates which got modest improvements are the most mapped by the German DBpedia from Wikipedia<sup>20</sup>. Consequently, these predicates are present in abundance in the original German KG. Overall, it becomes clear that THOTH

<sup>20</sup> <http://mappings.dbpedia.org/server/statistics/de/>

achieves the task of improving the quality of KGs w.r.t. their completeness. Additionally, we can answer **Q2** with the results of THOTH on the fact-validation task, where it achieved an increase of +18.4% accuracy. THOTH obviously led to a significant increase in the number of correct facts in the original KG.

## Fact-validation

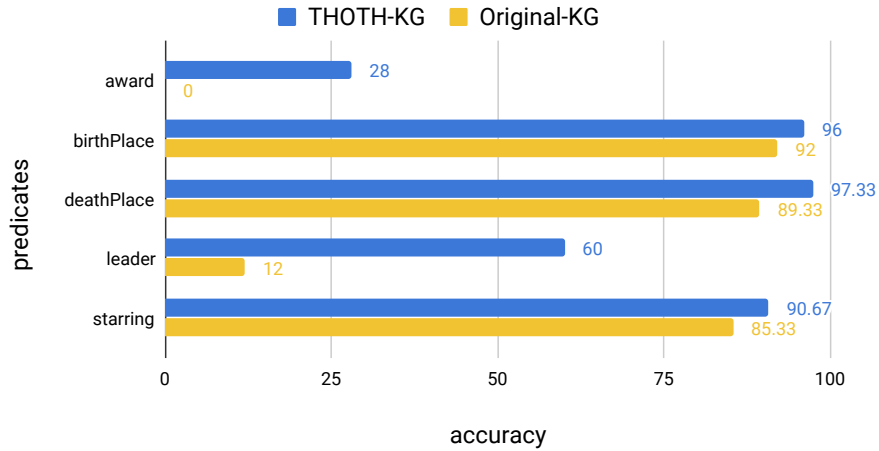

Fig. 4: A comparison between the enriched-German DBpedia (THOTH) KG with the original German DBpedia on the validation of facts.

**Entity Linking results.** For this evaluation, we used the optimal parameter configuration for MAG described by Moussallem et al. [29]. Table 2 reports the results of MAG in two configuration sets, one with original German DBpedia and another with the *Enriched-German DBpedia (THOTH)* as reference KGs. The version of MAG running on the translated KG achieves significantly better results than that running on the original KG. The average improvement across all datasets is around 19% in F-measure. The results of the *German abstracts* data set and *N<sup>3</sup> news.de* are surprisingly high. We sampled the results manually, and we could establish that the results were correct. We also investigated the creation of both benchmarking datasets, and we concluded that at the time of their creation, the links used in both were based on the English DBpedia as an auxiliary KG. Therefore, when THOTH translated the English KG to German and enriched the original German DBpedia with English knowledge, MAG was able to get very high HITS scores for many resources. For example, the HITS score of *dbr\_de:Frankreich (dbr:France)* increased around 50% from 0.08 to 0.12. The superior results of MAG using the enriched knowledge on the VoXEL datasets (which do not suffer from the aforementioned biases) additionally confirm the pertinence of

Table 2: Micro results in a comparison between German DBpedia KG with Enriched-German DBpedia (THOTH) KG in MAG.

| Datasets               | MAG-DBpedia-KG |           |        | MAG-THOTH-KG |             |             |
|------------------------|----------------|-----------|--------|--------------|-------------|-------------|
|                        | F-measure      | Precision | Recall | F-measure    | Precision   | Recall      |
| German Abstracts       | 0.78           | 0.79      | 0.76   | <b>0.97</b>  | <b>0.99</b> | <b>0.96</b> |
| N <sup>3</sup> news.de | 0.77           | 0.78      | 0.76   | <b>0.98</b>  | <b>0.99</b> | <b>0.97</b> |
| VoxEL-strict           | 0.40           | 0.46      | 0.35   | <b>0.70</b>  | <b>0.81</b> | <b>0.61</b> |
| VoxEL-relaxed          | 0.57           | 0.57      | 0.57   | <b>0.64</b>  | <b>0.64</b> | <b>0.64</b> |

THOTH’s results. Finally, we answer **Q3** with the EL results, as they proved that MAG while using the *Enriched-German DBpedia (THOTH)* KG achieved an improvement of +19% F<sub>1</sub> in comparison to the original German DBpedia.

#### 5.4 Error Analysis and Discussion

In this section, we report findings and some problems found in THOTH. One of the outcomes came about while analyzing the significant drop in the translation triple accuracy shown in the overall results. We examined the translations manually and perceived that the accuracy mainly decreased because THOTH was capable of generating disambiguated URIs instead of the correct ones. For example, the following triple in the reference translation `<dbr_de:don_getty dbo:birthplace dbr_de:westmount>` did not match with the following output, `<dbr_de:don_getty dbo:birthplace dbr_de:westmount_(québec)>`, simply because THOTH generated a different object URI. Although the output object has a different URI, it is correct because the birthplace of Don Getty was Westmount in Québec. However, this more explicit URI led to an error and consequently decreased the translation accuracy. It is a fascinating example because we could see that the NN models along with the KGE were able to understand the KGs graph structure and predict a disambiguated URI based on the knowledge from the English DBpedia. Additionally, no similar example was present in the training set, indicating that the BPE model learned correctly to translate the URIs.

Besides the aforementioned results, we noticed some mistranslations of similar predicates which were responsible for decreasing the accuracy of triple translation. For example, the following English source triple `dbr:zenyattà_mondatta dbo:artist dbr:the_police` was translated into `dbr_de:zenyattà_mondatta dbo:producer dbr_de:the_police`. This example shows that THOTH translated the subject and object correctly. However, the predicate was incorrect and was mistranslated from `dbo:artist` to `dbo:producer`. A similar problem occurred while translating the triple, `dbr:albert_einstein dbo:citizenship dbr:Switzerland` to `dbr:albert_einstein dbo:birthplace dbr:der_Schweiz`. After a manual analysis, we identified that both cases happened because THOTH could not distinguish the predicates which share the same domain and range. In a more in-depth analysis, we perceived that the predicates mentioned above are very close to each other in the vector space thus complicating the disambiguation process of NN models. The

performance of THOTH was not affected by these false triples since they were automatically removed from the *Enriched-German DBpedia (THOTH)* dataset in the enrichment step. After this manual analysis of the results, we believe that addressing the problem of similar predicates (e.g., through novel embedding techniques) can enhance the translation quality of THOTH.

## 6 Conclusion

In this paper, we introduced a neural approach named THOTH for translating and enriching KGs from different languages. THOTH relies on two different RNN-based NMT models along with KGEs for translating triples and texts jointly. We carried out an extensive evaluation set for certifying the quality of our approach. Our results show that THOTH is a promising approach which achieves a translation accuracy of 88.56%. Moreover, its enrichment improves the quality of the German DBpedia significantly, as we report +18.4% accuracy for fact validation and +19%  $F_1$  for entity linking. As future work, we plan to investigate the application of sub-graphs [10] for improving the disambiguation of similar predicates. Additionally, we aim to exploit other NN architectures, such as Transformer [38], for improving THOTH's performance. Moreover, we plan to apply THOTH in the context of low-resource KG scenarios with Asian and African languages as well as apply THOTH on the Wikidata KG.

## Acknowledgments

This work has been supported by the German Federal Ministry of Transport and Digital Infrastructure (BMVI) in the projects LIMBO (no. 19F2029I) and OPAL (no. 19F2028A) as well as by the Brazilian National Council for Scientific and Technological Development (CNPq) (no. 206971/2014-1)

## References

1. Aposio, A.P., Giuliano, C., Lavelli, A.: Towards an automatic creation of localized versions of dbpedia. In: International Semantic Web Conference. pp. 494–509. Springer (2013)
2. Arcan, M., Buitelaar, P.: Ontology Label Translation. In: HLT-NAACL. pp. 40–46 (2013)
3. Arcan, M., Buitelaar, P.: Translating domain-specific expressions in knowledge bases with neural machine translation. arXiv preprint arXiv:1709.02184 (2017)
4. Auer, S., Bizer, C., Kobilarov, G., Lehmann, J., Cyganiak, R., Ives, Z.: Dbpedia: A nucleus for a web of open data. In: The semantic web, pp. 722–735. Springer (2007)
5. Bahdanau, D., Cho, K., Bengio, Y.: Neural machine translation by jointly learning to align and translate. arXiv preprint arXiv:1409.0473 (2014)
6. Böhning, D.: Multinomial logistic regression algorithm. *Annals of the institute of Statistical Mathematics* **1**, 197–200 (1992)
7. Bollacker, K., Evans, C., Paritosh, P., Sturge, T., Taylor, J.: Freebase: a collaboratively created graph database for structuring human knowledge. In: Proceedings of the 2008 ACM SIGMOD international conference on Management of data. pp. 1247–1250. AcM (2008)

8. Bordes, A., Usunier, N., Garcia-Duran, A., Weston, J., Yakhnenko, O.: Translating embeddings for modeling multi-relational data. In: *Advances in Neural Information Processing Systems*. pp. 2787–2795 (2013)
9. Brümmer, M., Dojchinovski, M., Hellmann, S.: Dbpedia abstracts: A large-scale, open, multilingual nlp training corpus. In: *Proceedings of the Tenth International Conference on Language Resources and Evaluation (LREC 2016)*. European Language Resources Association (ELRA), Paris, France (May 2016)
10. Cao, Z., Wang, L., de Melo, G.: Link prediction via subgraph embedding-based convex matrix completion. In: *Proceedings of the 32nd AAAI Conference on Artificial Intelligence (AAAI 2018)*. AAAI Press (2018)
11. Chen, M., Tian, Y., Yang, M., Zaniolo, C.: Multilingual knowledge graph embeddings for cross-lingual knowledge alignment. In: *Proceedings of the 26th International Joint Conference on Artificial Intelligence*. pp. 1511–1517. AAAI Press (2017)
12. Chen, M., Tian, Y., Yang, M., Zaniolo, C.: Multilingual Knowledge Graph Embeddings for Cross-lingual Knowledge Alignment. In: *Proceedings of the 26th International Joint Conference on Artificial Intelligence (IJCAI)*. pp. 1–10. AAAI Press (2017)
13. Cochez, M., Ristoski, P., Ponzetto, S.P., Paulheim, H.: Biased graph walks for rdf graph embeddings. In: *Proceedings of the 7th International Conference on Web Intelligence, Mining and Semantics*. p. 21. ACM (2017)
14. Cochez, M., Ristoski, P., Ponzetto, S.P., Paulheim, H.: Global rdf vector space embeddings. In: *International Semantic Web Conference*. pp. 190–207. Springer (2017)
15. Edunov, S., Ott, M., Auli, M., Grangier, D.: Understanding back-translation at scale. *arXiv preprint arXiv:1808.09381* (2018)
16. Feng, X., Tang, D., Qin, B., Liu, T.: English-chinese knowledge base translation with neural network. In: *Proceedings of COLING 2016, the 26th International Conference on Computational Linguistics: Technical Papers*. pp. 2935–2944 (2016)
17. Gerber, D., Esteves, D., Lehmann, J., Böhmann, L., Usbeck, R., Ngomo, A.C.N., Speck, R.: Defacto temporal and multilingual deep fact validation. *Web Semantics: Science, Services and Agents on the World Wide Web* **35**, 85–101 (2015)
18. Joulin, A., Grave, E., Bojanowski, P., Mikolov, T.: Bag of tricks for efficient text classification. In: *Proceedings of the 15th Conference of the European Chapter of the Association for Computational Linguistics: Volume 2, Short Papers*. vol. 2, pp. 427–431 (2017)
19. Joulin, A., Grave, E., Bojanowski, P., Nickel, M., Mikolov, T.: Fast linear model for knowledge graph embeddings. *arXiv preprint arXiv:1710.10881* (2017)
20. K M, A., Basu Roy Chowdhury, S., Dukkupati, A.: Learning beyond datasets: Knowledge graph augmented neural networks for natural language processing. In: *Proceedings of the 2018 Conference of the North American Chapter of the Association for Computational Linguistics: Human Language Technologies, Volume 1 (Long Papers)*. pp. 313–322. Association for Computational Linguistics (2018), <http://aclweb.org/anthology/N18-1029>
21. Kaffee, L.A., Elsahar, H., Vougiouklis, P., Gravier, C., Laforest, F., Hare, J., Simperl, E.: Mind the (language) gap: generation of multilingual wikipedia summaries from wikidata for articleplaceholders. In: *European Semantic Web Conference*. pp. 319–334. Springer (2018)
22. Kalchbrenner, N., Blunsom, P.: Recurrent Continuous Translation Models. In: *EMNLP*. vol. 3, p. 413 (2013)
23. Klein, G., Kim, Y., Deng, Y., Senellart, J., Rush, A.M.: OpenNMT: Open-Source Toolkit for Neural Machine Translation. *ArXiv e-prints* (2017)
24. Klein, G., Kim, Y., Deng, Y., Senellart, J., Rush, A.: Opennmt: Open-source toolkit for neural machine translation. *Proceedings of ACL 2017, System Demonstrations* pp. 67–72 (2017)



25. Lakshen, G.A., Janev, V., Vraneš, S.: Challenges in quality assessment of arabic dbpedia. In: Proceedings of the 8th International Conference on Web Intelligence, Mining and Semantics. p. 15. ACM (2018)
26. Luong, T., Pham, H., Manning, C.D.: Effective approaches to attention-based neural machine translation. In: Proceedings of the 2015 Conference on Empirical Methods in Natural Language Processing. pp. 1412–1421. Association for Computational Linguistics (2015). <https://doi.org/10.18653/v1/D15-1166>, <http://aclweb.org/anthology/D15-1166>
27. McCrae, J.P., Arcan, M., Asooja, K., Gracia, J., Buitelaar, P., Cimiano, P.: Domain adaptation for ontology localization. *Web Semantics: Science, Services and Agents on the World Wide Web* **36**, 23–31 (2016)
28. Moussallem, D., Arčan, M., Ngomo, A.C.N., Buitelaar, P.: Augmenting neural machine translation with knowledge graphs. *arXiv preprint arXiv:1902.08816* (2019)
29. Moussallem, D., Usbeck, R., Röeder, M., Ngomo, A.C.N.: MAG: A Multilingual, Knowledge-base Agnostic and Deterministic Entity Linking Approach. In: Proceedings of the Knowledge Capture Conference. p. 9. ACM (2017)
30. Moussallem, D., Wauer, M., Ngomo, A.C.N.: Machine translation using semantic web technologies: A survey. *Journal of Web Semantics* **51**, 1–19 (2018)
31. Nickel, M., Rosasco, L., Poggio, T.A., et al.: Holographic embeddings of knowledge graphs. In: AAAI. pp. 1955–1961 (2016)
32. Papineni, K., Roukos, S., Ward, T., Zhu, W.J.: BLEU: a method for automatic evaluation of machine translation. In: Proceedings of the 40th annual meeting on association for computational linguistics. pp. 311–318. Association for Computational Linguistics (2002)
33. Ristoski, P., Paulheim, H.: Rdf2vec: Rdf graph embeddings for data mining. In: International Semantic Web Conference. pp. 498–514. Springer (2016)
34. Sennrich, R., Haddow, B., Birch, A.: Neural machine translation of rare words with subword units. In: Proceedings of the 54th Annual Meeting of the Association for Computational Linguistics (Volume 1: Long Papers). pp. 1715–1725. Association for Computational Linguistics (2016)
35. Sorokin, D., Gurevych, I.: Modeling semantics with gated graph neural networks for knowledge base question answering. In: Proceedings of the 27th International Conference on Computational Linguistics. pp. 3306–3317. Association for Computational Linguistics (2018), <http://aclweb.org/anthology/C18-1280>
36. Tang, G., Müller, M., Rios, A., Sennrich, R.: Why self-attention? a targeted evaluation of neural machine translation architectures. In: Proceedings of the 2018 Conference on Empirical Methods in Natural Language Processing. pp. 4263–4272 (2018)
37. Usbeck, R., Röder, M., Ngomo, A.N., Baron, C., Both, A., Brümmer, M., Ceccarelli, D., Cornolti, M., Cherix, D., Eickmann, B., Ferragina, P., Lemke, C., Moro, A., Navigli, R., Piccinno, F., Rizzo, G., Sack, H., Speck, R., Troncy, R., Waitelonis, J., Wesemann, L.: GERBIL: general entity annotator benchmarking framework. In: Proceedings of the 24th International Conference on World Wide Web, WWW 2015, Florence, Italy, May 18-22, 2015. pp. 1133–1143. Florence, Italy (2015)
38. Vaswani, A., Shazeer, N., Parmar, N., Uszkoreit, J., Jones, L., Gomez, A.N., Kaiser, Ł., Polosukhin, I.: Attention is all you need. In: Advances in Neural Information Processing Systems. pp. 5998–6008 (2017)
39. Zaveri, A., Rula, A., Maurino, A., Pietrobon, R., Lehmann, J., Auer, S.: Quality assessment for linked data: A survey. *Semantic Web* **7**(1), 63–93 (2016)
