# Supplementary material for: Knowledge Graphs for Multilingual Language Translation and Generation
Source: arXiv:2009.07715 source file (2020-09-16)
Supplement: Supplementary file 10 [file sign.tex]

%\newcommand*\rot{\multicolumn{1}{R{60}{1em}}}% no optional argument here, please
%\chapter*{PUBLICATIONS}
%	\thispagestyle{empty}

% \includepdf[pages=1,pagecommand={\section{\label{appendix:MAG}}}]{appendices/papers/MAG/MAG_to_K_CAP.pdf}
% \includepdf[pages=2-,pagecommand={}]{appendices/papers/MAG/MAG_to_K_CAP.pdf}
\includepdf[pages=1,pagecommand={},trim=0mm 20mm 0mm 0mm]{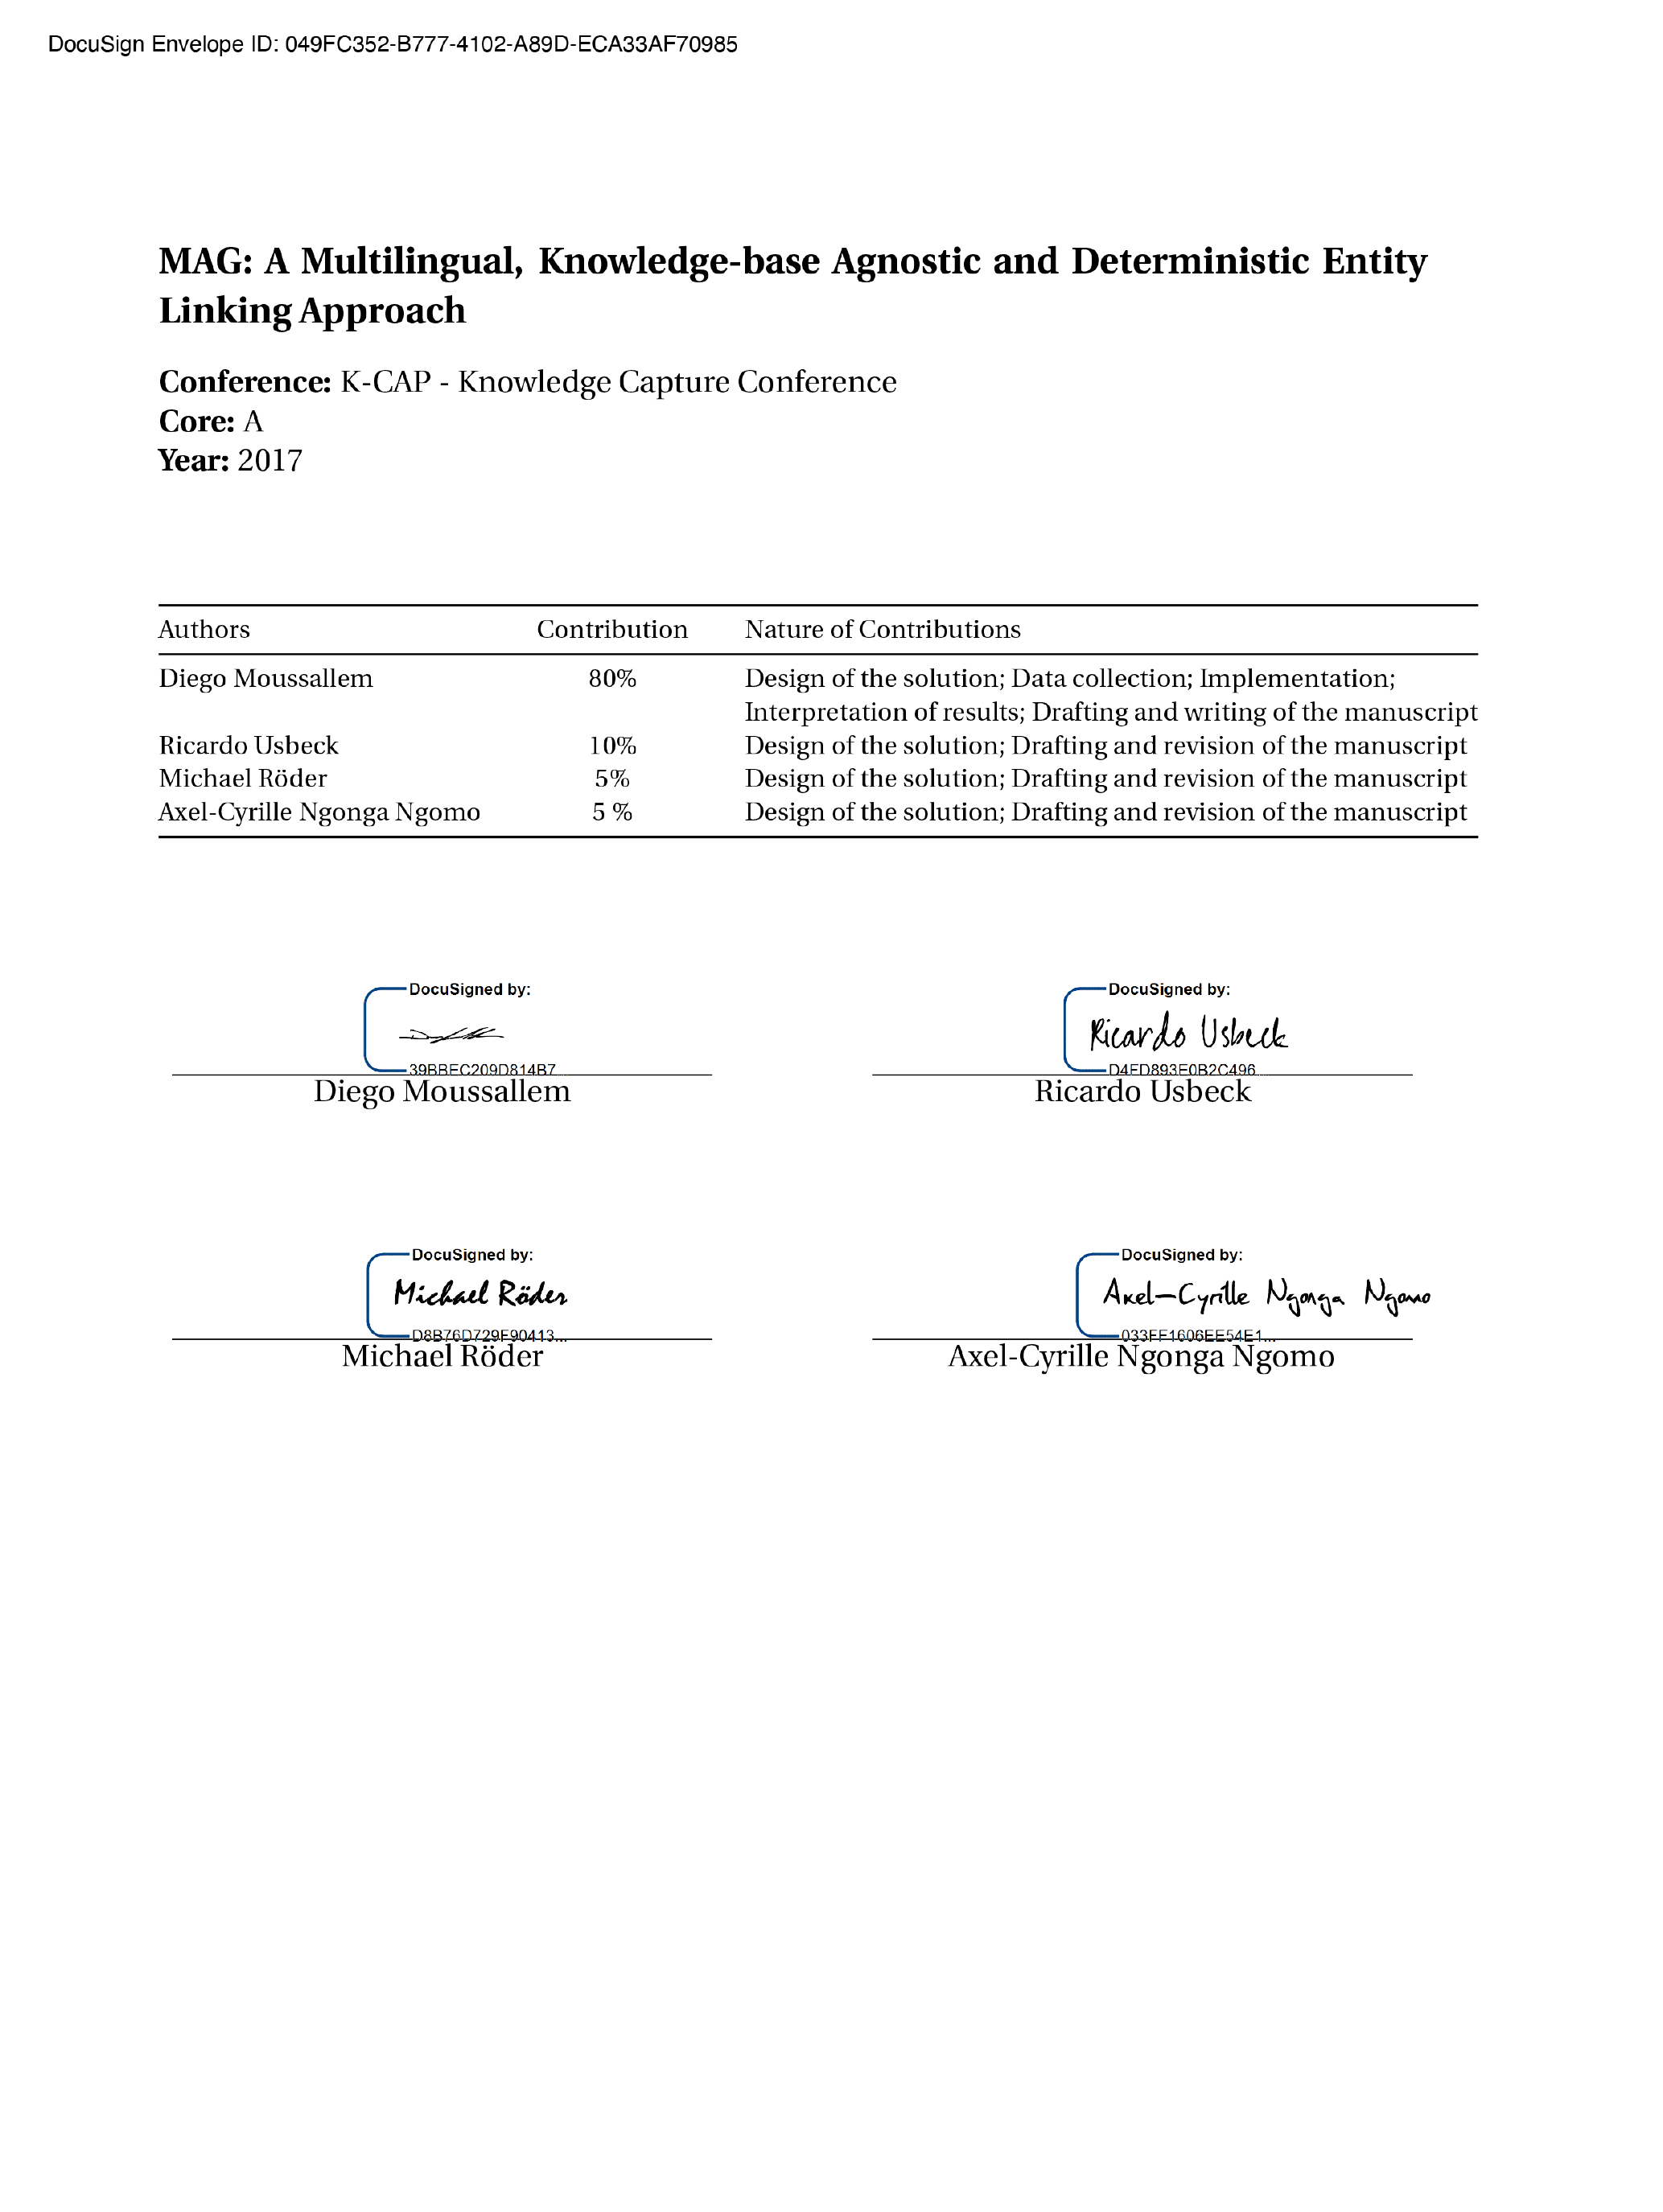}
\includepdf[pages=1,pagecommand={},trim=0mm 20mm 0mm 0mm]{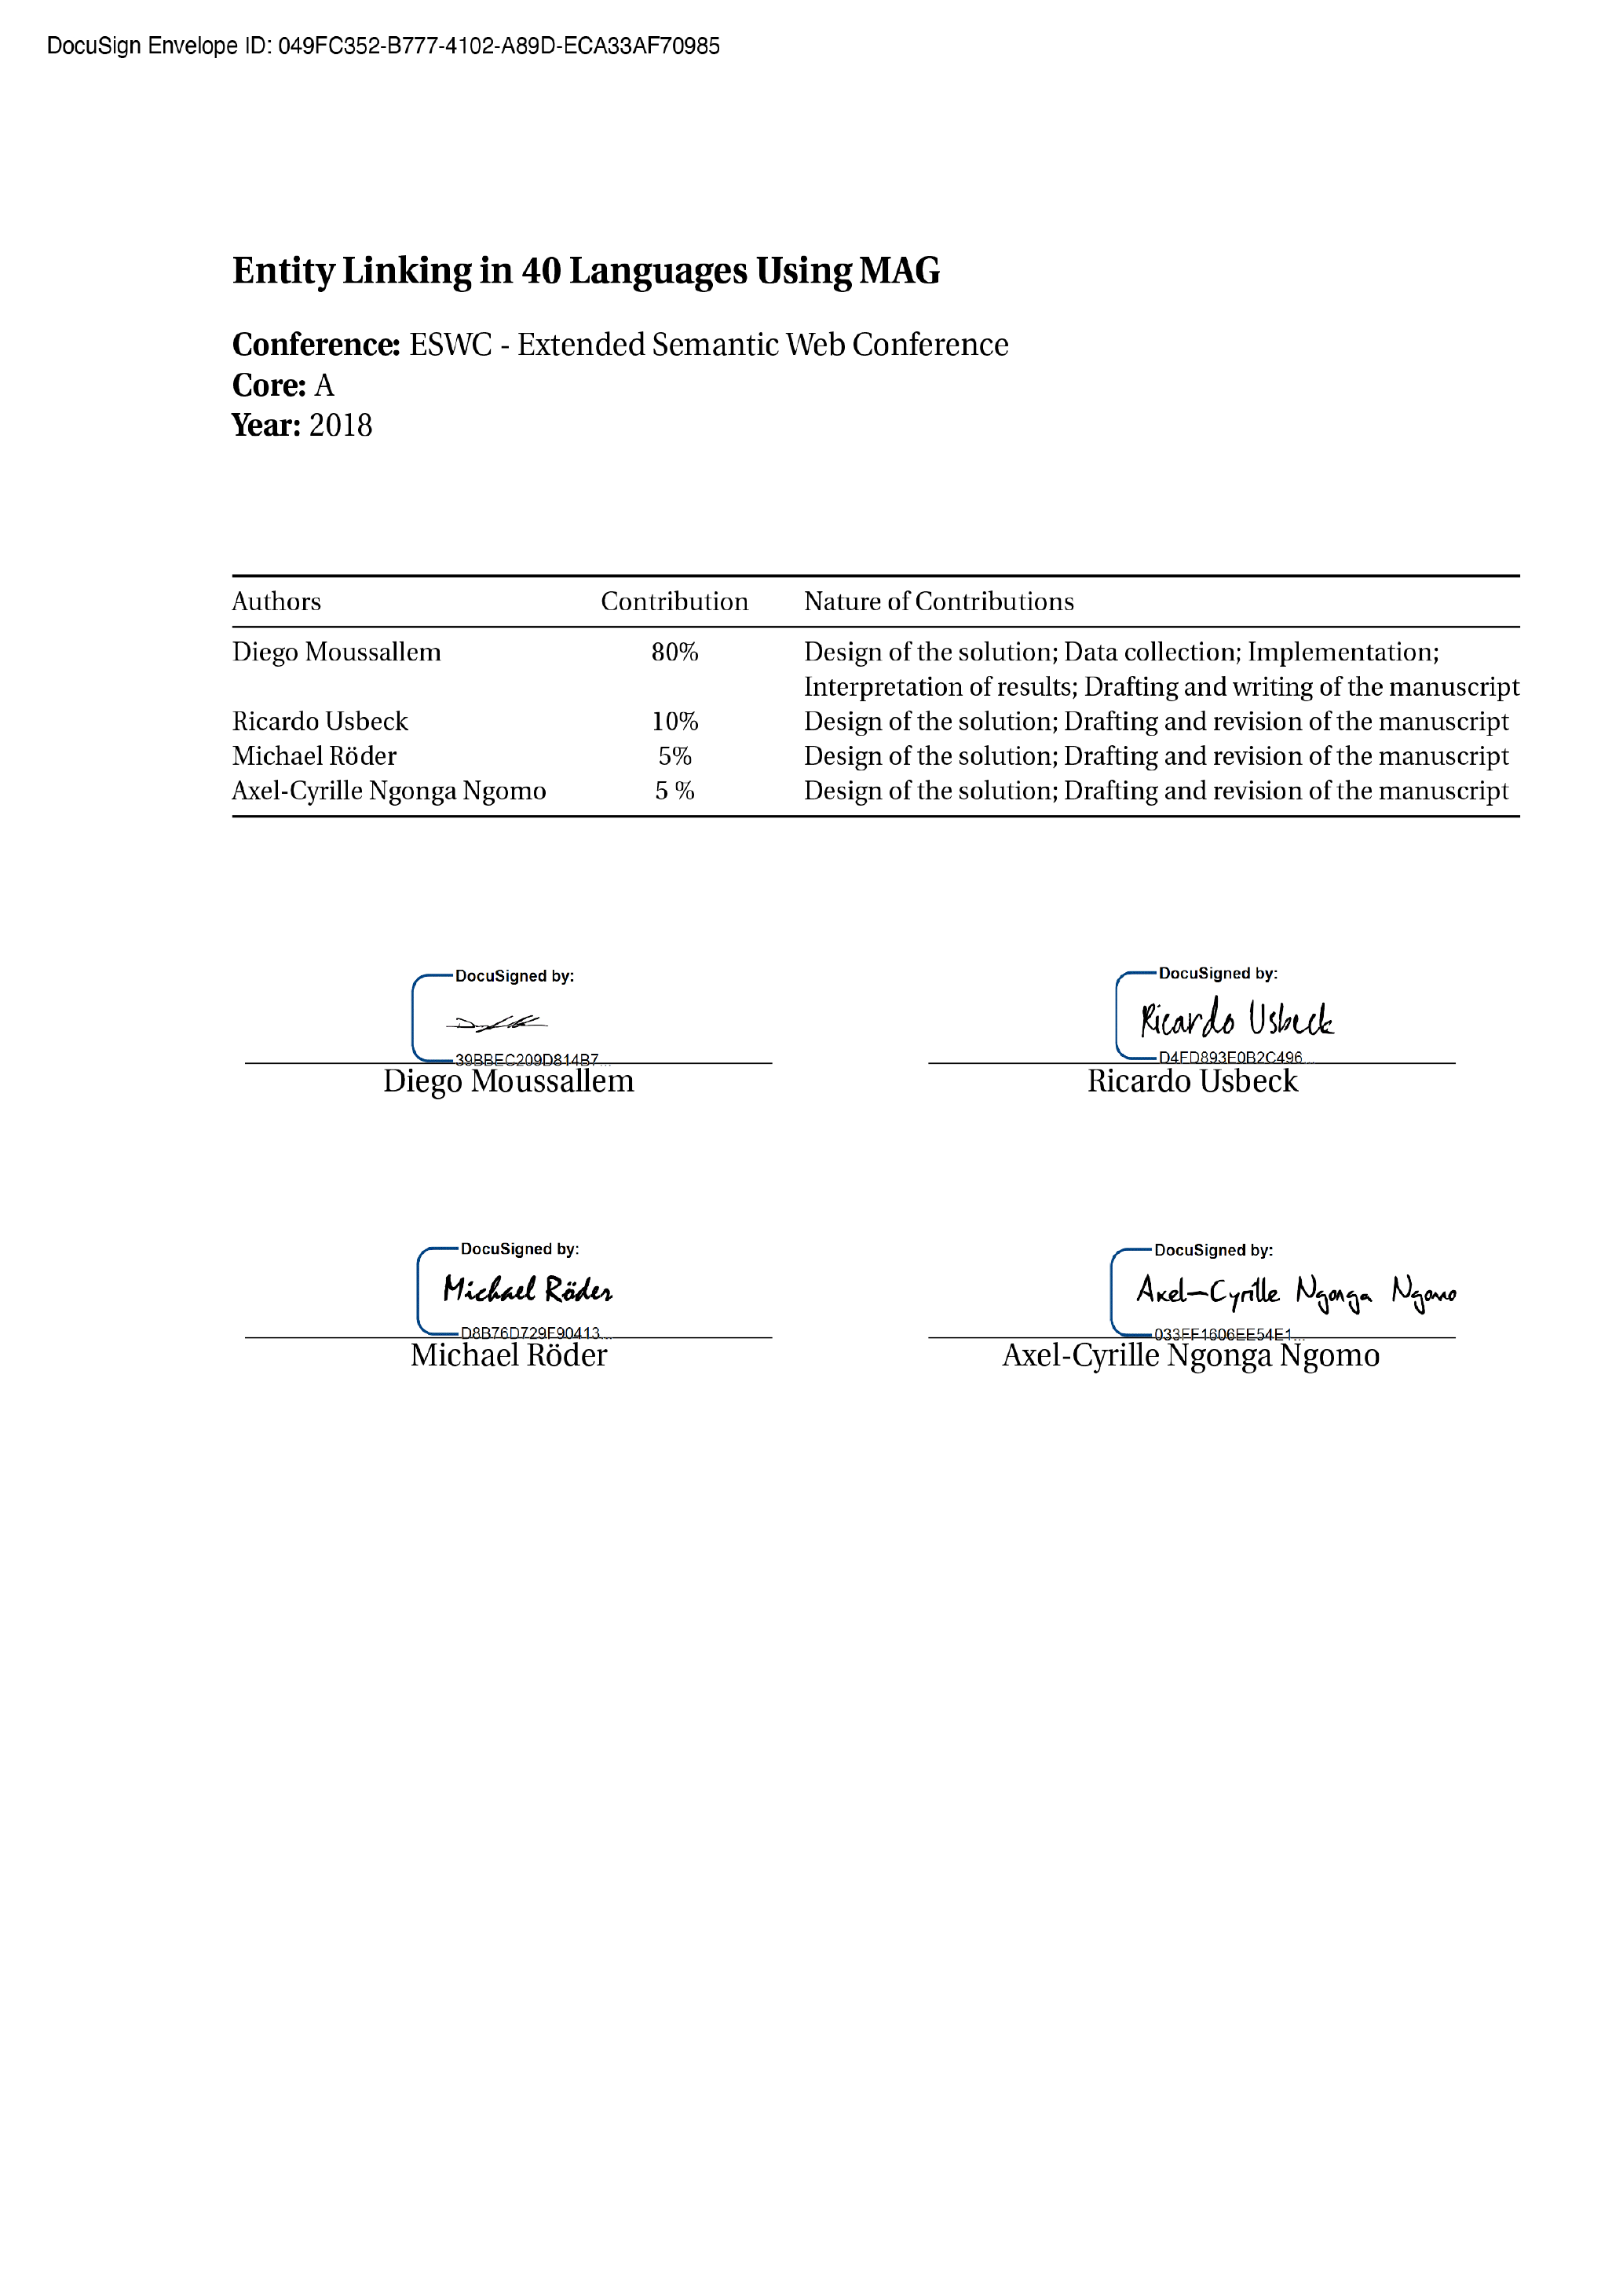}

\includepdf[pages=1,pagecommand={},trim=0mm 20mm 0mm 0mm]{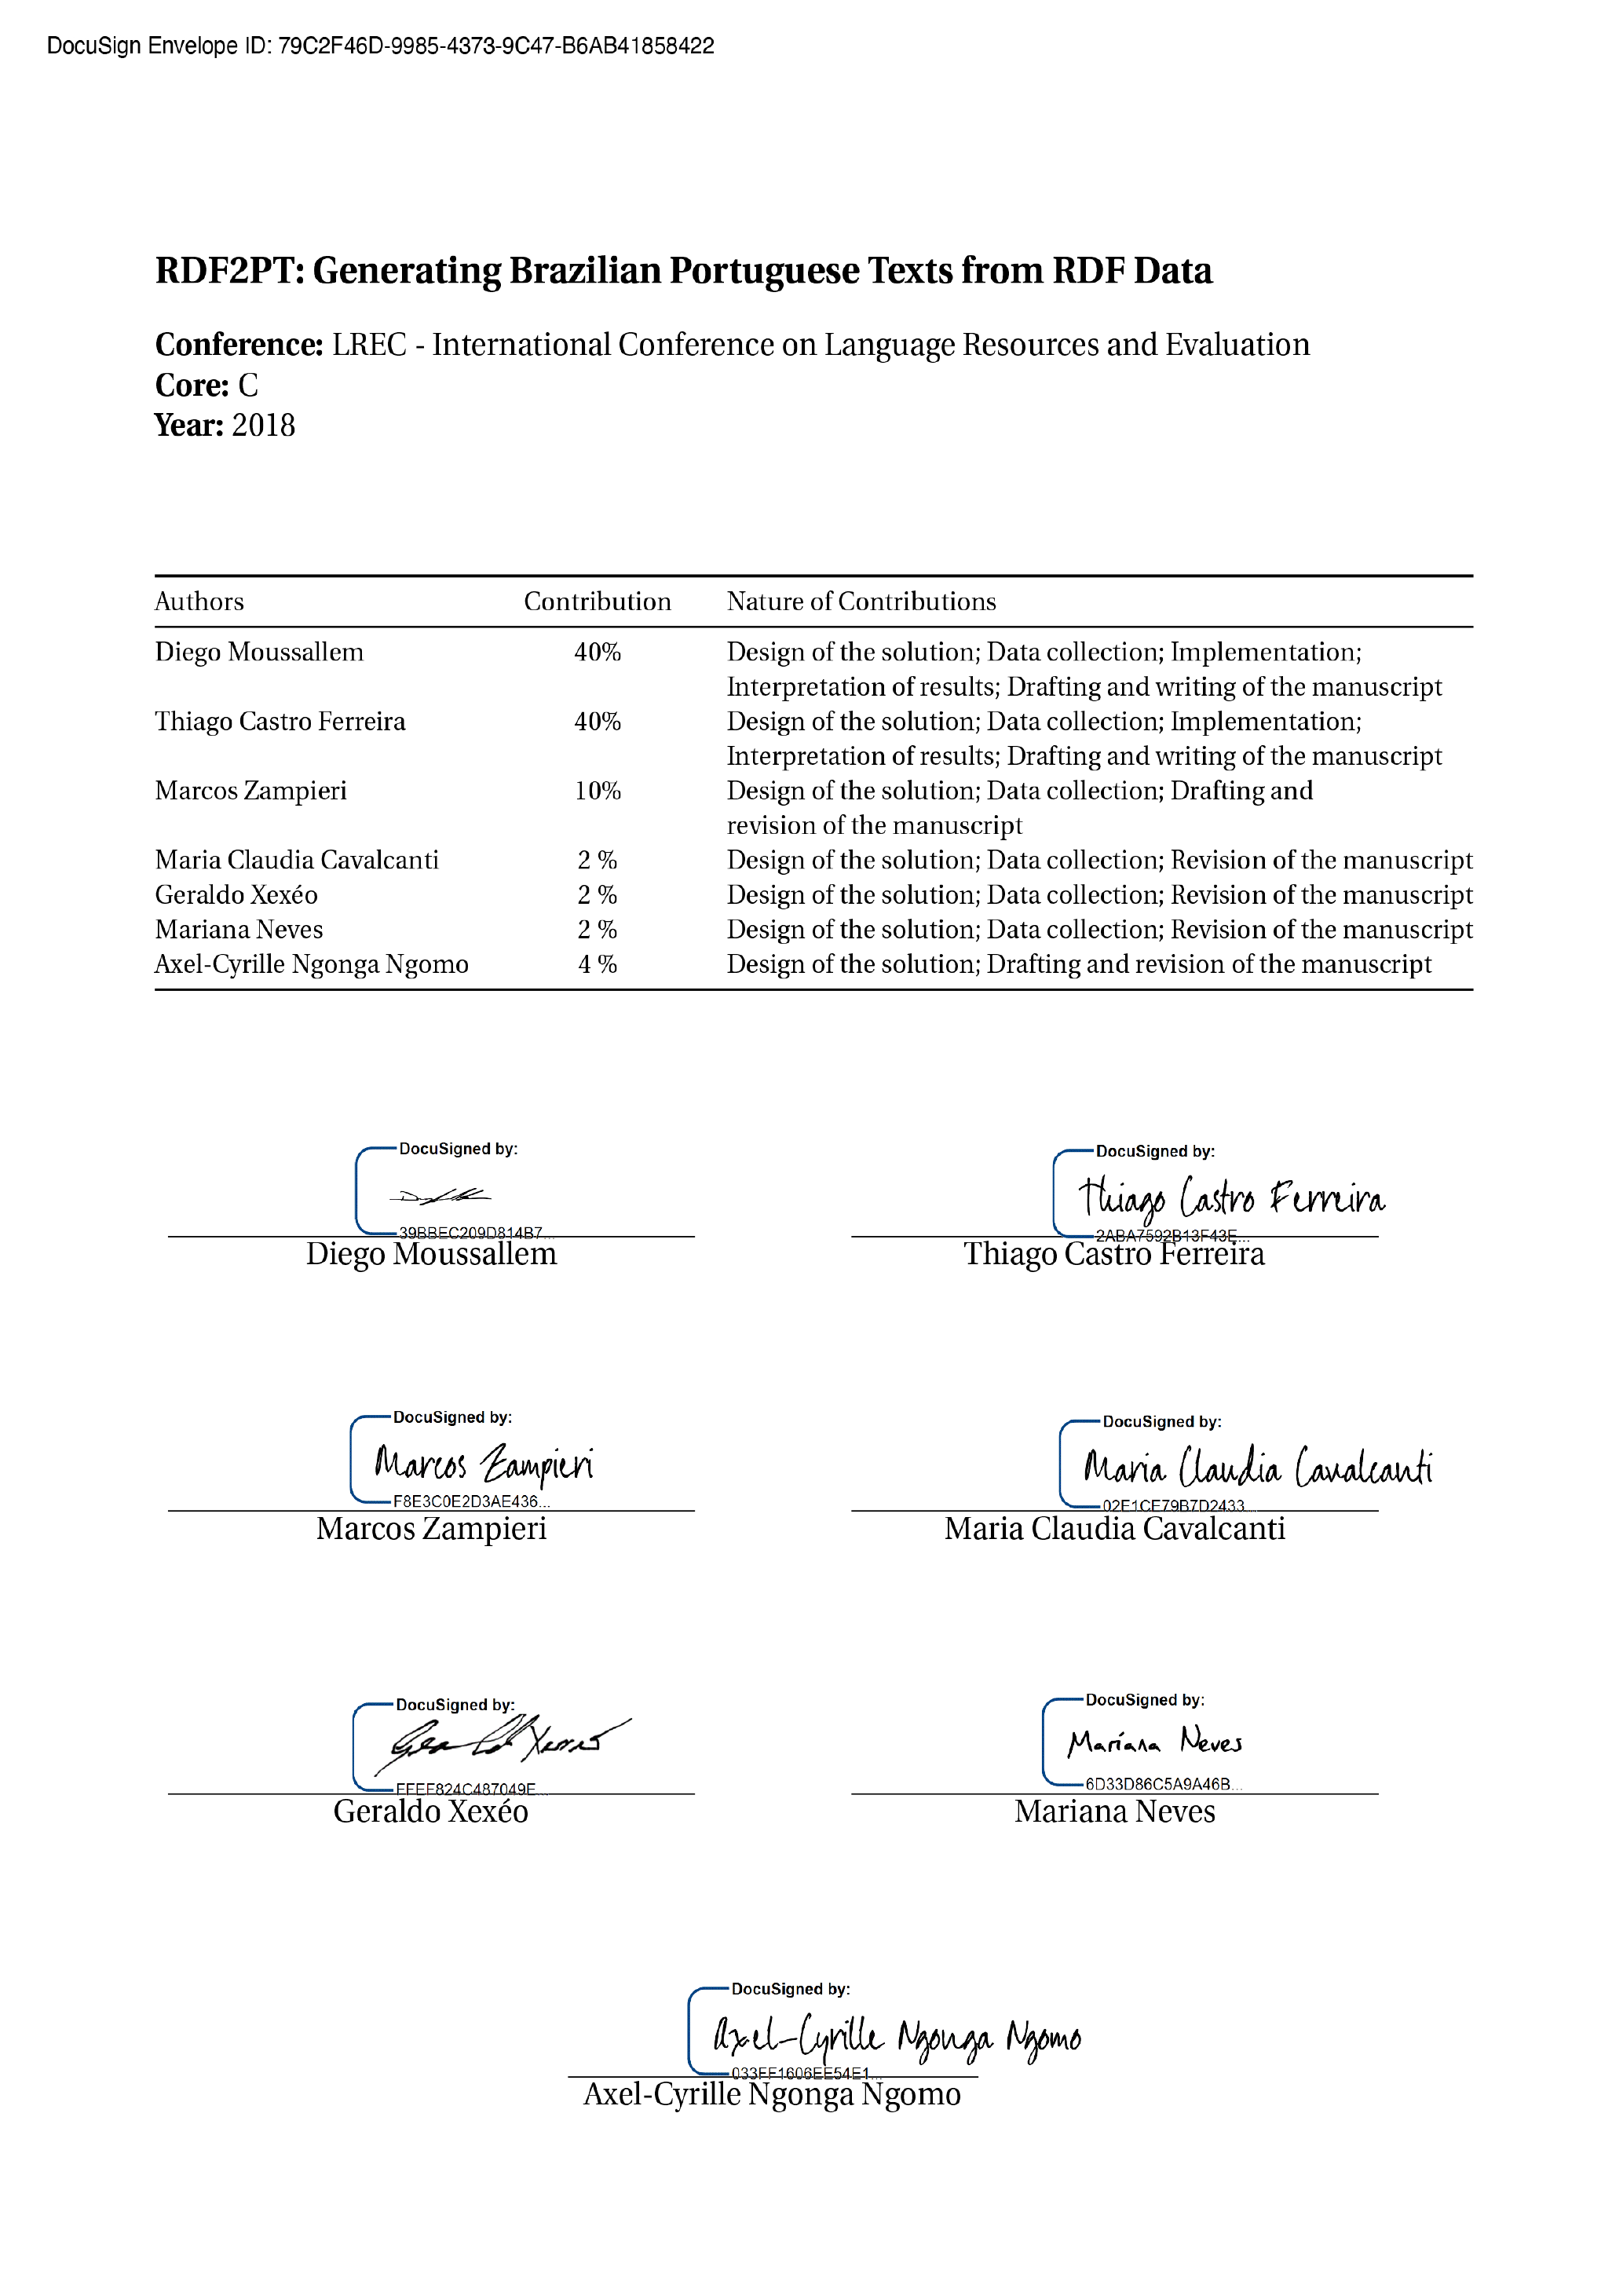}
\includepdf[pages=1,pagecommand={},trim=0mm 20mm 0mm 0mm]{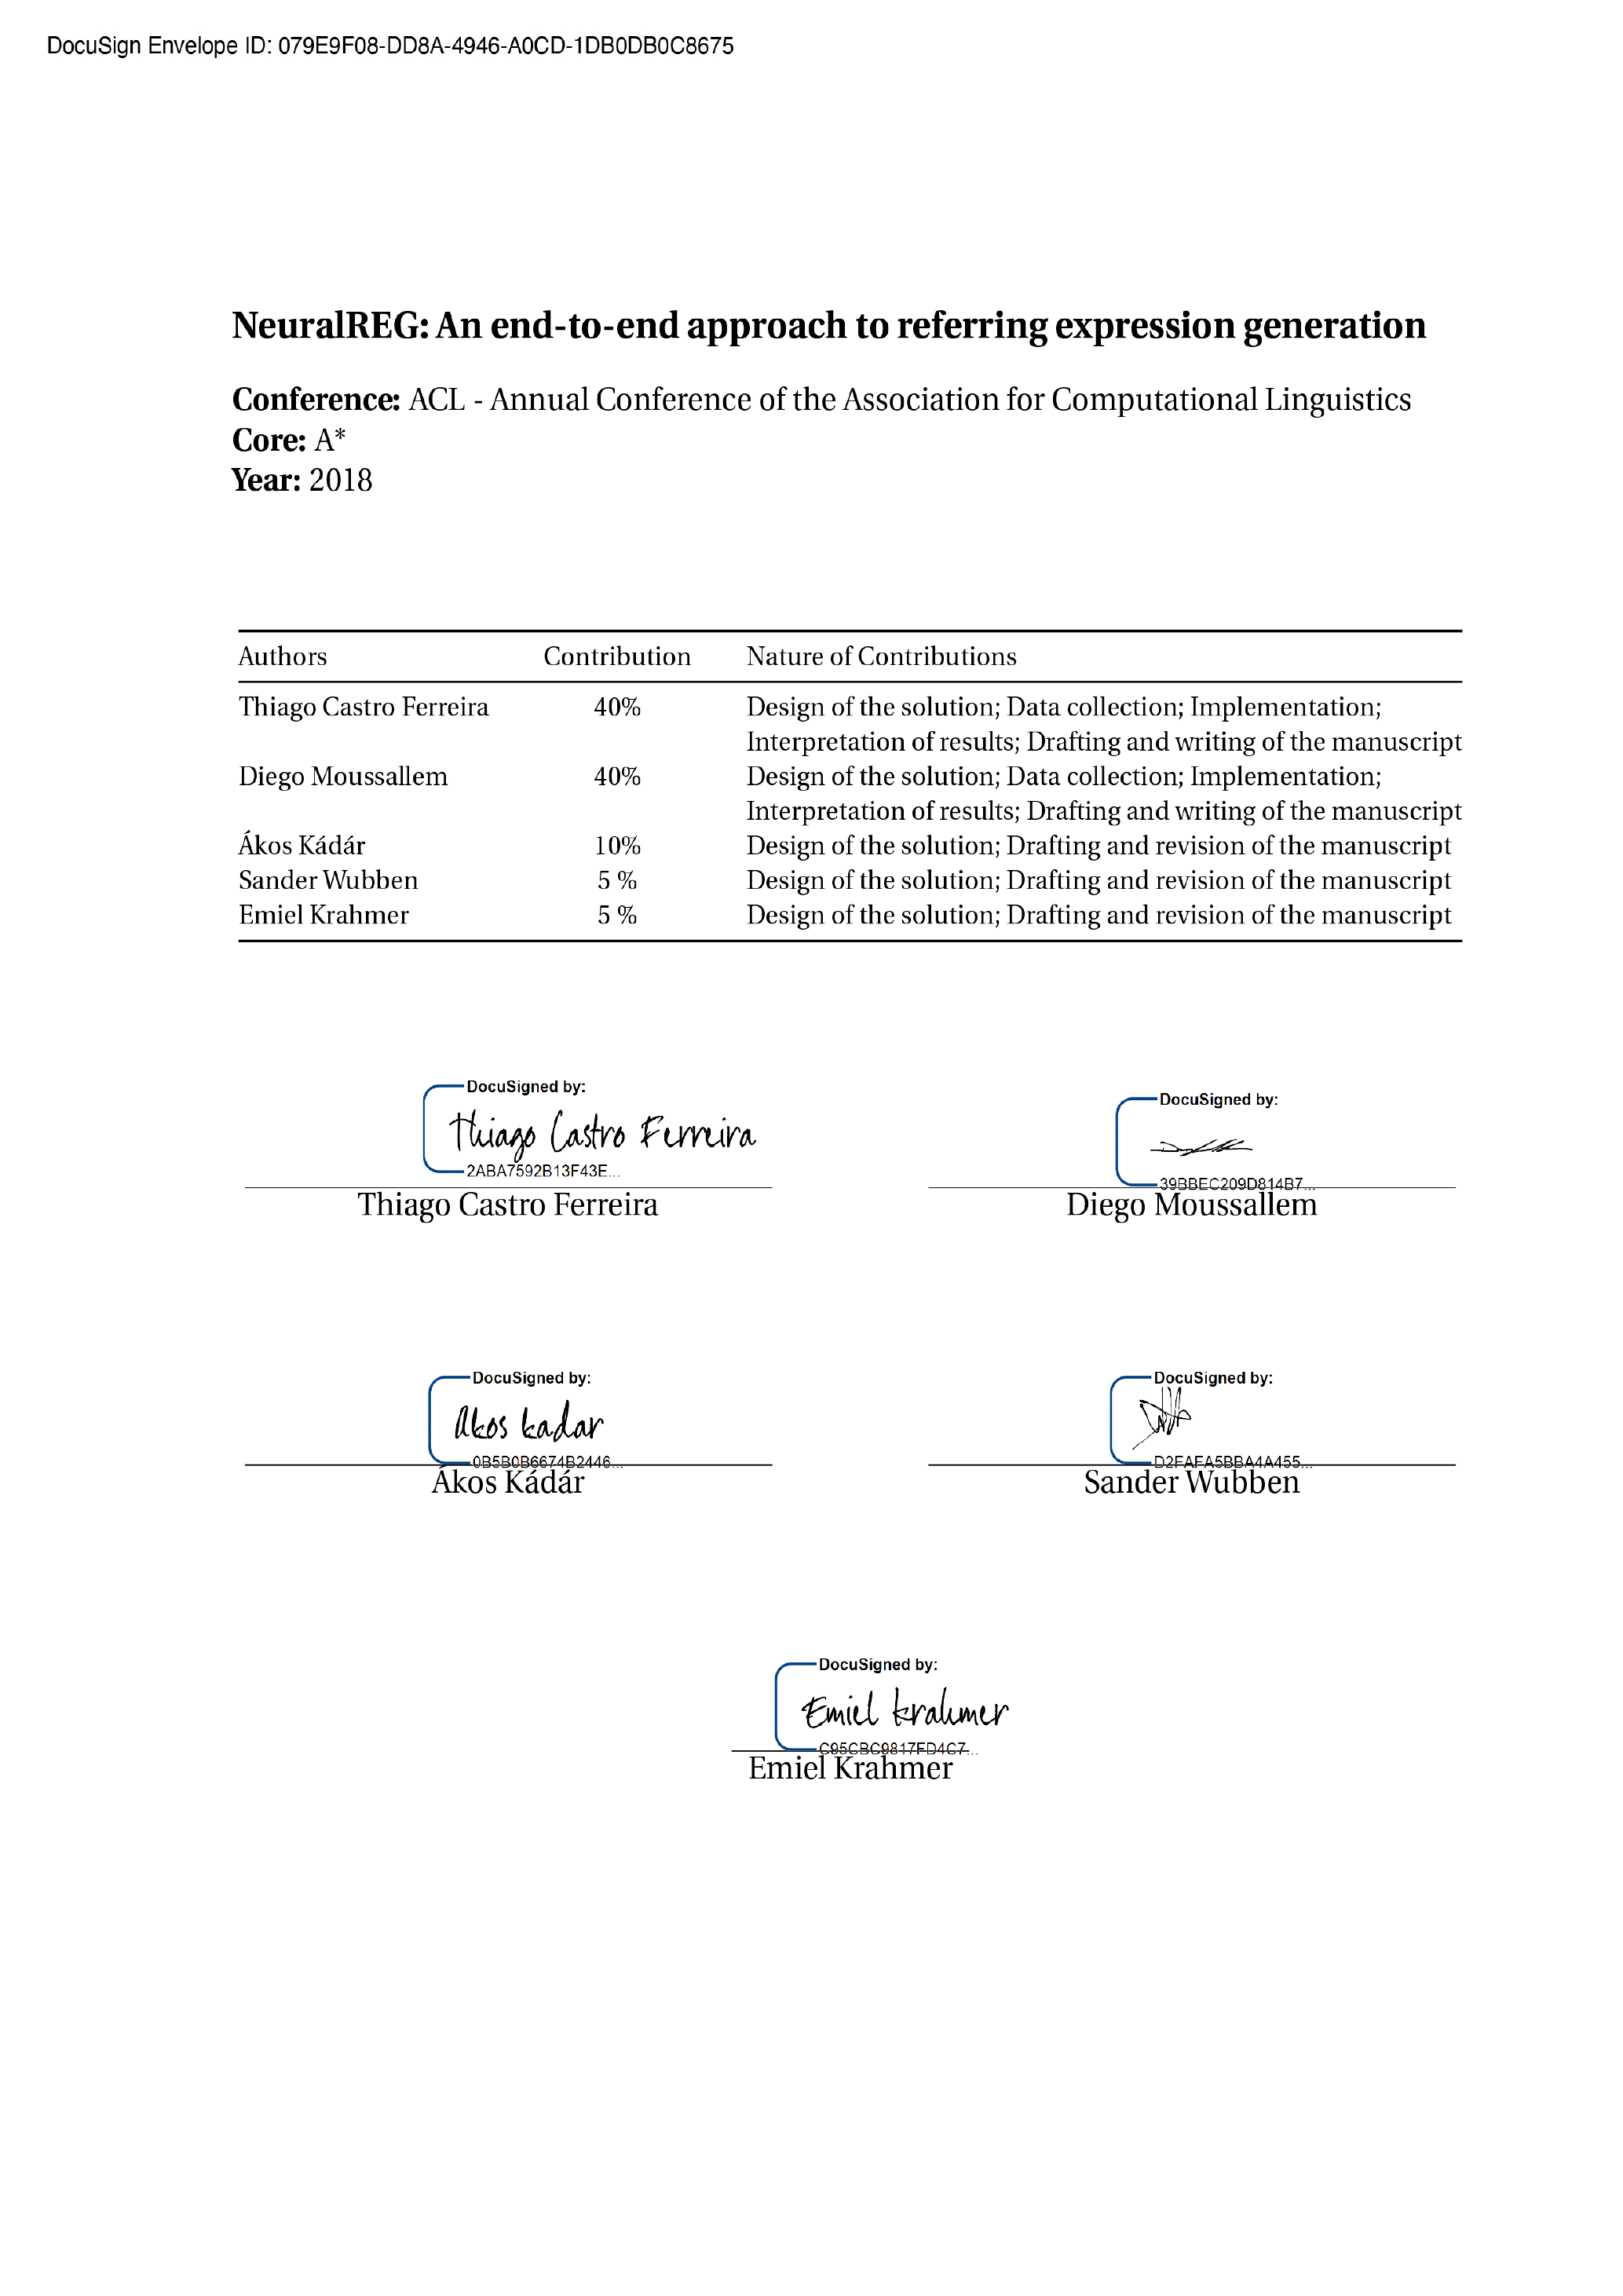}

\includepdf[pages=1,pagecommand={},trim=0mm 20mm 0mm 0mm]{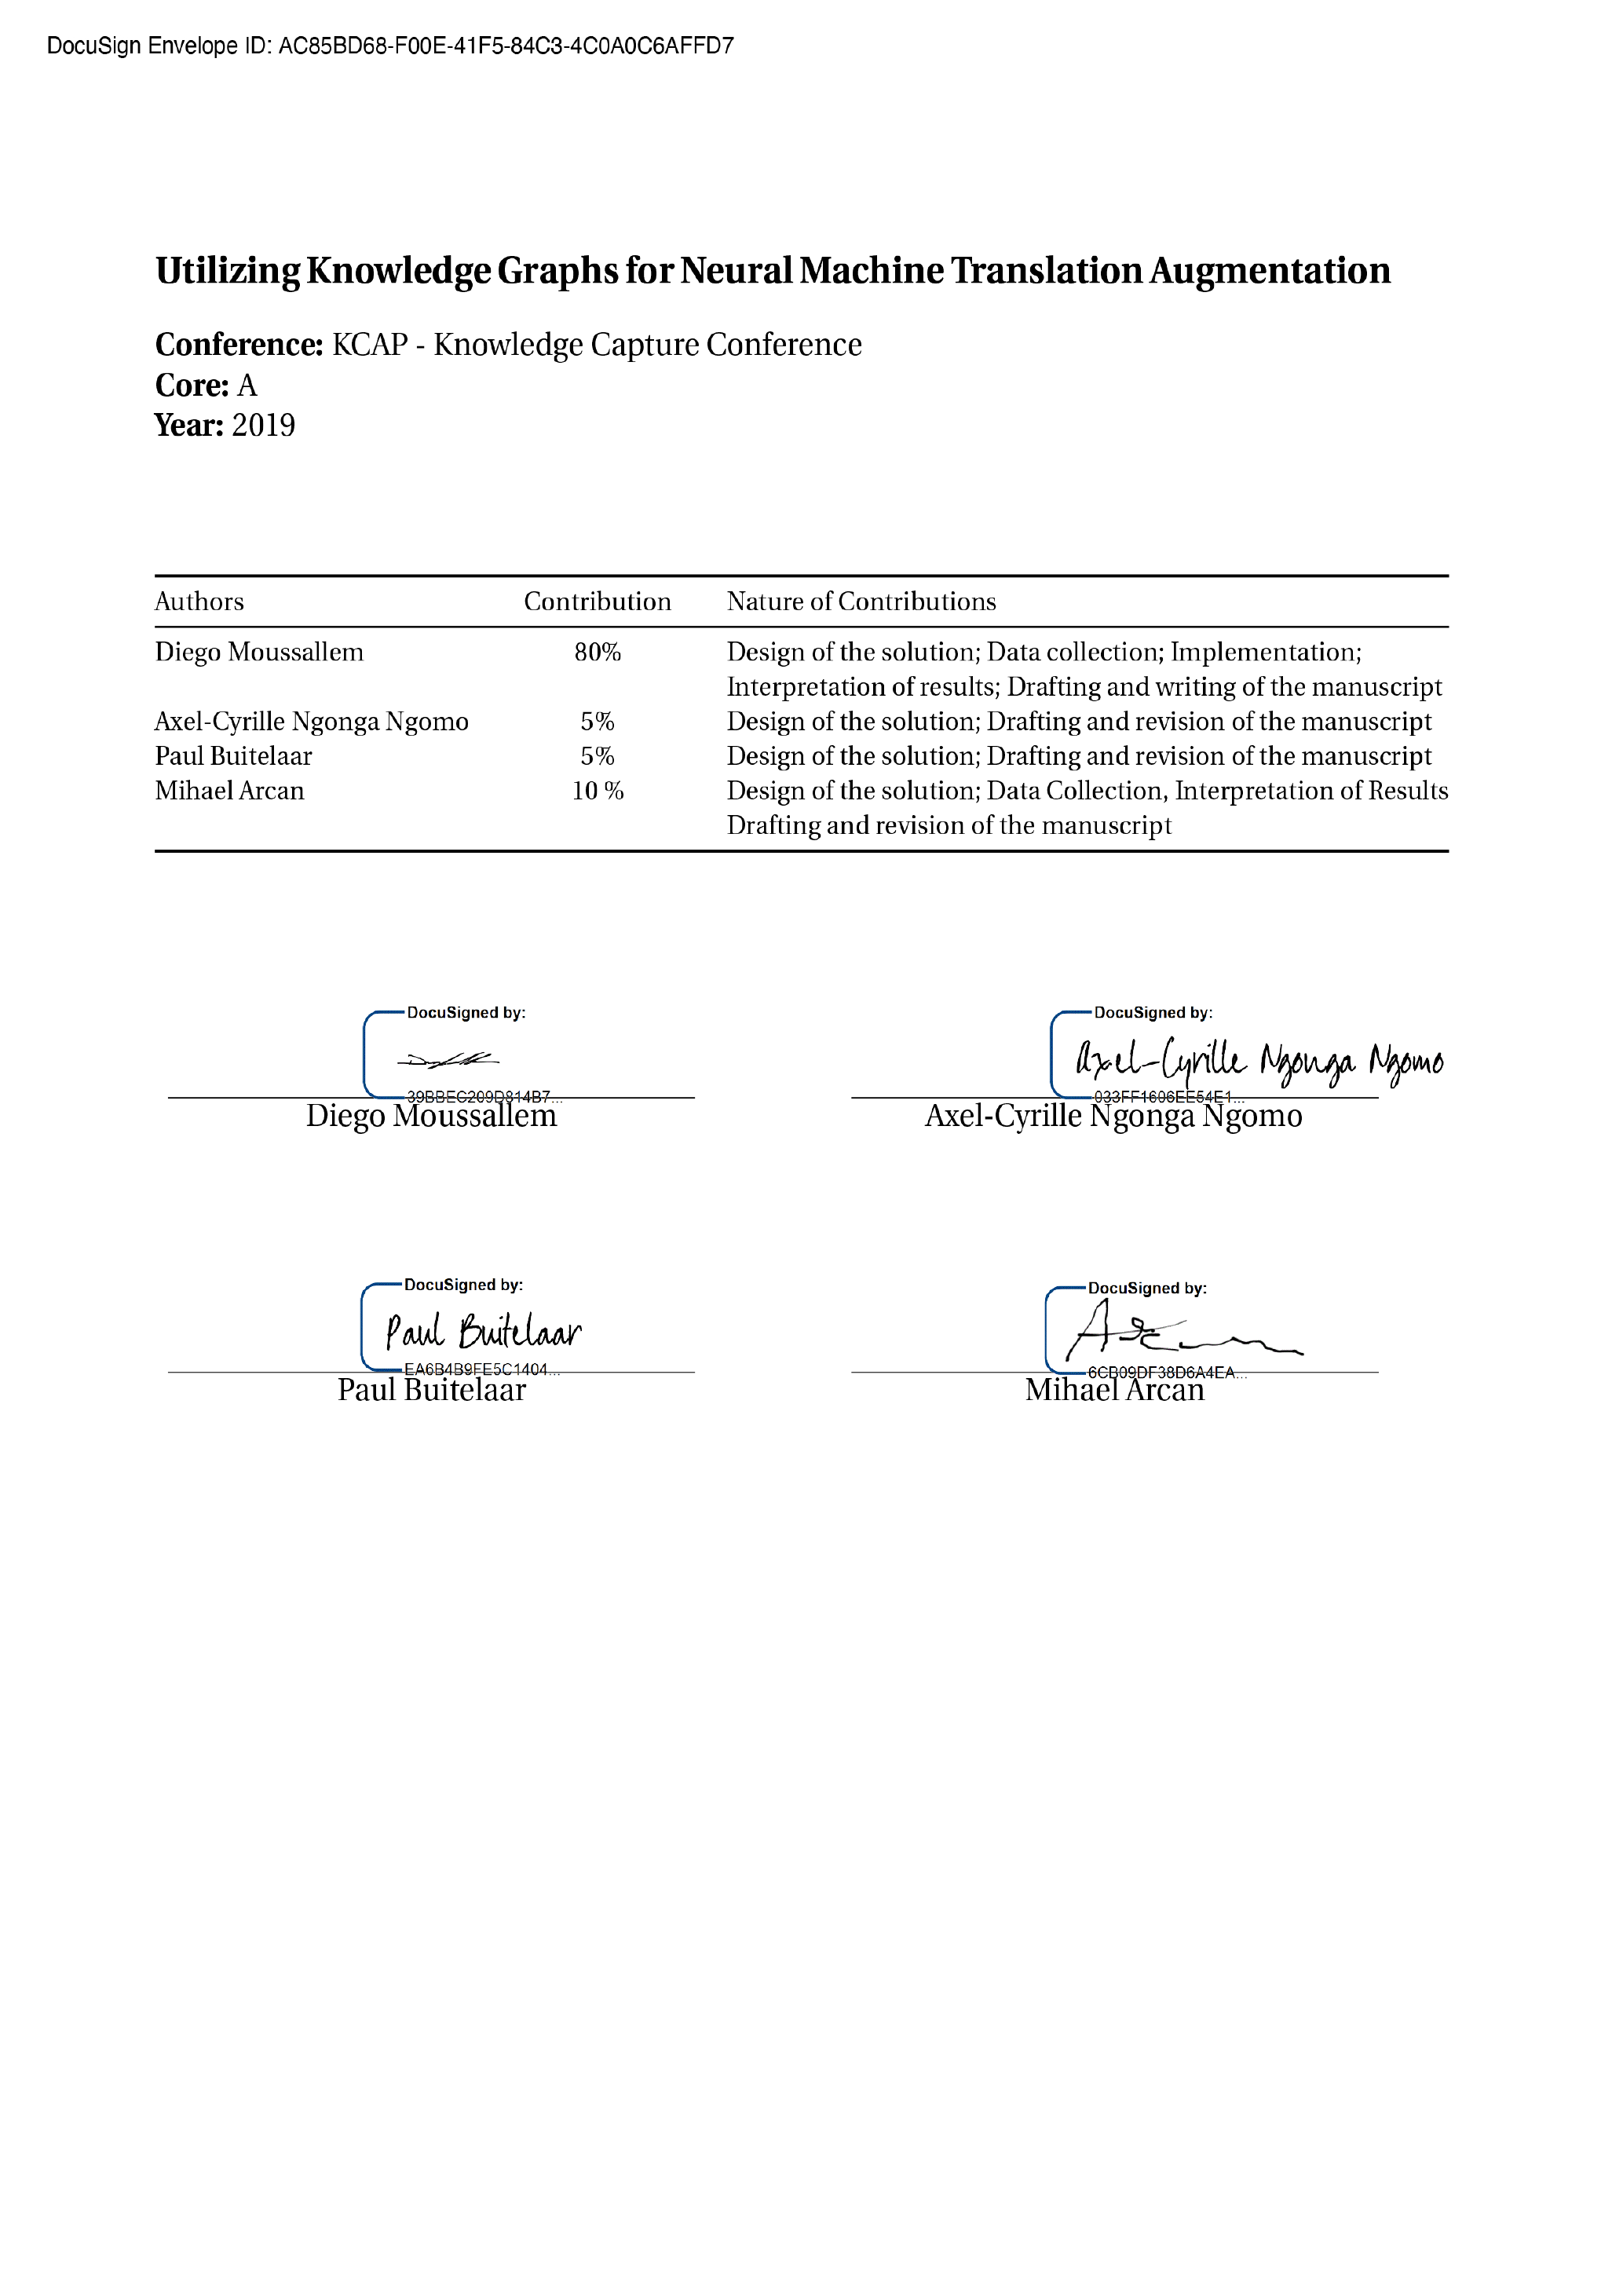}
\includepdf[pages=1,pagecommand={},trim=0mm 20mm 0mm 0mm]{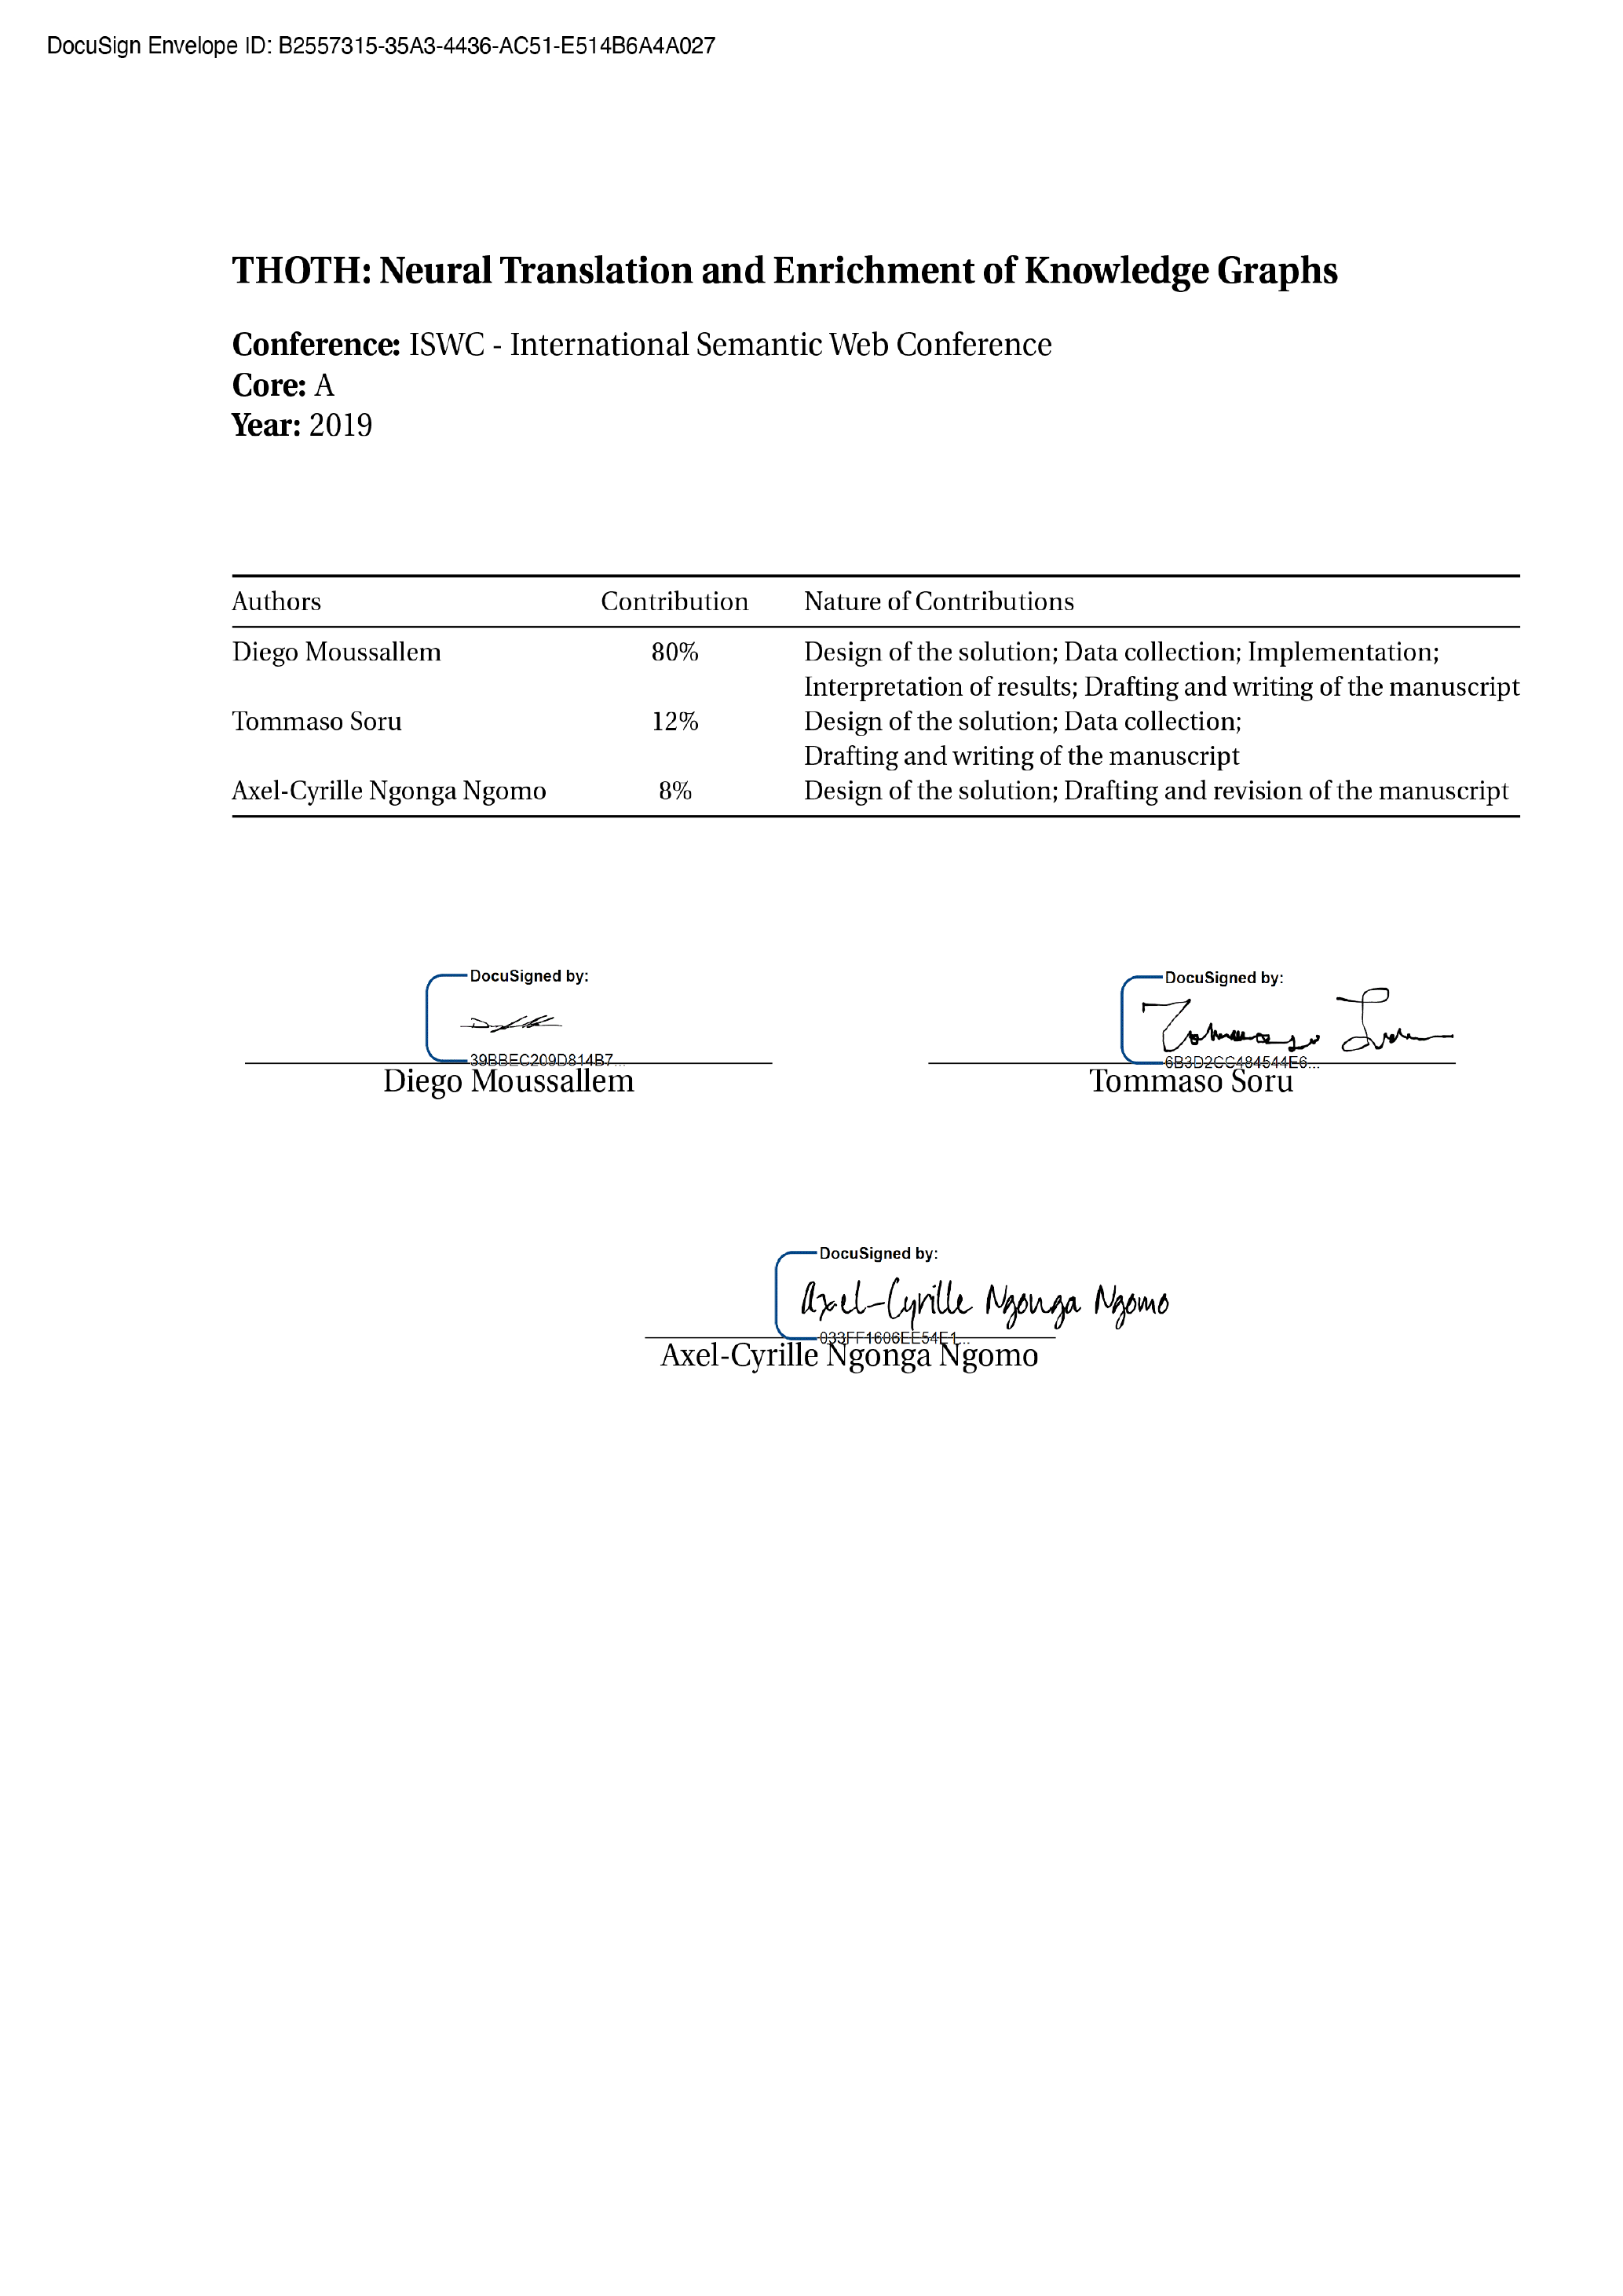}
% \section*{THOTH: Neural Translation and Enrichment of Knowledge Graphs}
% \large{\textbf{Conference:} ISWC - International Semantic Web Conference} \\
% \large{\textbf{Core:} A} \\
% \large{\textbf{Year:} 2019}
% \bigskip
% \bigskip
% \bigskip
% \begin{table*}[htb!]
% \setlength\tabcolsep{10pt}
% \small
% \centering
% %\caption{Fine-grained micro F1 evaluation.}
% \begin{tabular}{@{} lcl@{}}
% \toprule
% Authors & Contribution & Nature of Contributions\\
% \midrule
% Diego Moussallem & 80{\%} & Design of the solution; Data collection; Implementation; \\
% & & Interpretation of results; Drafting and writing of the manuscript \\
% Tommaso Soru & 12{\%} & Design of the solution; Data collection; \\
% & & Drafting and writing of the manuscript \\
% Axel-Cyrille Ngonga Ngomo & 8{\%} & Design of the solution; Drafting and revision of the manuscript \\
% \bottomrule
% \end{tabular}
% \end{table*}
% \bigskip
% \bigskip
% \bigskip
% \bigskip
% \bigskip
% \begin{center}
% 	\begin{tabular}{l p{0.1\textwidth} r}
% 		\cline{1-1} \cline{3-3}
% 		\begin{minipage}[t]{0.4\textwidth}
% 			\centering
% 				Diego Moussallem
% 		\end{minipage}
% 		&&
% 		\begin{minipage}[t]{0.4\textwidth}
% 			\centering
%                 Tommaso Soru
% 		\end{minipage}
% 	\end{tabular}
% \end{center}
% \bigskip
% \bigskip
% \bigskip
% \bigskip
% \bigskip
% \begin{center}
% 	\begin{tabular}{l p{0.1\textwidth} r}
% 		\cline{1-1}
%                 Axel-Cyrille Ngonga Ngomo
% 	\end{tabular}
% \end{center}

% \vspace*{\fill}
% \pagebreak
